# Supplementary material for: Minimal Perspective Autocalibration
Source: arXiv:2405.05605 source file (2024-05-09)
Supplement: Supplementary file 1 [file relatex.tex]

\section{Related Work}\label{SM:related}
\medskip
Surveys and summaries
\begin{itemize}
    \item[2000] Fusiello's overview~\cite{fusiello2000uncalibrated}
    \item[2003] Hartley and Zisserman~\cite{HartleyZisserman}
    \item[2023] A survey of deep learning for camera calibration~\cite{Liao-abs-2303-10559}
\end{itemize}

Varying intrinsic calibration parameters
\begin{itemize}
    \item[1999] Pollefeys - Self-Calibration and Metric Reconstruction in spite of Varying and Unknown Intrinsic Camera Parameters~\cite{PollefeysKG99} 
\end{itemize}

Constant intrinsic calibration parameteres
\begin{itemize}
    \item[1913] Kruppa - \cite{Kruppa,Gallego-abs-1801-01454}    
    \item[1992] Maybank - A theory of self-calibration of a moving camera~\cite{MaybankF92}
    \item[1992] Faugeras - Camera Self-Calibration: Theory and Experiments~\cite{FaugerasLM92}      
    \item[1995] Faugeras - Stratification of 3-D vision: projective, affine, and metric representations~\cite{Faugeras:95}
    \item[1996] Heyden - Euclidean reconstruction from constant intrinsic parameters~\cite{HeydenA96}
    \item[1996] Luong - Canonical Representations for the Geometries of Multiple Projective Views~\cite{LuongV96}
    \item[1996] Sturm - A Factorization Based Algorithm for Multi-Image Projective Structure and Motion~\cite{SturmT96}
    \item[1997] Triggs - Autocalibration and the absolute quadric~\cite{Triggs97}
    \item[1997] Luong - Self-Calibration of a Moving Camera from Point Correspondences and Fundamental Matrices~\cite{LuongF97} - uses HC on Kruppa equations - relaxes by using 5 of 6 Kruppa equations - the main competitor regarding the method, we need to compare experiments.
    \item[2000] Sturm - A case against Kruppa's equations for camera self-calibration~\cite{Sturm-2000} - singularity when the optical centers of all cameras lie on a sphere and if the optical axes pass through the sphere's center - can we solve it? If so, we beat Luong's paper from 1997.
    \item[2004] Fusiello - Globally Convergent Autocalibration Using Interval Analysis~\cite{FusielloBFB04}
    \item[2007] Chandraker - Globally Optimal Affine and Metric Upgrades in Stratified Autocalibration~\cite{ChandrakerAKB07} 
    \item[2010] Chandraker - Globally Optimal Algorithms for Stratified Autocalibration~\cite{ChandrakerAKB10}    
    \item[2010] Fusiello's local optimization~\cite{gherardi2010practical}
    \item[2018] Paudel - Sampling Algebraic Varieties for Robust Camera Autocalibration~\cite{PaudelG18}
    \item Sturm: https://imagine.enpc.fr/~monasse/Callisto/pdf/paper088.pdf
    \item Martyushev: (6pt + Abs. quadric.) https://arxiv.org/pdf/1307.3759.pdf - an overconstrained F4-like symbolic-numeric solver, returns single solution, fast but exhibits quite larger errors in s than our approach. We should compare to this too. 
\end{itemize}
