# Supplementary material for: Minimal Perspective Autocalibration
Source: arXiv:2405.05605 source file (2024-05-09)
Supplement: Supplementary file 3 [file supp.tex]

%\title{Minimal Perspective Autocalibration\\--- Supplementary Material ---}
%\maketitle
% \begin{center}
% {\Large \bf Minimal Perspective Autocalibration}\\[1ex]
% {\large \bf Supplementary Material}    
% \end{center}
\noindent In this document, we provide additional details concerning the main paper.
% {\em Andrea Porfiri Dal Cin, Timothy Duff, Luca Magri, Tomas Pajdla. Minimal Perspective Autocalibration. CVPR 2024. }

\section{Problem formulation --- additional details} \label{SM:formulation}

Although the depth equations~\eqref{eq:depth-equation-2} described in \cref{sec:depth} are the main constraints used in our approach, we wish to point out that they are by no means the only polynomial equations involving depths $\lambda_{i p},$ image points $x_{i p}$ and the calibration matrix $K$ that must be satisfied by an exact solution $((\lambda_{i p}) , K).$
In the language of~\cref{SM:sec:exp:minimal-relaxations}: the depth constraints determine the variety of problem-solution pairs $X$ \emph{locally but not globally.}

We may derive additional constraints as follows: using~\eqref{eq:zx=K[R|-RC][X;;]}, for any view pair $1\le i <j \le M$ and four distinct world points with indices $1\le p_1, \ldots , p_4\le 4$, we have
\begin{align}
\footnotesize
&\det \left(\begin{smallmatrix}
\lambda_{i p_1} x_{i p_1} -
\lambda_{i p_2} x_{i p_2} 
&
\lambda_{i p_3} x_{i p_3} -
\lambda_{i p_2} x_{i p_2} 
&
\lambda_{i p_4} x_{i p_4} -
\lambda_{i p_2} x_{i p_2} 
    \end{smallmatrix}\right) = \nonumber \\
&\det \left(\begin{smallmatrix}
\lambda_{j p_1} x_{j p_1} -
\lambda_{j p_2} x_{j p_2} 
&
\lambda_{j p_3} x_{j p_3} -
\lambda_{j p_2} x_{j p_2} 
&
\lambda_{j p_4} x_{j p_4} -
\lambda_{j p_2} x_{j p_2} 
\end{smallmatrix}\right).\label{eq:oriented-tetrahedra}
    \end{align}
This follows from our assumption that $K$, and hence also $\det (K)$, is constant: compare with~\eqref{eq:recover-rotation} below.
    
It is important to remember that, when solving with a minimal relaxation, the equations that are not enforced may or may not continue to hold for noisy data.
As an example of this, we may consider the unique class of minimal problems in~\Cref{tab:Minimal-Autocalibration-Substitution-Tab} for the scenario $\mathtt{11000}$ with $M=3$ fully calibrated views.
As illustrated in \cref{SM:fig:scranton-relax}, we may drop exactly one depth equation for the view pair $(i,j) = (1,2)$ to obtain a representative for the equivalence class of minimal relaxations.
This relaxation has the effect that~\eqref{eq:oriented-tetrahedra} no longer must hold for this view pair.
Indeed, we find that this equation is typically violated in the case of noisy data and for all $639$ non-synthetic solutions when solving a generic synthetic problem instance.
On the other hand, for the view pair $(i,j) = (1,3)$, the equation~\eqref{eq:oriented-tetrahedra} holds even for non-synthetic solutions or noisy data.

We may rephrase the observations of the previous paragraph in the geometric language developed in~\cref{sec:relax-enumerate-solve} (see also SM~\ref{SM:relaxation} below.)
From this point of view,~\eqref{eq:oriented-tetrahedra} is valid for both view pairs on the incidence variety $X$ associated with the overconstrained problem but only generally valid for the view pair $(1,3)$ on the incidence variety $\VV (\bg )$ associated to the minimal relaxation.
The local nature of parameter homotopy ensures, for this problem, that we do not need to explicitly enforce the constraint~\eqref{eq:oriented-tetrahedra} for one view pair.
However, any attempt to simultaneously enforce these constraints for both view pairs and the chosen depth constraints will invariably lead us back to an overconstrained problem.

\begin{figure}[b]
\centering
\includegraphics[width=0.25\textwidth]{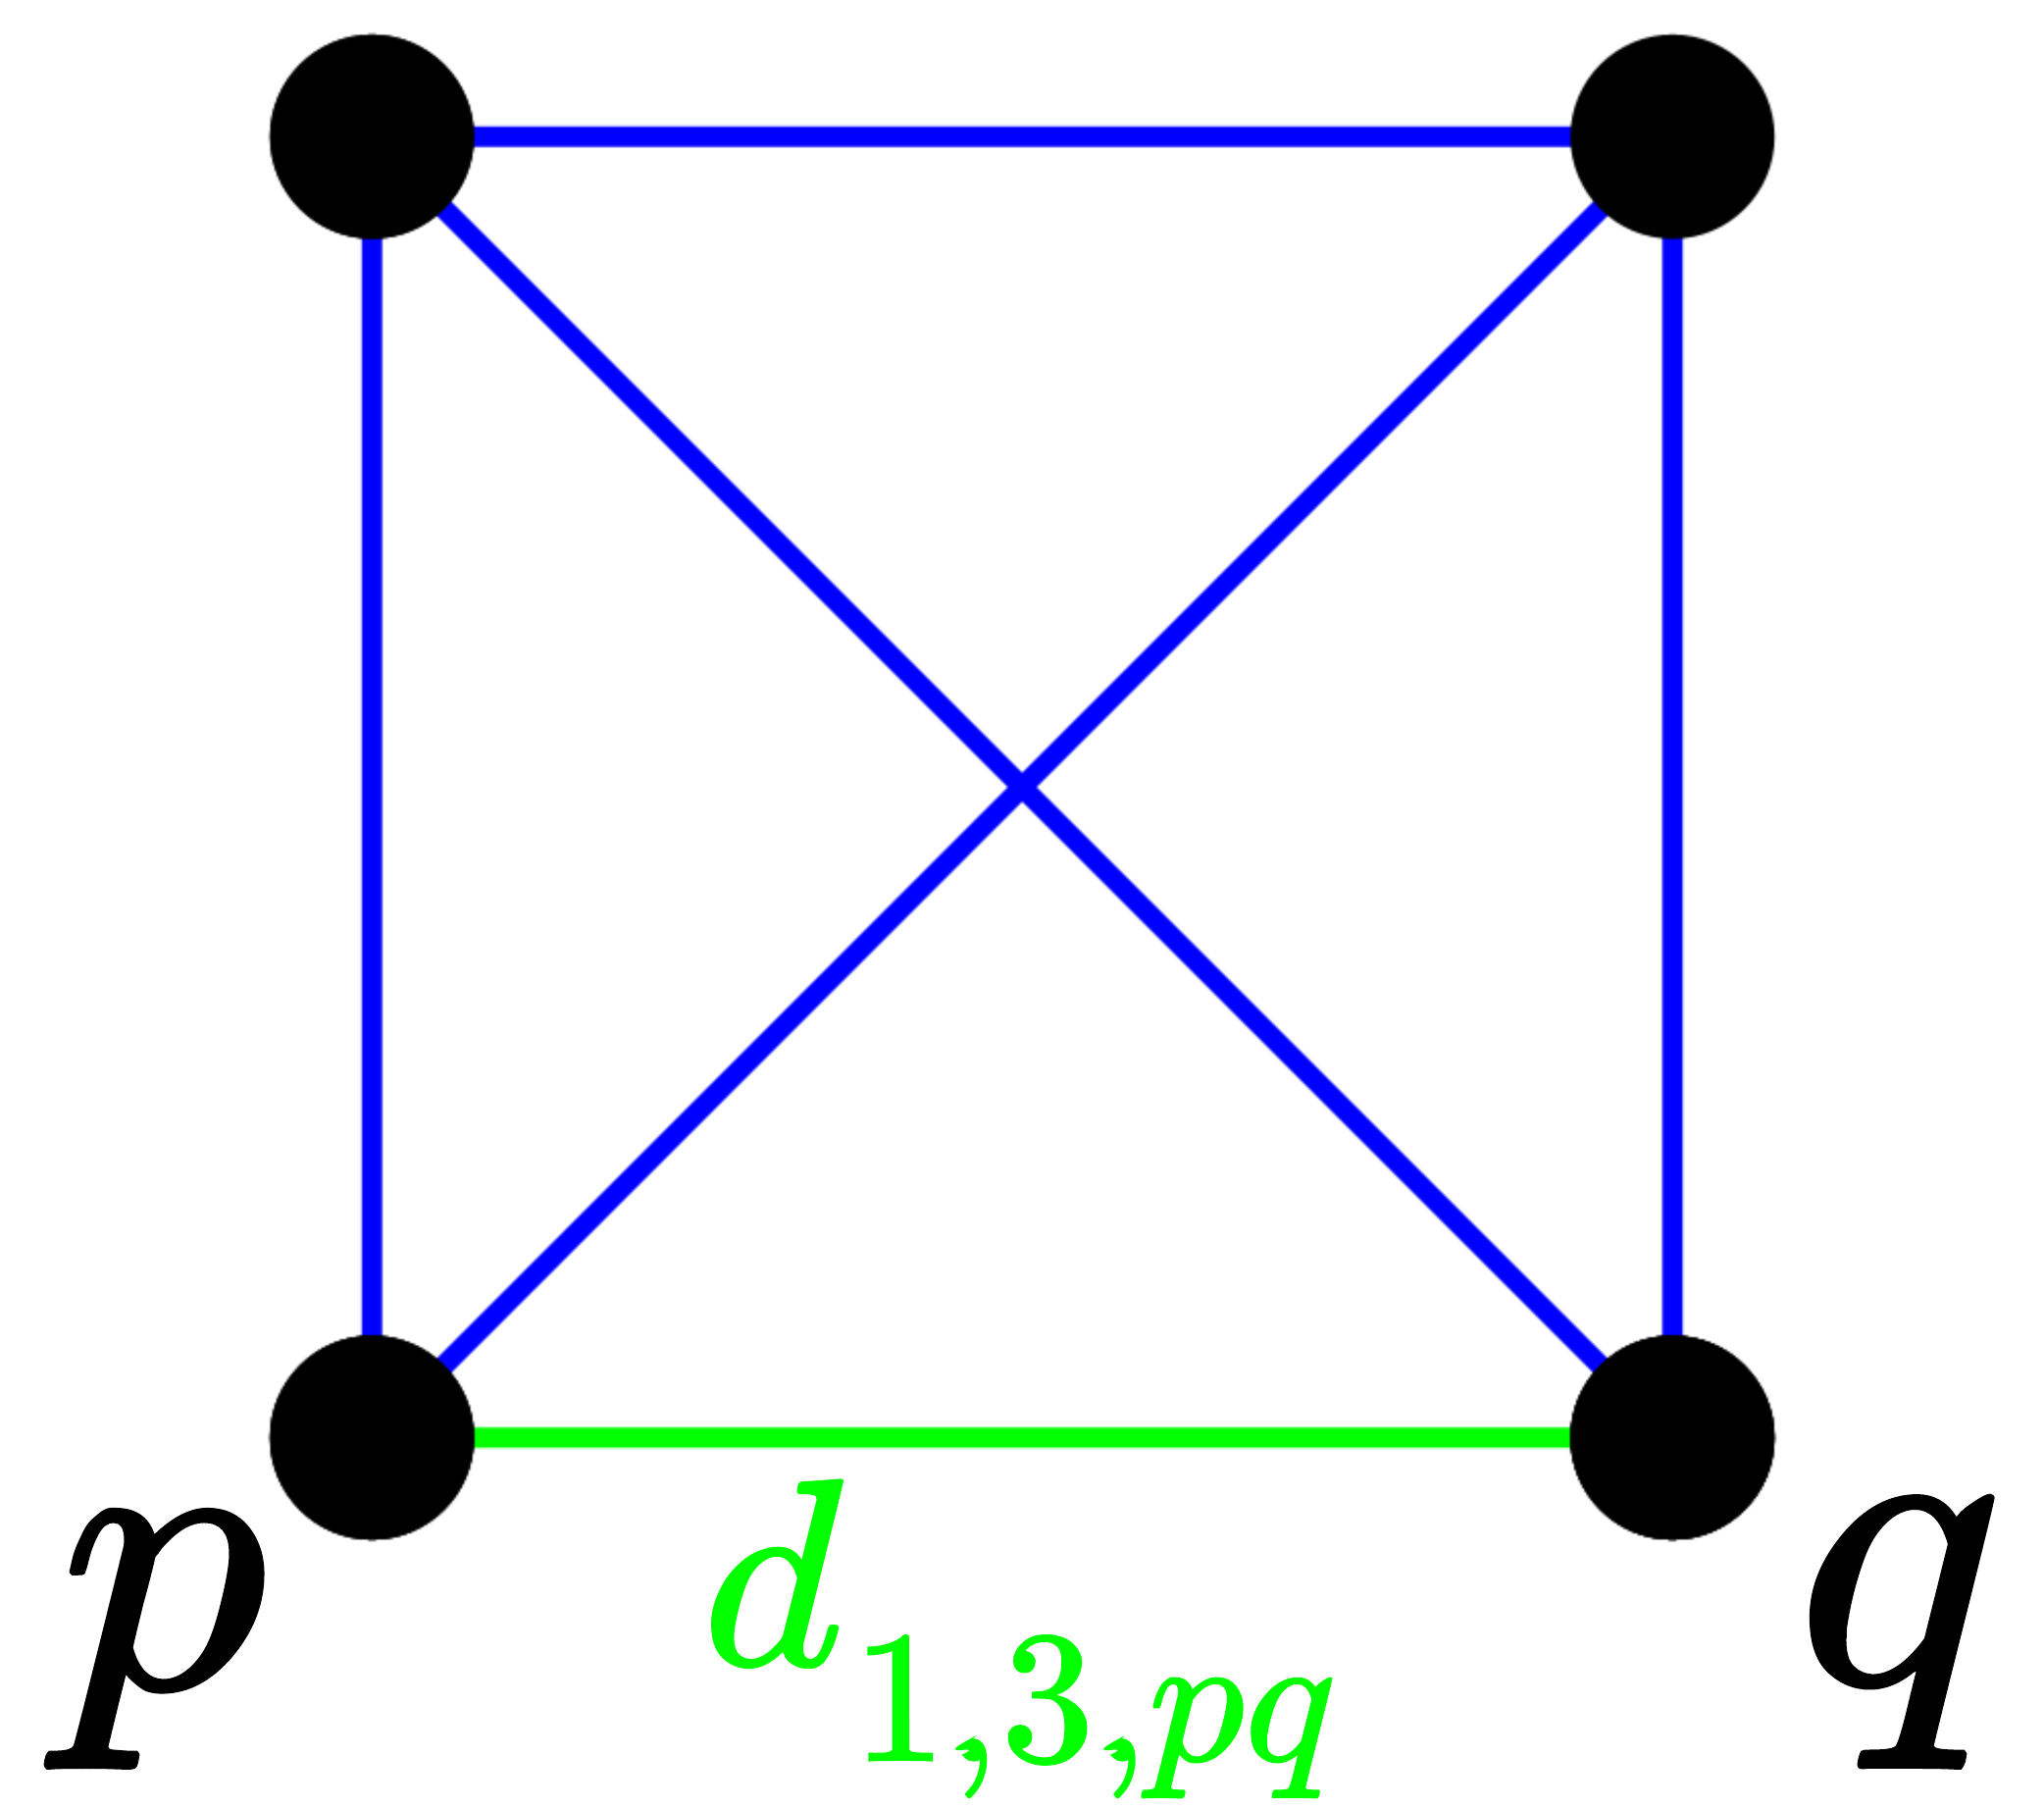}
\caption{Visualization of a representative of the equivalence class of minimal relaxations for the $\mathtt{11000}$ problem obtained by dropping a constraint $d_{1,2,pq}$ for view pair $(1,2)$.}
\label{SM:fig:scranton-relax}
\end{figure}

\input{supp/supp-tab-autocalibration}

\section{Normalization of known intrinsics}\label{SM:normalization}
Referring to \cref{sec:specification}, we provide details on transforming image coordinates to normalize the value of known intrinsic parameters. Without loss of generality, for $R_i = I_3$ and $C_i = 0$, \cref{eq:zx=K[R|-RC][X;;]} writes
\begin{equation}
\small
\lambda_{ip}\,x_{ip} = \mat{c}{K \mid 0}\mat{c}{X_p\\1},\ i \in [M],\ p \in [N] \; .
\end{equation}
If $X_p = \left( \alpha \;\; \beta \;\; \gamma \right)^\top$, then $\lambda_{ip} = \gamma$, and
\begin{equation} \label{SM:eq:image-coords}
\small
x_{ip} = \mat{c}{x_{ip,1} \\ x_{ip,2} \\ 1} = \mat{c}{f a + s b + u \\ g b + v \\ 1} ,\ a = \frac{\alpha}{\gamma}, \; b = \frac{\beta}{\gamma} \; .
\end{equation}

Additionally, we present the well-known decomposition of $K$ into scaling, shear, and translation transformations applied to normalized image coordinates, which we will reference in later sections:
\begin{equation} \label{SM:eq:decomp-k}
    K = \underbrace{\mat{ccc}{1 & 0 & u \\ 0 & 1 & v \\ 0 & 0 & 1}}_\mathrm{Translation} \underbrace{\mat{ccc}{1 & s/g & 0 \\ 0 & 1 & 0 \\ 0 & 0 & 1}}_\mathrm{Shear} \underbrace{\mat{ccc}{f & 0 & 0 \\ 0 & g & 0 \\ 0 & 0 & 1}}_\mathrm{Scaling}.
\end{equation}

\subsection{Known Focal Lengths}
Normalization of known focal lengths involves reversing the scaling transformation in~\eqref{SM:eq:decomp-k} along the x and/or y axes. When $f$ is known, $x_{ip}$ may be transformed into normalized coordinates $\tilde{x}_{i p}$ in which $f=1$, %to its standard one $f = 1$ by substituting $\tilde{s}$ and $\tilde{u}$ into \eqref{SM:eq:image-coords}:
\begin{equation}
    \tilde{x}_{ip} = \mat{c}{a + \tilde{s} b + \tilde{u} \\ g b + v \\ 1} ,\ \tilde{s} = \frac{s}{f}, \; \tilde{u} = \frac{u}{f} \; .
\end{equation}
Then, we may solve for the unknown transformed intrinsics $(g, \tilde{u}, v, \tilde{s})$ and recover the original values of $u, s$ using the known value of $f$. Similarly, when $g$ is known, we use%~\eqref{SM:eq:image-coords}:
\begin{equation}
    \tilde{x}_{ip} = \mat{c}{f a + s b + u \\ b + \tilde{v} \\ 1} ,\ \tilde{v} = \frac{v}{g} \; ,
\end{equation}
we solve for the unknown transformed intrinsics $(f, u, \tilde{v}, s)$, and recover the original value of $v$.

\subsection{Known Principal Point} \label{SM:sec:norm-pp}
Normalizing known principal point coordinates involves reversing the translation transformation in~\eqref{SM:eq:decomp-k} to center image coordinates at the origin.

When $u$ is known, normalizing the known value of $u$ to $u = 0$ involves subtracting $u$ from $x_{ip,1}$, the first coordinate of $x_{ip}$. Notably, no additional substitution of other intrinsic parameters is necessary. Similarly, when $v$ is known, normalizing the known value of $v$ to $v = 0$ may be achieved by subtracting $v$ from the second coordinate $x_{ip,2}$. 

\subsection{Known Skew}
Knowing the camera skew, when it is nonzero, implies knowledge of the shear transformation embedded in $K$, and that is applied to the normalized image coordinates.

The shear transformation in \eqref{SM:eq:decomp-k} is determined by $s^\star = \frac{s}{g}$. Thus, when $s^\star$ is known, the skew-induced shear in image coordinates may be removed by transforming $x_{ip,1}$, the first coordinate of $x_{ip}$, as follows:
\begin{equation} \label{SM:eq:skew-norm}
    \tilde{x}_{ip,1} = x_{ip,1} - s^\star x_{ip,2} \; .
\end{equation}
Importantly, \eqref{SM:eq:skew-norm} successfully reverses the shear transformation when either $v = 0$ or when $v$ is known and $x_{ip}$ is first normalized to fix $v = 0$, as detailed in \cref{SM:sec:norm-pp}. This can be observed by rewriting $x_{ip}$ from \eqref{SM:eq:image-coords} as follows:
\begin{equation}
\small
\tilde{x}_{ip} = \mat{c}{\tilde{x}_{ip,1} \\ \tilde{x}_{ip,2} \\ 1} = \mat{c}{f a + s^\star x_{ip,2} + u - s^\star v \\ g b + v \\ 1} ,\
\end{equation}
by substituting $b = (x_{ip,2} - v)/g$.
Notably, no additional substitution of other intrinsic parameters is necessary.
% \tim{Say that this is the generic case for $s^\star $ is fixed.}

Our previous autocalibration specification can be extended to minimal problems in the notable case where a \emph{generic} $s^\star$ is known and nonzero, but $v$ is unknown. Referring to \ref{sec:depth}, $s^\star$ appears explicitly in our parametrization of $\omega$, as defined in \eqref{eq:omega}. Thus, referring to \cref{sec:solving-hc}, given any system $\mathbf{g}(\mathbf{p}, \mathbf{x}) = 0$ encoding a minimal relaxation of an autocalibration problem in which $s^\star$ is known and nonzero and $v$ is unknown, we may treat $s^\star \in \mathbf{p}$, as a parameter of the system. Then, we may construct minimal solvers using a standard online/offline parameter homotopy approach such as described in~\Cref{sec:solving-hc}. Referring to \cref{sec:specification}, we indicate known nonzero $s^\star$ in the 5-tuple of unknowns $\mathtt{fguvs}$ by setting $s = s^\star$. This notation is used in \cref{SM:tab:norm-skew-minimal} to report the solution count in $\mathbb{C}$ computed during the offline stage for all cases where $s^\star$ is known and nonzero and $v$ is unknown, mirroring the comprehensive approach taken in \cref{tab:Minimal-Autocalibration-Substitution-Tab}.

% In the offline stage, the synthetic solution $(\mathbf{p}_0, \mathbf{x}_0)$ is parametrized not just by the image points $x_{ip}$ but has an additional parameter $s^\star \in \mathbf{p}_0$. Similarly to what has been done in \cref{tab:Minimal-Autocalibration-Substitution-Tab}, we report the minimum solution count for these minimal problems, when $s^\star$ is known. We indicate knowledge of $s^\star$ in the 5-tuple of unknowns $\mathtt{fguvs}$ by setting $s = s^\star$.

\input{supp/supp-tab-skew}

\section{Depth equations without symmetry removal} \label{SM:taxonomy-no-sub}
We discuss the effect of substituting \eqref{eq:omega} into $d_{i,j,pq}$ on the solution count in $\mathbb{C}$ for the 80 interesting minimal autocalibration problems presented in \cref{tab:Minimal-Autocalibration-Substitution-Tab}.

Without substituting \eqref{eq:omega}, $d_{i,j,pq}(\lambda, K; x)$ writes:
\begin{align} \label{SM:eq:depth-equation}
\small
d_{i,j,pq} (\lambda , K ; x) := & (K^{-1} \lambda_{ip} x_{ip} - K^{-1} \lambda_{iq} x_{iq})^T \nonumber \\ 
& (K^{-1} \lambda_{ip} x_{ip} - K^{-1} \lambda_{iq} x_{iq}) \nonumber \\
- & (K^{-1} \lambda_{jp} x_{jp} - K^{-1} \lambda_{jq} x_{jq})^T \nonumber \\
& (K^{-1} \lambda_{jp} x_{jp} - K^{-1} \lambda_{jq} x_{jq}),
\end{align}
and we may write our main constraint as
\begin{equation}
\label{SM:eq:depth-equation-2}
    d_{i,j,pq}(\lambda, K; x) = 0 \; .
\end{equation}

In \cref{SM:Tab:minimal-autocalibration}, we list the same 80 interesting groups of problems indexed by $(\mathtt{fguvs},M,N)$, mirroring \cref{tab:Minimal-Autocalibration-Substitution-Tab} in the main paper. Notably, we report the minimum and maximum solution count in $\mathbb{C}$, referring to the unknown depths and the parameters of $K$ in \eqref{eq:zx=K[R|-RC][X;;]}-\eqref{SM:eq:depth-equation}.

\section{Details on minimal relaxations}\label{SM:relaxation}
To illustrate some technicalities in our definition of minimal relaxation, we consider again the irreducible variety
$$
X = \{ (p_1, p_2, x) \in \CC^3 \mid x^2 - p_1 = p_2 x^2 -1 = 0 \}
$$
depicted in~\Cref{fig:minimal-relaxation} of the main paper.
The real-valued points of $X$ in $\mathbb{R}^3$ form the purple space curve where the red and blue surfaces intersect below.
\begin{center}
\includegraphics[width=0.25\textwidth]{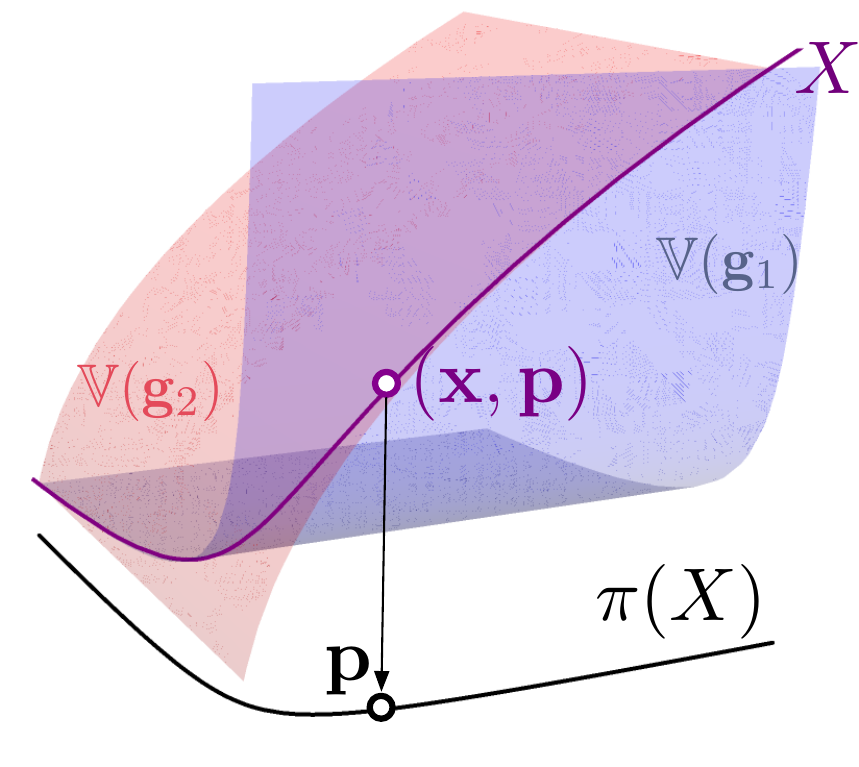}
\end{center}
In this example, we understand the vector $(p_1, p_2) \in \CC^2$ to represent a problem instance and $x\in \CC$ one of its solutions.
The set of exactly solvable problems is the image of the projection map $\pi : X \to \CC^2$, namely the hyperbola $p_1p_2=1$ drawn in black.
Then, the problem is overconstrained since a generic problem instance will not lie on the hyperbola and will have no solutions.
This manifests in the failure of the rank conditions~\eqref{eq:rank-conditions}
: for a generic problem-solution pair $(p_1,p_2,x)\in X$, we have
$$
\small
\operatorname{rank} 
\begin{pmatrix}
-1 & 0 & 2x\\
0 & x^2 & -2p_2 x
\end{pmatrix}
\ne 1
\quad
\forall \, (p_1, p_2, x) \in X \setminus \{ (0,0,0) \}.
$$
Two minimal relaxations can be obtained by dropping one of the two equations defining $X$. 
These relaxations correspond to the surfaces $X_1 = X_{x^2 -p_1}$ and $X_2 = X_{p_2 x^2 -1},$ drawn above in red and blue, respectively.
The union of these two surfaces is \emph{not} a minimal relaxation, since the Jacobian of $(x^2-p_1)(p_2x^2-1)$ vanishes identically along $X.$
For the rational function $\bg (p_1, p_2, x) = 1/x^2 - p_2,$ note that we also have $\VV (\bg ) = X_{\bg} = X_2.$
If we instead consider $\bg ' = (p_2 x^2 - 1) x,$ the variety $\VV (\bg ') $ has two irreducible components, given by $\VV (x)$ and the minimal relaxation $X_{\bg '} = X_{\bg} = X_1$.
Finally, let us observe that in this example, the degrees of the minimal relaxations $X_i \to \CC^2$ are both $2.$
This need not be the case in general: if we consider instead of $X$ the space curve $\VV (x^2 - p_1, x^3 - p_3)$, we see there are minimal relaxations of degree 2 or 3.
This example also shows that relaxations can increase the number of solutions, even for an exactly solvable problem instance.

\medskip
\noindent 
We wish to point out that our notion of a minimal relaxation occurs implicitly in previous works~\cite{kileel-trifocal,DBLP:conf/eccv/DuffKLP20} studying constraints involving calibrated trifocal tensors and point-line minimal problems with partial visibility.
Both works consider a minimal relaxation of the overconstrained problem of estimating four points in three calibrated views. In this minimal relaxation, one point in one view is replaced by a line.
Both of these works formulate the overconstrained problem of estimating four points in three calibrated views and consider the ``Scranton" relaxation of this problem in which only a single point-point-line constraint on the trifocal tensor is enforced for one of the point triplets.
This problem has $272$ solutions.
As observed in~\cite{DBLP:conf/cvpr/HrubyDLP22},
Scranton can also be formulated in terms of depths and an extra slack variable.
The depth-formulated Scranton is \emph{not} a minimal relaxation in the sense defined above.
In this work, instead of adding variables, we drop equations.
We may simply drop the equation $d_{1,2,12} (\lambda, \omega; x)=0 $ in the fully calibrated case. 
This gives a minimal relaxation with $640 = 2 \times 320$ solutions and a two-way symmetry that sends $\lambda_{2, p} \to -\lambda_{2,p}$ and fixes all other variables.
We remark that a further systematic study of symmetries appearing in our zoo of autocalibration problems, along the lines conducted in~\cite{DBLP:journals/corr/Duff-Korotynskiy-22}, would be very interesting.
However, this study lies beyond the scope of this investigation.

HC methods for solving Kruppa's equations may also be understood in our framework of minimal relaxations.
For Kruppa, solutions $\xx $ are the entries of $3\times 3$ matrix representing the DIAC, and triples of fundamental matrices specify parameters $\pp$. Moreover, for a synthetic problem-solution pair $(\pp_0, \xx_0)\in X$ used to initialize monodromy, certain compatability conditions on fundamental matrices encoded in $\pp_0$ must be satisfied~\cite[\S 15.4]{HartleyZisserman}.

\input{supp/relaxations/figure}

\section{Enumerating minimal problems ---\\additional details}\label{SM:enumeration}

Returning to the enumeration problem described in in~\Cref{sec:relax-enumerate-solve}, we now discuss \emph{line graphs}, a standard graph-theoretic construction.
The utility of this construction is that the isomorphism class of a $4$-coloring is completely determined by an associated line graph $\LL(c)$ after equipping it with a suitable vertex labeling. 
The vertices of the line graph $\LL(c)$ are simply the non-white edges, and an edge between two vertices of $\LL(c)$ exists whenever the two non-white edges share a vertex between $1$ and $N$.
We label each vertex $pq \in \LL(c)$ by its color $c(pq).$ 
Two isomorphic graphs have isomorphic line graphs; conversely, a classical theorem of Whitney~\cite{whitney1992congruent} implies that two connected graphs whose line graphs are isomorphic are themselves isomorphic, with the sole exception of the complete graph $K_3$ and the claw graph $K_{1,3}$ (see eg.~\cite[Theorem 8.3]{harary}.)
Although  $\LL(K_3) \cong \LL(K_{1,3})$, the original graphs $K_3$ and $K_{1,3}$ have different numbers of edges. 
From this, it easily follows that we can decide whether or not two $4$-colorings $c_1,c_2$ are isomorphic: form the two graphs $\LL(c_1)$ and $\LL(c_2)$, decide if there exists an isomorphism that respects their labelings, and repeat this same procedure for the two graphs $\LL(c_1), \LL(c_2 \circ \tau),$ where $\tau $ swaps green and red edges.

We implement software based on the \emph{NetworkX} library \cite{networkx}, and the VF2++ algorithm \cite{juttner2018vf2++} to compute the isomorphism classes for all minimal problems listed in \cref{tab:Minimal-Autocalibration-Substitution-Tab}. The code is implemented in Python and is publicly available at {\small \href{https://github.com/andreadalcin/MinimalPerspectiveAutocalibration}{github.com/andreadalcin/MinimalPerspectiveAutocalibration}}.

\cref{SM:tab:isomorphism-viz} provides a visualization of one representative 4-coloring for each isomorphism class for the $\mathtt{fguv0}, \mathtt{fgu00}, \mathtt{fg000}$ minimal problems in $M = 3$ views. The isomorphism classes for $\mathtt{fguvs}$ are too many to be visualized in \cref{SM:tab:isomorphism-viz}. Still, as part of our software, we provide a visualization tool and instruction to visualize equivalence classes for $\mathtt{fguvs}$.

\input{supp/supp-tab-graphs}

\section{Experiments} \label{SM:experiments}
We provide additional details on our experimental validation that were omitted from the main paper due to space restrictions.

\subsection{Choice of Minimal Relaxations} \label{SM:sec:exp:minimal-relaxations}
In case of different minimal relaxations yielding the same minimum solution count, e.g., in $\mathtt{fguv0}$, we selected that yielding the lowest mean reprojection error in our synthetic test described in Sec.~\ref{sec:experiments-synthetic}. We noted that reprojection error fluctuations among different relaxations with identical solution counts are always below 1\%, suggesting comparable numerical performance between different minimal relaxations with the same solution count.

For the purposes of this work, we list the specific minimal relaxations used to implement the solvers $\mathtt{ffuv0}$, $\mathtt{fguv0}$, and $\mathtt{fguvs}$, which are used throughout our experiments. Specifically, for each implemented solver, we specify the depth constraints that are omitted from the chosen system of equations $\mathbf{g}$:

\begin{itemize}
\item $\mathtt{ffuv0}$: $d_{1,2,45}$, $d_{1,3,45}$, $d_{1,2,35}$ (see~Fig.~\ref{SM:fig:relaxation:ffuv0}).
\item $\mathtt{fguv0}$: $d_{1,2,45}$, $d_{1,3,45}$ (see~Fig.~\ref{SM:fig:relaxation:fguv0}).
\item $\mathtt{fguvs}$: 
$d_{1,2,56}$, 
$d_{1,3,56}$,
$d_{1,2,45}$, 
$d_{1,3,45}$,
$d_{1,2,46}$,
$d_{1,2,36}$,
$d_{1,2,26}$,
$d_{1,3,34}$ (see~Fig.~\ref{SM:fig:relaxation:fguvs}).
\end{itemize}

\medskip
Our public code also includes starting the parameters and solutions for parameter homotopies used by each solver to ensure full reproducibility.

\subsection{Computing Camera Rotations and Centers from Projective Depths} \label{SM:sec:exp:depth2rot}
We discuss the conversion of projective depths into camera rotations and centers. Referring to \cref{sec:experiments}, our autocalibration formulation allows us to perform an Euclidean reconstruction. However, we obtain the projective depths associated with image points rather than camera roto-translations and 3D point coordinates. However, recovering camera rotations and centers is straightforward, assuming that, without loss of generality, the $i = 1$ camera is at $R_1 = I$ and $C_1 = 0$.

Initially, we compute 3D points, denoted as $X_{ip}$, for each camera $i \in [M]$, using $X_{ip} = \lambda_{ip} K^{-1} x_{ip}$. Throughout this section, we express $X_{ip}$ in Cartesian coordinates, \emph{i.e.}, $X_{ip} \in \mathbb{R}^3$. Centering all 3D points by subtracting $X_{11}$ (the point $p=1$ seen by the $i=1$ camera), we extract translation components $t_{i} = X_{i1}$ for $i \in [2, \ldots, M]$. Subtracting the translation component from the 3D points seen by the $i$-th view ($\tilde{X}_{ip} = X_{ip} - t_{i}$), we compute the rotation component
\begin{equation}\label{eq:recover-rotation}
    R_i = \mat{ccc}{\tilde{X}_{i2} & \tilde{X}_{i3} & \tilde{X}_{i4}} \mat{ccc}{\tilde{X}_{12} & \tilde{X}_{13} & \tilde{X}_{14}}^{-1} \; .
\end{equation}
Finally, we compute the camera centers
\begin{equation}
    C_i = \lambda_{i2} K^{-1} x_{i2} - R_i \lambda_{12} K^{-1} x_{12} \, , \quad i \in [2, \ldots, M] \; .
\end{equation}

As discussed in \cref{SM:formulation}, a given relaxation might remove constraints that enforce the validity of the recovered rotation matrices, \emph{i.e.}, $R_i \in \mathrm{SO}(3)$. If $R_i$ is not an orthogonal matrix, we compute an SVD $R_i = U S V^\top$ and the closest orthogonal matrix $\tilde{R}_i = U V^\top$ (with respect to either the Frobenius or spectral norm.)

This approach is consistently applied in our experimental validation, and we provide Julia code for the conversion from projective depth to camera roto-translation.

\begin{figure*}[t]
    \centering
    \includegraphics[width=\textwidth]{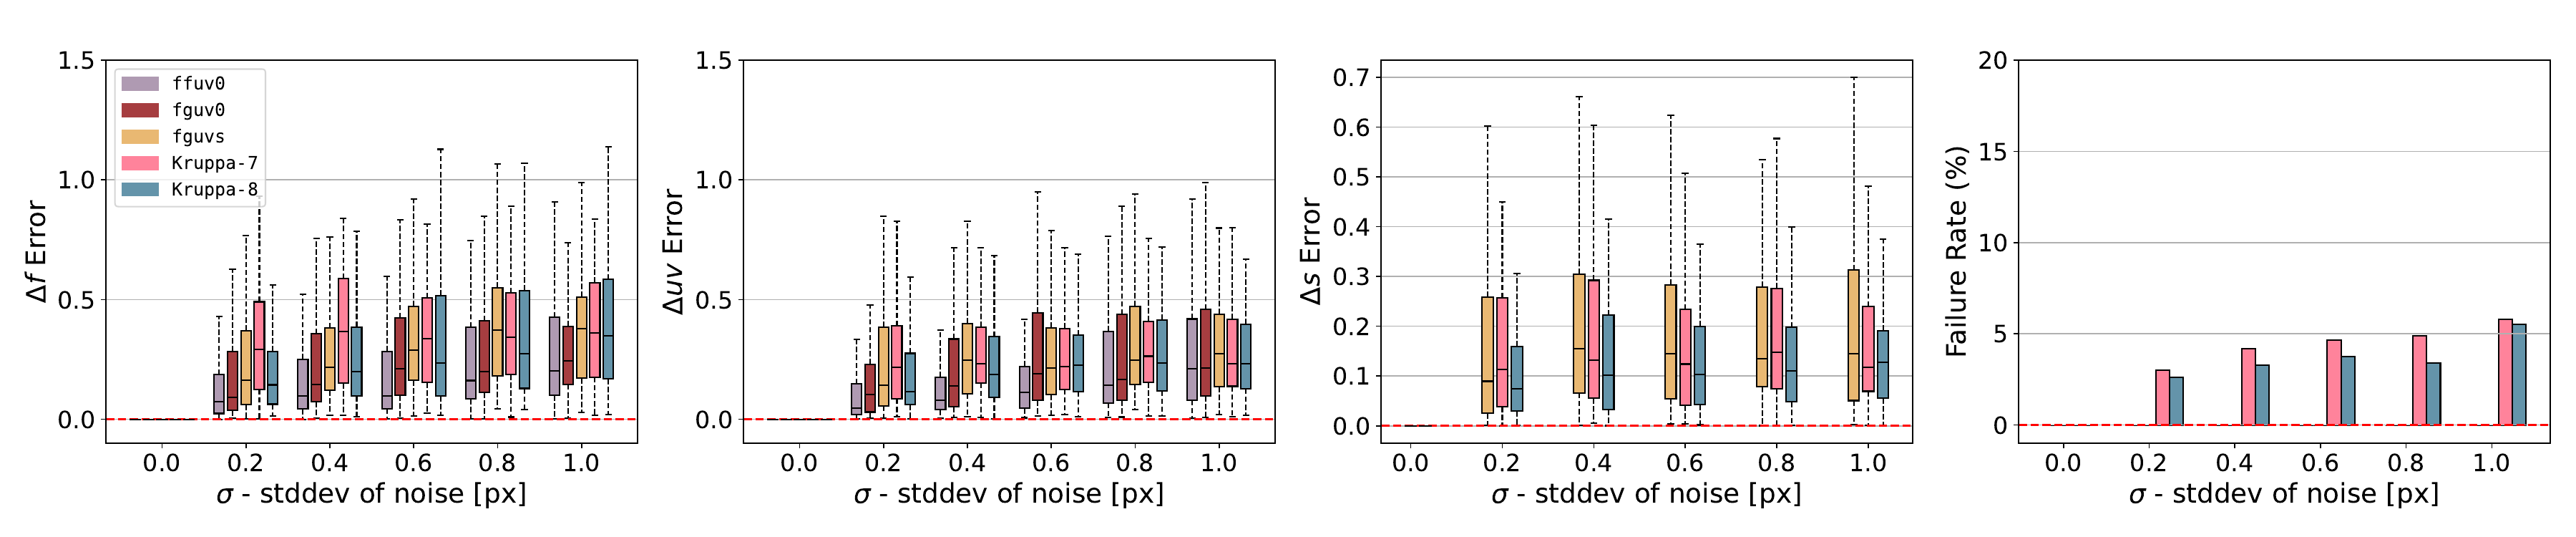}
    \caption{\textbf{Kruppa-7 Evaluation on Synthetic Images.} Solver accuracy is assessed under varying levels of zero-mean Gaussian noise (denoted by $\sigma$ on the x-axis) applied to pixel coordinates. Mean reprojection error and relative errors in focal lengths $\Delta fg$, principal point $\Delta uv$, and skew $\Delta s$ are reported. For error measures, boxes represent the interquartile range of error distribution. The right-most plot illustrates the failure rate as a percentage, with \TT{fguv0}, \TT{ffuvs}, and \TT{fguvs} excluded due to no failures. Results are averaged for 1000 synthetic image sequences. Synthetic camera parameters are set to mirror the configuration described in \cref{sec:experiments-synthetic}. Results are averaged over 1000 synthetic image sequences.
    }
    \label{SM:fig:experiments-synthetic}
\end{figure*}


\begin{figure*}
    \centering
    \includegraphics[width=\textwidth]{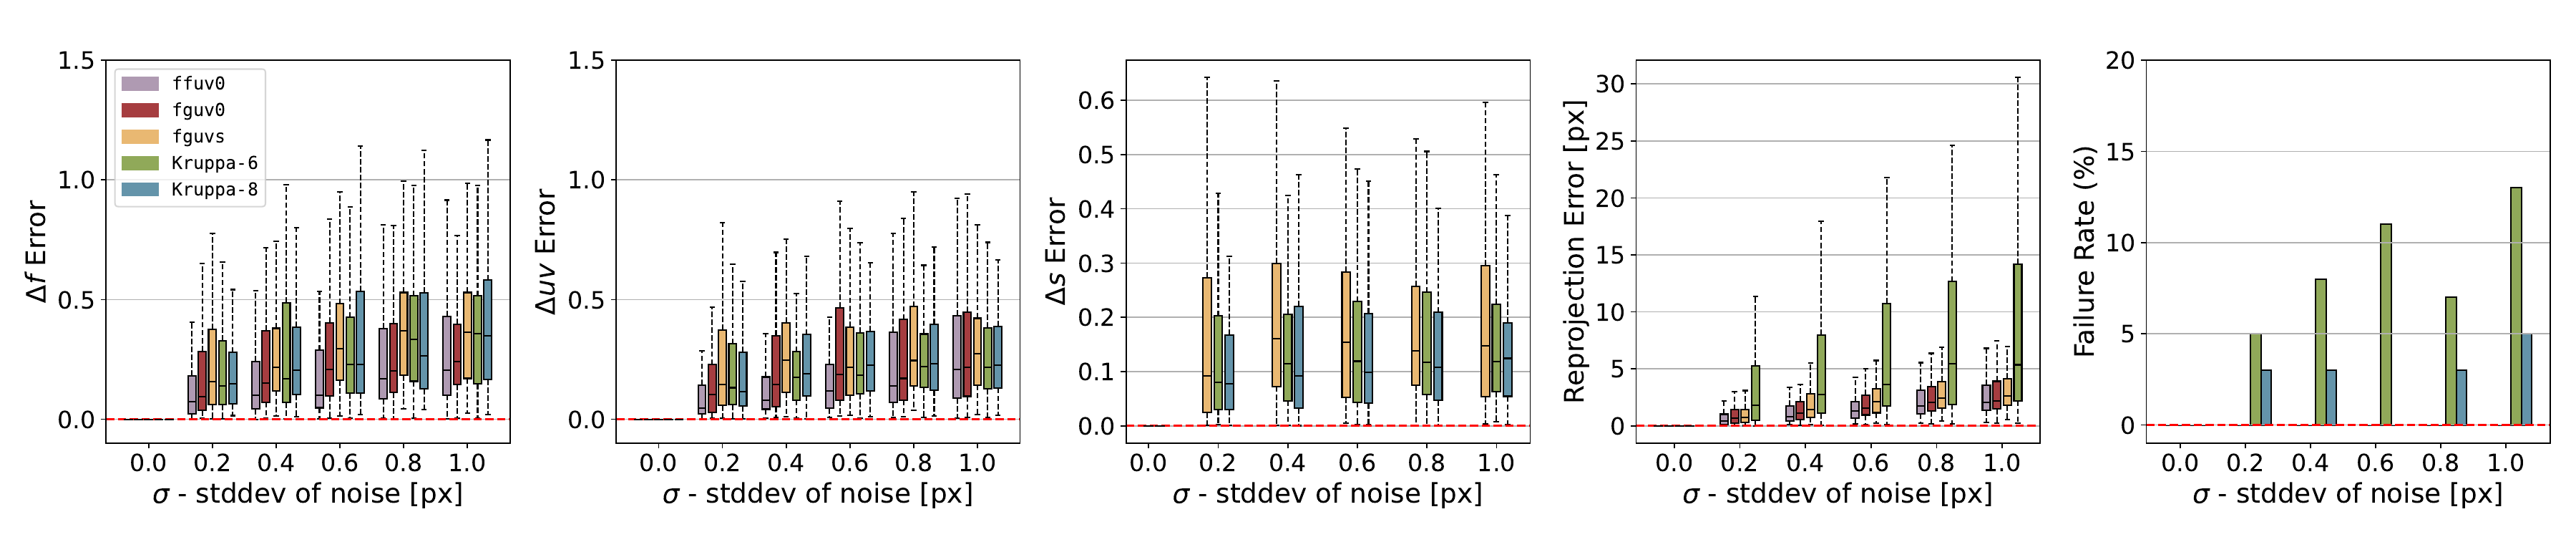}
    \caption{\textbf{Autocalibration Evaluation on Synthetic Images with Specialized Intrinsics.} Solver accuracy is assessed under varying levels of zero-mean Gaussian noise (denoted by $\sigma$ on the x-axis) applied to pixel coordinates. Mean reprojection error and relative errors in focal lengths $\Delta fg$, principal point $\Delta uv$, and skew $\Delta s$ are reported. For error measures, boxes represent the interquartile range of error distribution. The right-most plot illustrates the failure rate as a percentage, with \TT{ffuv0}, \TT{fguv0}, and \TT{fguvs} excluded due to no failures. Synthetic camera parameters vary across solvers to match their prior camera knowledge. For \TT{fguv0} we set $s = 0$, and for \TT{ffuv0} we set $f = g = 330$. Results are averaged over 1000 synthetic image sequences.
    }
    \label{SM:fig:synthetic-constant-K}
\end{figure*}

\input{supp/supp-tab-colmap}

\subsection{Error Metrics} \label{SM:sec:exp:metric}
We provide complete error definitions for the error metrics employed in our experimental evaluation within the main paper. Referring to \cref{sec:experiments}, we define the relative error $\Delta fg$ in focal lengths as follows:
\begin{equation}
\small
\Delta fg = \frac{1}{2} \left( \frac{| \hat{f} - f_\mathrm{gt} |}{f_\mathrm{gt}}  + \frac{| \hat{g} - g_\mathrm{gt} |}{g_\mathrm{gt}} \right).
\end{equation}
The reprojection error $Re$ is computed as
\begin{equation} \label{SM:eq:reprojection}
    Re = \frac{1}{N(M-1)} \sum_{i = 2}^{M} \sum_{p = 1}^{N} \| x_{ip} - \hat{x}_{ip} \|_2 \; ,
\end{equation}
where $\hat{x}_{ip}$ denotes the projection of the $p$-th point onto the $i$-th view using the estimated camera parameters:
\begin{equation}
    \hat{x}_{ip} = \frac{1}{\hat{\lambda}_{ip}} \hat{K}\,\hat{R}_i\mat{c}{I \mid -\hat{C}_i}\mat{c}{\hat{\lambda}_{1p} \hat{K}^{-1} x_{1p}\\1} \; ,
\end{equation}
where $\hat{K}, \hat{R}_i, \hat{C}_i, \hat{\lambda}_{ip}$ denote the estimated camera intrinsics, rotation, center, and projective depth of point $p$ seen by view $i$, respectively. The definition of the reprojection error $Re_\mathrm{gt}$ is consistent with \eqref{SM:eq:reprojection}, but $\hat{x}_{ip}$ is computed as:
\begin{equation}
    \hat{x}_{ip} = \frac{1}{\hat{\lambda}_{ip}} \hat{K}\,R_i\mat{c}{I \mid -C_i}\mat{c}{\hat{\lambda}_{1p} \hat{K}^{-1} x_{1p}\\1} \; ,
\end{equation}
where $R_i, C_i$ are the ground truth camera rotation and center, respectively.

In \cref{sec:experiments-real}, the angular errors $\epsilon_R$ and $\epsilon_C$ for estimated camera rotations and centers, respectively, are defined as follows:
\begin{align} \label{eq:experiments-err-rot-1}
\epsilon_R &= \frac{1}{M - 1} \sum_{i=2}^{M} \left| \; \arccos \left( \frac{\textrm{tr}(R_{i}^\top \hat{R}_{i}) - 1}{2} \right) \; \right| \; ,
\\
\label{eq:experiments-err-rot-2}
\epsilon_C &= \frac{1}{M - 1} \sum_{i=2}^{M} \left| \; \arccos\left(\frac{C_{i}^\top \hat{C}_{i}}{\|C_{i}\| \|\hat{C}_{i}\|}\right) \; \right| \; ,
\end{align}
where $\hat{R}_{i}, \hat{C}_{i}$ denote the estimated rotation and camera center, respectively, of the $i$-th camera with respect to the $i = 1$ camera, for which $R_1 = I$ and $C_1 = [0, 0, 0]$. $R_{i}, C_{i}$ denote the ground truth camera rotation and center, respectively. The values of $\epsilon_R$ and $\epsilon_C$ are expressed in degrees for all experiments.

\subsection{Synthetic Experiments --- additional details} \label{SM:sec:exp:synthetic}

We provide additional details regarding our synthetic evaluation, referring to \cref{sec:experiments-synthetic} of the main paper.

\medskip
\noindent
\textbf{Kruppa-7.} \cref{SM:fig:experiments-synthetic} presents a comparative analysis of the results achieved by the Kruppa-7 solver in relation to the \TT{ffuv0}, \TT{fguv0}, \TT{fguvs}, and Kruppa-8 solvers. Results reveal that Kruppa-7 exhibits inferior accuracy in focal length estimation ($\Delta fg$) compared to Kruppa-8, especially at lower noise levels $\sigma \geq 0.6$. Nonetheless, principal point and skew estimation accuracy are comparable to Kruppa-8. Finally, the failure rates of Kruppa-7 match or surpass those of Kruppa-8 across all noise levels $\sigma$.

\medskip
\noindent
\textbf{Evaluation with Specialized Intrinsics.} \cref{SM:fig:synthetic-constant-K} presents the results of our \TT{ffuv0} and \TT{fguv0} solvers evaluated on synthetic scenes generated using varying camera parameters that depend on the prior camera knowledge assumed by each solver. For \TT{fguvs}, Kruppa-6, and Kruppa-8, which do not assume any camera knowledge, synthetic camera parameters are set to $f = 330$, $g = 310$, $u = 300$, $v = 250$, and $s = 10$. For \TT{fguv0}, which assumes zero-skew, we set $s = 0$. Finally, for \TT{ffuv0}, which assumes squared pixel aspect ratio, we set $f = g = 330$. 

The results affirm that \TT{ffuv0} and \TT{fguv0} excel in focal length estimation and achieve comparable performance to the other solvers in principal point estimation. As expected, errors $\Delta fg$ and $\Delta uv$ are reduced due to the synthetic camera parameters perfectly matching the prior knowledge assumed by each of these solvers.

This evaluation also focuses on evaluating the theoretical correctness of our solvers, \emph{i.e.}, verifying that zero error is achieved in the noiseless case. Both \TT{ffuv0} and \TT{fguv0} attain zero errors when $\delta = 0$ and their assumed prior knowledge matches the ground truth camera parameters, confirming their theoretical correctness. As expected, our solvers do not exhibit any failures in this synthetic evaluation.

\medskip
\noindent
\textbf{Degeneracies. } As discussed in \cref{sec:experiments-synthetic}, our proposed autocalibration solvers are unaffected by the degeneracy of Kruppa-based methods arising from a singularity in the Kruppa equations when the optical centers of cameras lie on a sphere, and their optical axes intersect at the sphere's center \cite{Sturm-2000}. To verify that our solvers overcome this substantial problem, we synthetically reproduce the aforementioned degeneracy condition and assess calibration on these generated image sequences. We generate 1000 synthetic scenes that exhibit the degeneracy condition of Kruppa and verify our \TT{ffuv0}, \TT{fguv0} and \TT{fguvs} can successfully perform autocalibration in all cases, exhibiting zero-error in the noiseless case and a failure rate of 0\%. 

Furthermore, referring to \cref{sec:solving-hc}, we confirm the well-posed nature of our autocalibration problem by verifying that the Jacobian of the given relaxed system $\mathbf{g}(\mathbf{p}, \mathbf{x}) = 0$ is full-rank at the synthetic solution $(\mathbf{p}_0, \mathbf{x}_0)$. Additionally, we observe that the least singular value of the Jacobian of the system never falls below $10^{-4}$ in our testing. This indicates the robust numerical stability of our solvers.

We implement code to generate degenerate image sequences for Kruppa equations and verify that our solvers are unaffected by this problem. The code is implemented in Julia and is publicly available at {\small \href{https://github.com/andreadalcin/MinimalPerspectiveAutocalibration}{github.com/andreadalcin/MinimalPerspectiveAutocalibration}}.

\subsection{Autocalibration in COLMAP ---\\additional details}
Finally, we provide further details on evaluating the COLMAP integration of our autocalibration solvers.

\medskip
\noindent
\textbf{Datasets.} For Fountain-P11 \cite{strecha2008benchmarking}, we consider the 0-2-4 and 0-3-6 image triplets. Rathaus \cite{strecha2008benchmarking} includes a single calibrated image triplet. For KITTI-Depth \cite{geiger2012we}, we extract image triplets from the 2011-09-26-drive-0005 sequence.

\medskip
\noindent
\textbf{Results.} \cref{SM:tab:colmap} provides an extended view of \cref{tab:experiments-colmap}, including the results achieved by $\text{COLMAP}_\mathtt{ffuv0}$ --- the initialization strategy of $K$ based on the \TT{ffuv0} solver. This variant excludes $K$ from Bundle Adjustment (BA), and we present results achieved by $\text{COLMAP}_\mathtt{ffuv0}$ when BA is applied to $K$. The calibration accuracy of $\text{COLMAP}_\mathtt{ffuv0}$ surpasses that of $\text{COLMAP}_\mathtt{fguv0}$ marginally, particularly in terms of principal point estimation ($\Delta uv$). When Bundle Adjustment is extended to $K$, the disparity in performance diminishes and becomes negligible, especially in the Fountain-P11 and Rathaus datasets. Notably, in KITTI-Depth, extending Bundle Adjustment to $K$ shows that $\text{COLMAP}_\mathtt{ffuv0}$ achieves a slightly lower accuracy in focal lengths ($\Delta fg$) but exhibits improved accuracy in the principal point ($\Delta uv$).

\medskip
\noindent
\textbf{Discussion.} In the context of integrating our autocalibration solvers into COLMAP, both \TT{ffuv0} and \TT{fguv0} demonstrate similar accuracy in both $\Delta fg$ and $\Delta uv$, particularly when extending Bundle Adjustment to $K$. Consequently, opting for \TT{fguv0} as an initialization strategy in COLMAP is preferable for many practical applications. This preference is attributed to the faster processing speed of \TT{fguv0} over \TT{ffuv0} (1.78 s/iter compared to 9.21 s/iter) and its support for cameras without square pixel aspect ratio.
