# Supplementary material for: Minimal Perspective Autocalibration
Source: arXiv:2405.05605 source file (2024-05-09)
Supplement: Supplementary file 4 [file figure.tex]

\begin{figure*}[t]
  \centering
  \begin{subfigure}[b]{0.25\textwidth}
    \centering
    \includegraphics[width=\textwidth]{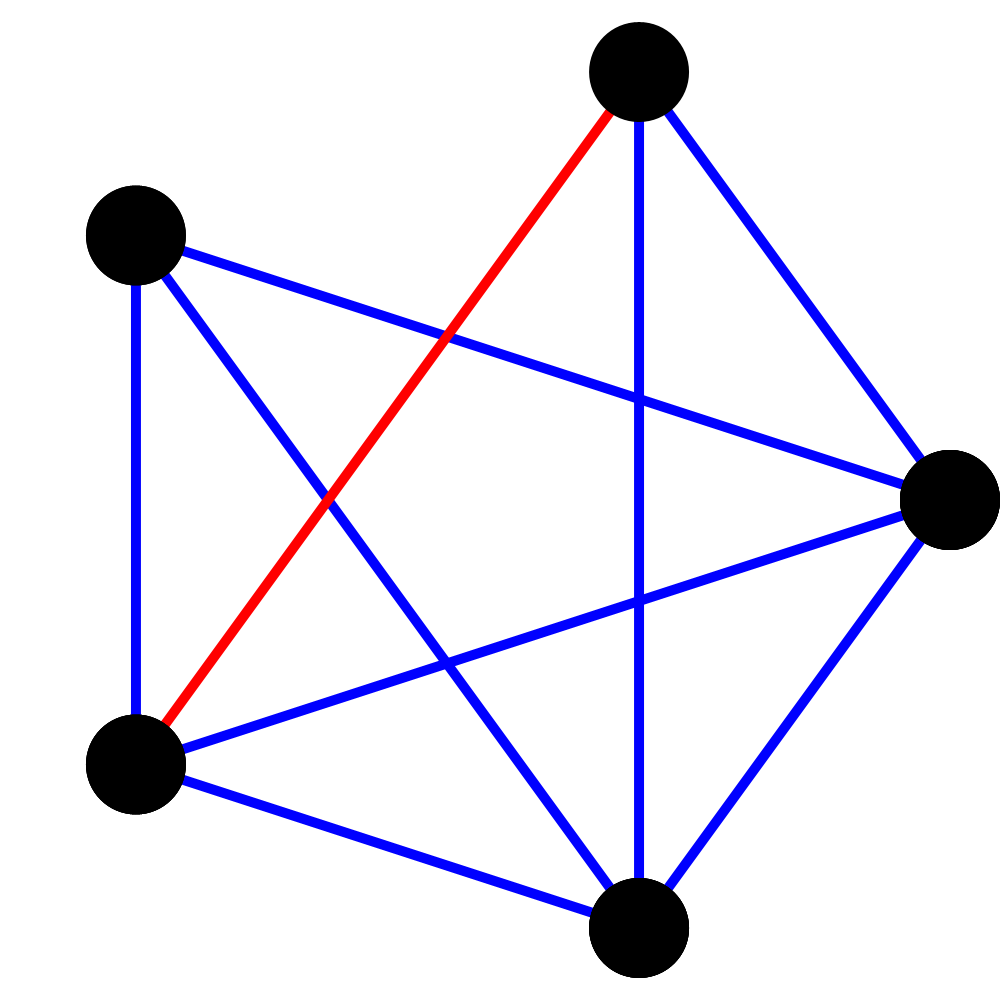}
    \caption{$\mathtt{ffuv0}$}
    \label{SM:fig:relaxation:ffuv0}
  \end{subfigure}
  \hfill
  \begin{subfigure}[b]{0.25\textwidth}
    \centering
    \includegraphics[width=\textwidth]{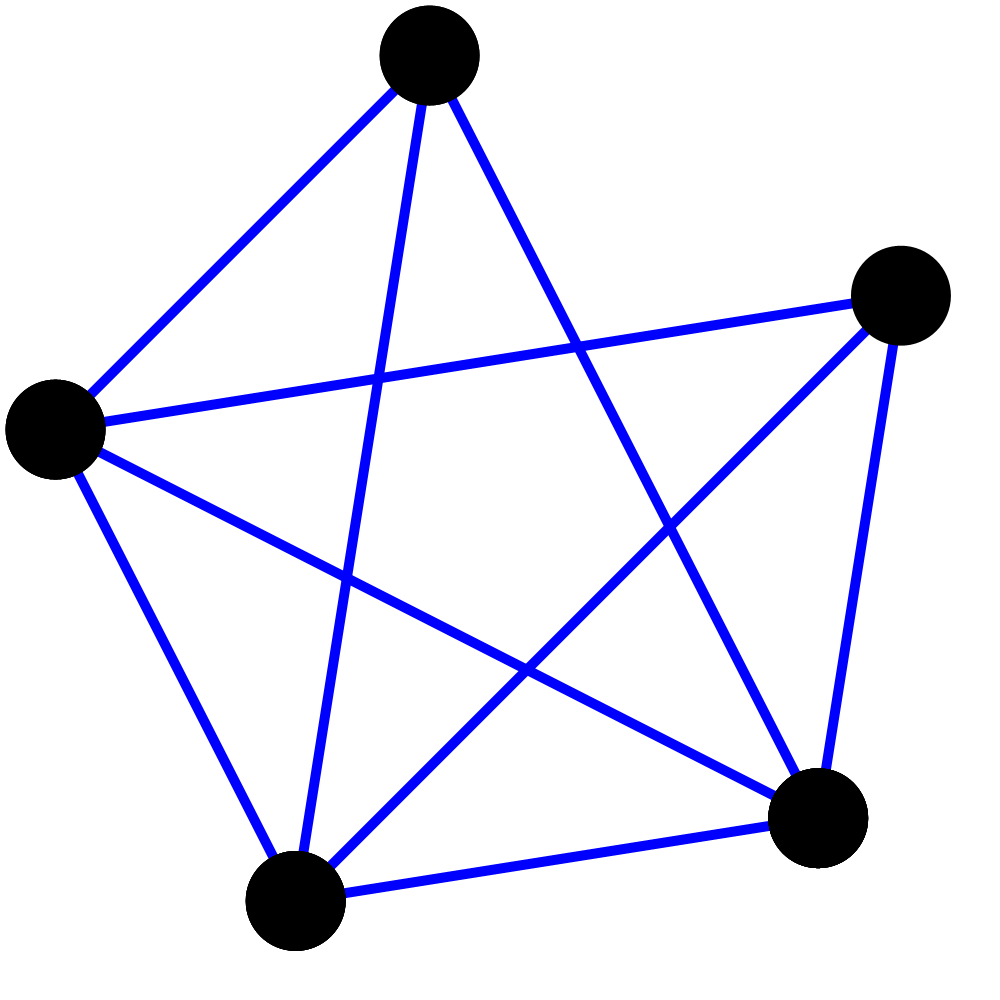}
    \caption{$\mathtt{fguv0}$}
    \label{SM:fig:relaxation:fguv0}
  \end{subfigure}
  \hfill
  \begin{subfigure}[b]{0.25\textwidth}
    \centering
    \includegraphics[width=\textwidth]{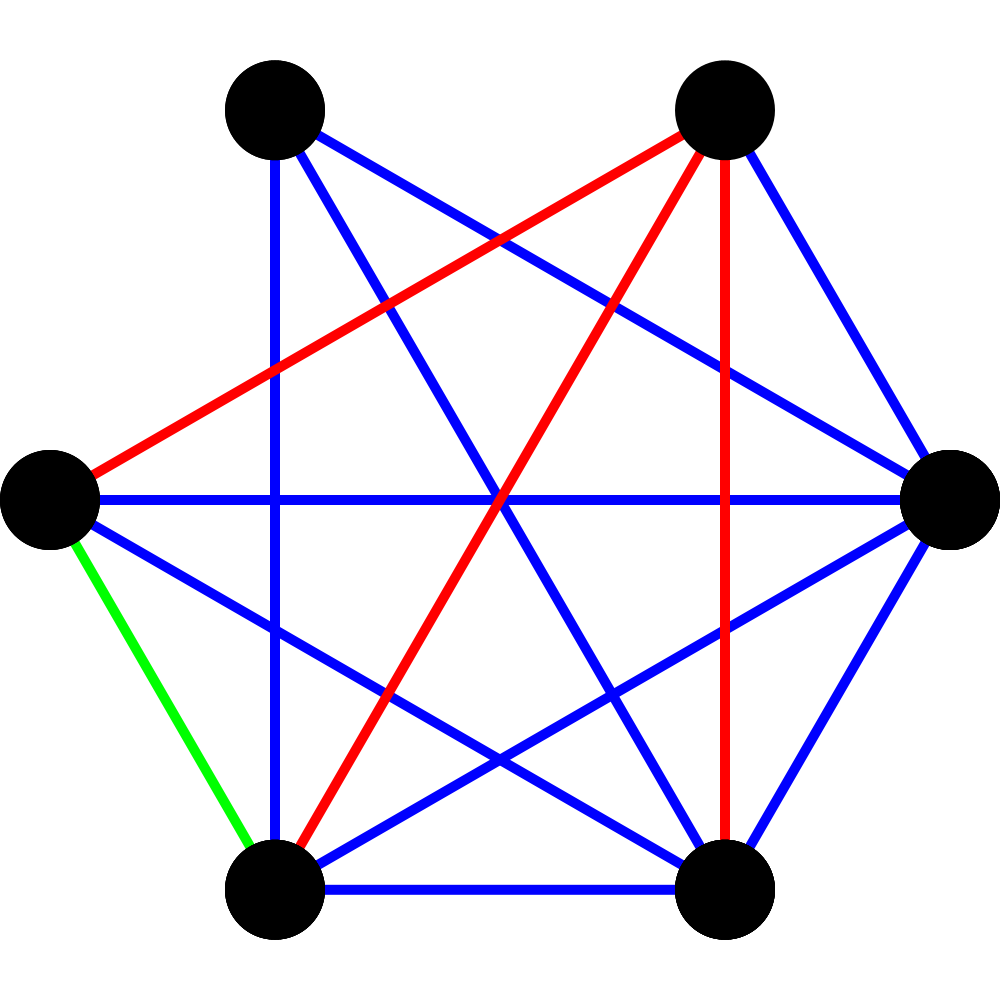}
    \caption{$\mathtt{fguvs}$}
    \label{SM:fig:relaxation:fguvs}
  \end{subfigure}
  \caption{4-colorings of the minimal relaxations used in our implementation of solvers for the $\mathtt{ffuv0}$, $\mathtt{fguv0}$ and $\mathtt{fguvs}$ problems.}
\end{figure*}
