# Supplementary material for: Minimal Perspective Autocalibration
Source: arXiv:2405.05605 source file (2024-05-09)
Supplement: Supplementary file 5 [file supp-tab-autocalibration.tex]

% \renewcommand{\arraystretch}{0.975}
\begin{table*}[ht]
    \centering
    {\tiny
    \vspace{-2.0em}
    \begin{tabular}{|c|c|c|c|cc|c|c||c|c|c|c|cc|c|c|} 
         \hline
         Prior on $K$ & $M$ & $N$ & $L$ & Min \# sol. in $\mathbb{C}$ & Max \# sol. in $\mathbb{C}$ & $\# \text{balanced} $ & $\# \bg$ & Prior on $K$ & $M$ & $N$ & $L$ & Min \# sol. in $\mathbb{C}$ & Max \# sol. in $\mathbb{C}$ & $\# \text{balanced} $ & $\# \bg$ \\ \hline
         \TT{fguvs} & 2 & - & 0 & $\infty$ & $\infty$ & 0 & 0 & \TT{1g0vs} & 2 & - & 2 & $\infty$ & $\infty$ & 0 & 0 \\ 
         \TT{fguvs} & 3 & 6 & 0 & $11940^\ast $ & $4544808^\ast$ & 5852925 & 3313 & \TT{1g0vs} & 3 & 5 & 2 & 58024 & 631306 & 1140 & 8 \\ \hline 
         \TT{fguv0} & 2 & - & 1 & $\infty$ & $\infty$ & 0 & 0 & \TT{1g0v0} & 2 & 7 & 3 & 36 & 36 & 1 & 1 \\ 
         \TT{fguv0} & 3 & 5 & 1 & 9252 & 9252 & 190 & 3 & \TT{1g0v0} & 3 & 5 & 3 & 8800 & 205568 & 4845 & 37 \\ \hline 
         \TT{fgu0s} & 2 & - & 1 & $\infty$ & $\infty$ & 0 & 0 & \TT{1g00s} & 2 & 7 & 3 & 48 & 48 & 1 & 1 \\ 
         \TT{fgu0s} & 3 & 5 & 1 & 8232 & 8232 & 190 & 3 & \TT{1g00s} & 3 & 5 & 3 & 8960 & 477088 & 4845 & 37 \\ \hline 
         \TT{fgu00} & 2 & - & 2 & $\infty$ & $\infty$ & 0 & 0 & \TT{1g000} & 2 & 6 & 4 & 60 & 60 & 1 & 1 \\ 
         \TT{fgu00} & 3 & 5 & 2 & 38744 & 134424 & 1140 & 8 & \TT{1g000} & 3 & 4 & 4 & 1336 & 1336 & 1 & 1 \\ \hline 
         \TT{fg0vs} & 2 & - & 1 & $\infty$ & $\infty$ & 0 & 0 & \TT{11uvs} & 2 & - & 2 & $\infty$ & $\infty$ & 0 & 0 \\ 
         \TT{fg0vs} & 3 & 5 & 1 & 8232 & 8232 & 190 & 3 & \TT{11uvs} & 3 & 5 & 2 & 57912 & 201265 & 1140 & 8 \\ \hline 
         \TT{fg0v0} & 2 & - & 2 & $\infty$ & $\infty$ & 0 & 0 & \TT{11uv0} & 2 & 7 & 3 & 48 & 48 & 1 & 1 \\ 
         \TT{fg0v0} & 3 & 5 & 2 & 38744 & 450080 & 1140 & 8 & \TT{11uv0} & 3 & 5 & 3 & 8940 & 477080 & 4845 & 37 \\ \hline 
         \TT{fg00s} & 2 & - & 2 & $\infty$ & $\infty$ & 0 & 0 & \TT{11u0s} & 2 & 7 & 3 & 36 & 36 & 1 & 1 \\ 
         \TT{fg00s} & 3 & 5 & 2 & 38744 & 134424 & 1140 & 8 & \TT{11u0s} & 3 & 5 & 3 & 8786 & 46192 & 4845 & 37  \\ \hline 
         \TT{fg000} & 2 & 7 & 3 & 72 & 72 & 1 & 1 & \TT{11u00} & 2 & 6 & 4 & 60 & 60 & 1 & 1 \\
         \TT{fg000} & 3 & 5 & 3 & 15536 & 830656 & 4845 & 37 & \TT{11u00} & 3 & 4 & 4 & 1336 & 1336 & 1 & 1 \\ \hline
         \TT{f1uvs} & 2 & - & 2 & $\infty$ & $\infty$ & 0 & 0 & \TT{110vs} & 2 & 7 & 3 & 72 & 72 &  1 & 1 \\ 
         \TT{f1uvs} & 3 & 5 & 2 & 8222 & 8222 & 190 & 3 & \TT{110vs} & 3 & 5 & 3 & 16390 & 85480 & 4845 & 37  \\ \hline 
         \TT{f1uv0} & 2 & - & 2 & $\infty$ & $\infty$ & 0 & 0 & \TT{110v0} & 2 & 6 & 4 & 60 & 60 & 1 & 1 \\ 
         \TT{f1uv0} & 3 & 5 & 2 & 58088	& 201632 & 1140 & 8 & \TT{110v0} & 3 & 4 & 4 & 1336 & 1336 & 1 & 1 \\ \hline
         \TT{f1u0s} & 2 & - & 2 & $\infty$ & $\infty$ & 1 & 1 & \TT{1100s} & 2 & 6 & 4 & 60 & 60 & 1 & 1 \\ 
         \TT{f1u0s} & 3 & 5 & 2 & 29520 & 320380 & 1140 & 8 & \TT{1100s} & 3 & 4 & 4 & 1336 & 1336 & 1 & 1 \\ \hline 
         \TT{f1u00} & 2 & 7 & 3 & 36 & 36 & 1 & 1 & \TT{11000} & 2 & 5 & 5 & 20 & 20 & 1 & 1 \\ 
         \TT{f1u00} & 3 & 5 & 3 & 8800 & 489088 & 4845 & 37 & \TT{11000} & 3 & 4 & 5 & 640 & 640 & 1 & 1 \\ \hline
         \TT{f10vs} & 2 & - & 2 & $\infty$ & $\infty$ & 0 & 0 & \TT{ffuvs} & 2 & - & 1 &$ \infty$ & $\infty$ & 0 & 0\\ 
         \TT{f10vs} & 3 & 5 & 2 & 48664 & 173078 & 1140 & 8 & \TT{ffuvs} & 3 & 5 & 1 & 9234 & 9234 & 190 & 3 \\ \hline 
         \TT{f10v0} & 2 & 7 & 3 & 72 & 72 & 1 & 1 & \TT{ffuv0} & 2 & - & 2 & $\infty$ & $\infty$ & 0 & 0 \\
         \TT{f10v0} & 3 & 5 & 3 & 15528 & 114440 & 4845 & 37 & \TT{ffuv0} & 3 & 5 & 2 & 32376 & 238238 & 1140 & 8 \\ \hline
         \TT{f100s} & 2 & 7 & 3 & 36 & 36 & 1 & 1 & \TT{ffu0s} & 2 & - & 2 & $\infty$ & $\infty$ & 0 & 0 \\
         \TT{f100s} & 3 & 5 & 3 & 8784 & 205556 & 4845 & 37 & \TT{ffu0s} & 3 & 5 & 2 & 58056 & 201516 & 1140 & 8 \\ \hline
         \TT{f1000} & 2 & 6 & 4 & 60 & 60 & 1 & 1 & \TT{ffu00} & 2 & 7 & 3 & 48 & 48 & 1 & 1 \\
         \TT{f1000} & 3 & 4 & 4 & 1336 & 1336 & 1 & 1 & \TT{ffu00} & 3 & 5 & 3 & 8968 & 353984 & 4845 & 37 \\ \hline
         \TT{1guvs} & 2 & - & 1 & $\infty$ & $\infty$ & 0 & 0 & \TT{ff0vs} & 2 & - & 2 & $\infty$ & $\infty$ & 0 & 0 \\ 
         \TT{1guvs} & 3 & 5 & 1 & 8720 & 8720 & 190 & 3 & \TT{ff0vs} & 3 & 5 & 2 & 77400 & 268704 & 1140 & 8 \\ \hline 
         \TT{1guv0} & 2 & - & 2 & $\infty$ & $\infty$ & 0 & 0 &  \TT{ff0v0} & 2 & 7 & 3 & 48 & 48 & 1 & 1 \\ 
         \TT{1guv0} & 3 & 5 & 2 & 58092 & 201616 & 1140 & 8 & \TT{ff0v0} & 3 & 5 & 3 & 8968 & 184672 & 4845 & 37 \\ \hline 
         \TT{1gu0s} & 2 & - & 2 & $\infty$ & $\infty$ & 0 & 0 & \TT{ff00s} & 2 & 7 & 3 & 72 & 72 & 1 & 1 \\ 
         \TT{1gu0s} & 3 & 5 & 2 & 58048	& 201436 & 1140 & 8 & \TT{ff00s} & 3 & 5 & 3 & 15512 & 792084 & 4845 & 37 \\ \hline 
         \TT{1gu00} & 2 & 7 & 3 & 72 & 72 & 1 & 1 & \TT{ff000} & 2 & 6 & 4 & 60 & 60 & 1 & 1 \\
         \TT{1gu00} & 3 & 5 & 3 & 15520 & 86630 & 4845 & 37 & \TT{ff000} & 3 & 4 & 4 & 1336 & 1336 & 1 & 1 \\ \hline
    \end{tabular}
    }
\caption{\textbf{80 classes of minimal autocalibration problems} for $M \in \{ 2, 3 \}$ views. 
Solution counts refer to unknown depths and the unknown enries of $K$ in~\eqref{SM:eq:depth-equation-2}. 
Other notation and conventoions are the same as in~\Cref{tab:Minimal-Autocalibration-Substitution-Tab}.}
\label{SM:Tab:minimal-autocalibration}
\end{table*}
