# Supplementary material for: Minimal Perspective Autocalibration
Source: arXiv:2405.05605 source file (2024-05-09)
Supplement: Supplementary file 6 [file supp-tab-colmap.tex]

\renewcommand{\arraystretch}{1.2}
\begin{table*}[t]
\centering
\resizebox{0.99\linewidth}{!}{
\begin{tabular}{@{}lcccccccccccccccccc@{}}
\toprule
& \multicolumn{4}{c}{Fountain-P11}
& \multicolumn{4}{c}{Rathaus}
& \multicolumn{4}{c}{KITTI-Depth} \\
\cmidrule(l){2-5} \cmidrule(l){6-9} \cmidrule(l){10-13}
Variant &
  $\Delta fg \downarrow$ &
  $\Delta uv \downarrow$ &
  $Re$ &
  Points3D &
  $\Delta fg \downarrow$ &
  $\Delta uv \downarrow$ &
  $Re$ &
  Points3D &
  $\Delta fg \downarrow$ &
  $\Delta uv \downarrow$ &
  $Re$ &
  Points3D \\ \midrule
$\text{COLMAP}_\mathrm{guess}$ & 0.3350 & 0.0140 & 0.444 & 4848 & 0.0671 & 0.0812 & 0.624 & 847 & 0.6510 & 0.1360 & 0.810 & 210 \\
$\text{COLMAP}_\texttt{ffuv0}$ & 0.0053 & 0.0281 & 0.238 & 5357 & 0.0215 & 0.0102 & 0.441 & 831 & 0.0698 & 0.0161 & 0.402 & 231 \\
$\text{COLMAP}_\texttt{fguv0}$ & 0.0058 & 0.0297 & 0.241 & 5356 & 0.0237 & 0.0111 & 0.450 & 823 & 0.0720 & 0.0185 & 0.409 & 231 \\
$\text{COLMAP}_\mathrm{guess}$ + $K\text{-BA}$ & 0.0012 & 0.0013 & 0.212 & 5296 & 0.0185 & 0.0607 & 0.435 & 868 & 0.3480 & 0.5072 & 0.547 & 232 \\
$\text{COLMAP}_\texttt{ffuv0}$ + $K\text{-BA}$ & 0.0011 & 0.0012 & 0.212 & 5367 & 0.0165 & 0.0305 & 0.431 & 823 & 0.0691 & 0.1281 & 0.401 & 236 \\
$\text{COLMAP}_\texttt{fguv0}$ + $K\text{-BA}$ & 0.0011 & 0.0012 & 0.212 & 5367 & 0.0165 & 0.0307 & 0.432 & 823 & 0.0626 & 0.1773 & 0.404 & 236 \\ \midrule
$\text{COLMAP}_\mathrm{gt}$ + $K\text{-BA}$ & 0.0013 & 0.0011 & 0.210 & 5368 & 0.0069 & 0.0291 & 0.430 & 794 & 0.0401 & 0.0553 & 0.398 & 237 \\ 
\bottomrule
\end{tabular}
}
\caption{
Comparing errors and numbers of registered points for autocalibration strategies in COLMAP.
} 
\label{SM:tab:colmap}
\end{table*}
