# Supplementary material for: Minimal Perspective Autocalibration
Source: arXiv:2405.05605 source file (2024-05-09)
Supplement: Supplementary file 7 [file supp-tab-graphs.tex]

\begin{table*}
\centering
{ 
\footnotesize
\begin{tabular}[t]{|c|c|c|c|cccccccc|c|}
\hline
Prior on $K$ & $M$ & $N$ & $L$ & \multicolumn{8}{c|}{Sol. in $\mathbb{C}$ for isomorphism class} & \#$\bg$ \\ \hline
\TT{fguv0} & 3 & 5 & 1 & 2313 & 2313 & 2313 & & & & & & 3 \\
& & & &
\includegraphics[width=0.06\textwidth]{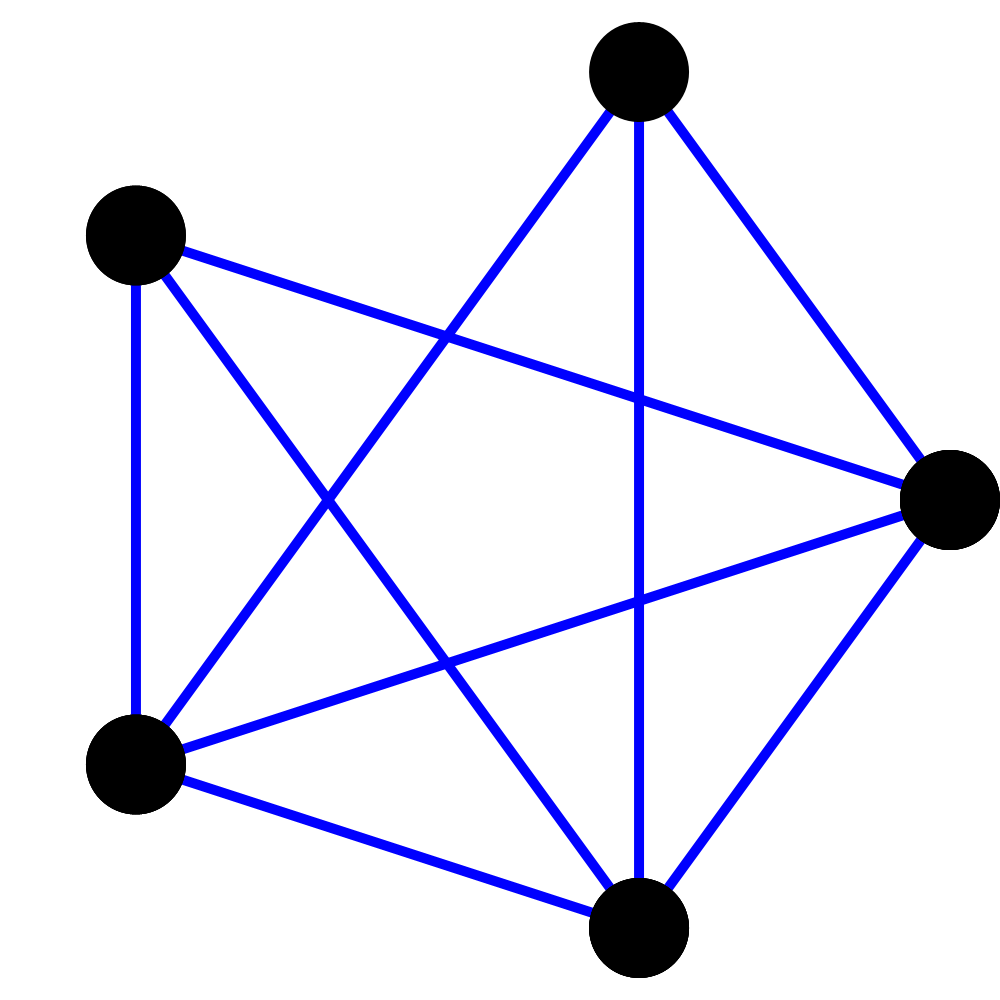} & \includegraphics[width=0.06\textwidth]{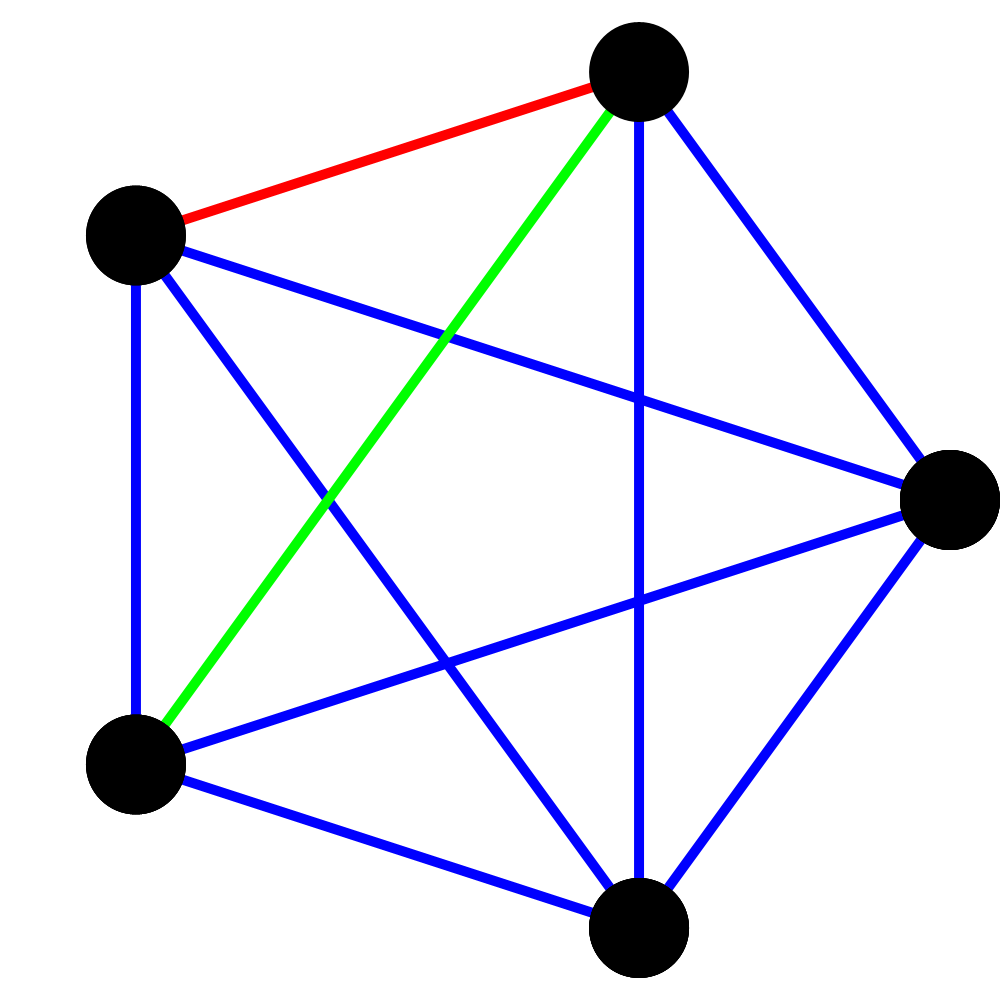} &
\includegraphics[width=0.06\textwidth]{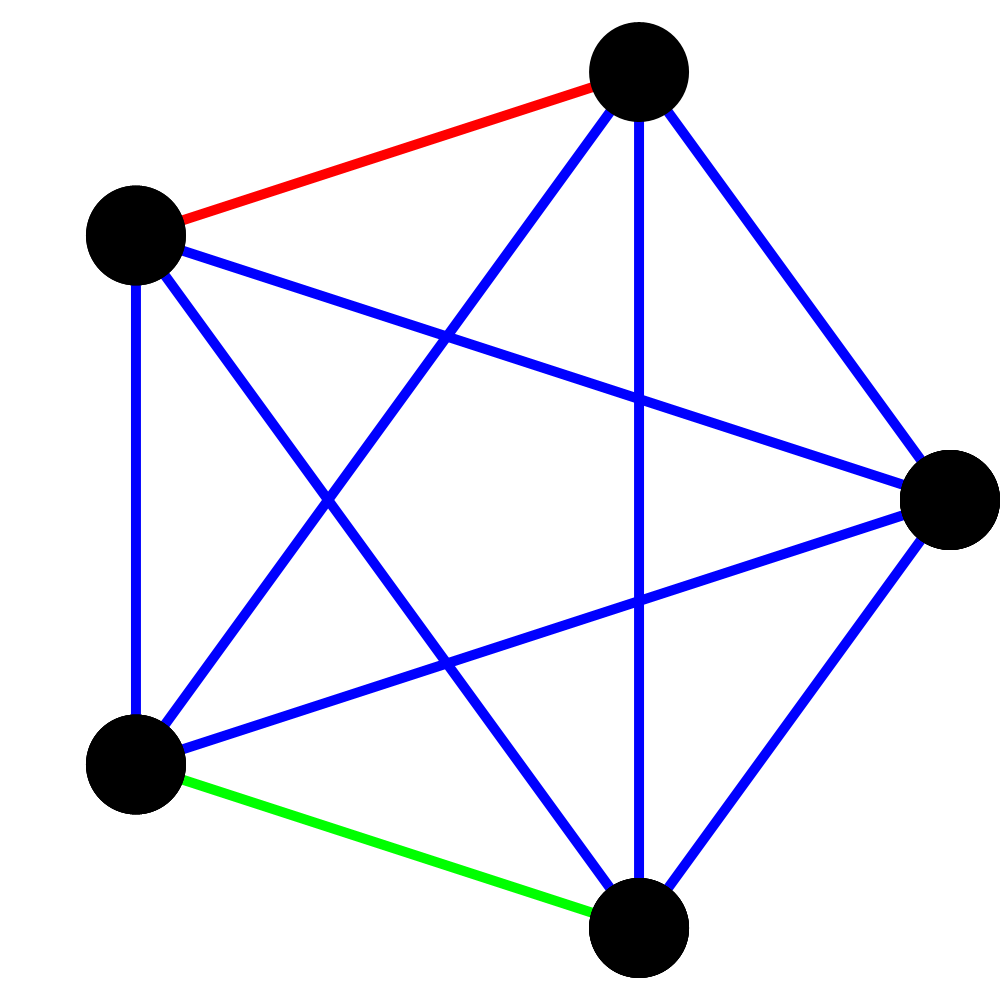} & & & & & & \\
\hline
\TT{fgu00} & 3 & 5 & 2 & 9686 & 9686 & 9686 & 9686 & 9686 & 33606 & 33606 & 33606 & 8 \\
& & & &
\includegraphics[width=0.06\textwidth]{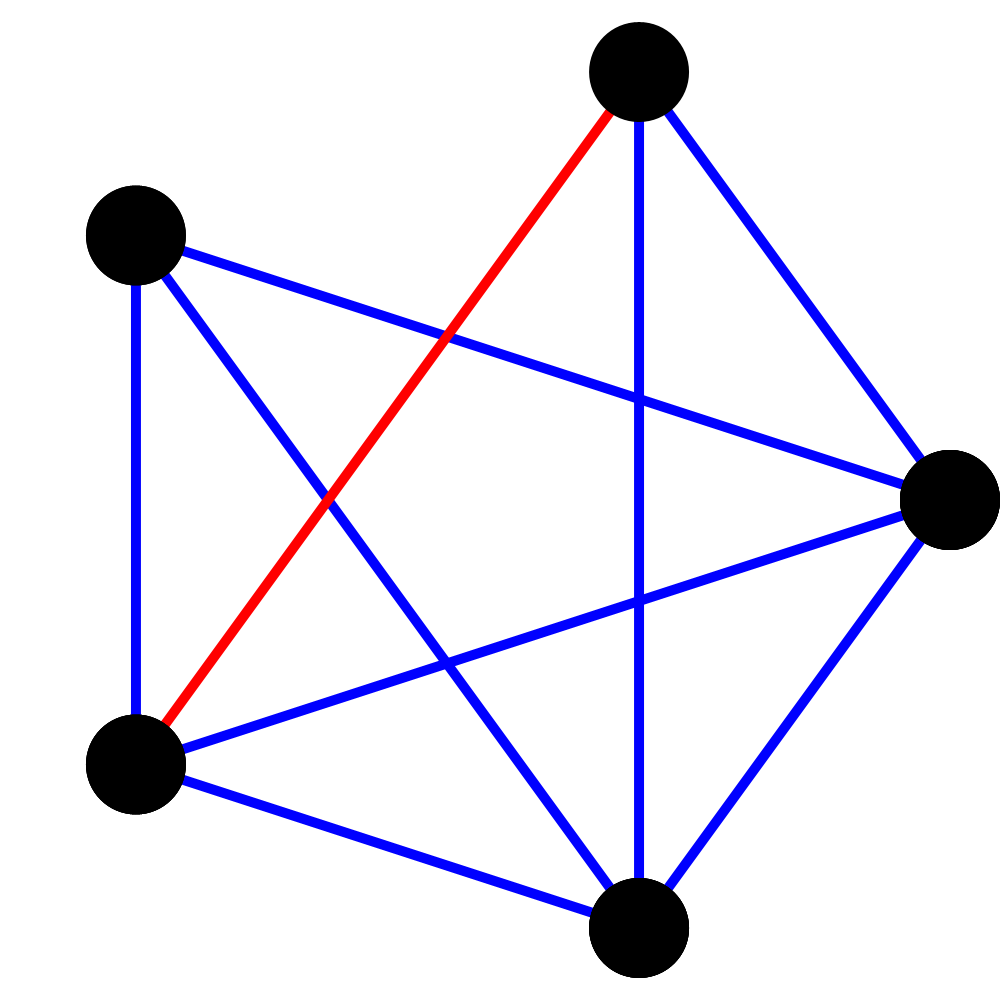} & \includegraphics[width=0.06\textwidth]{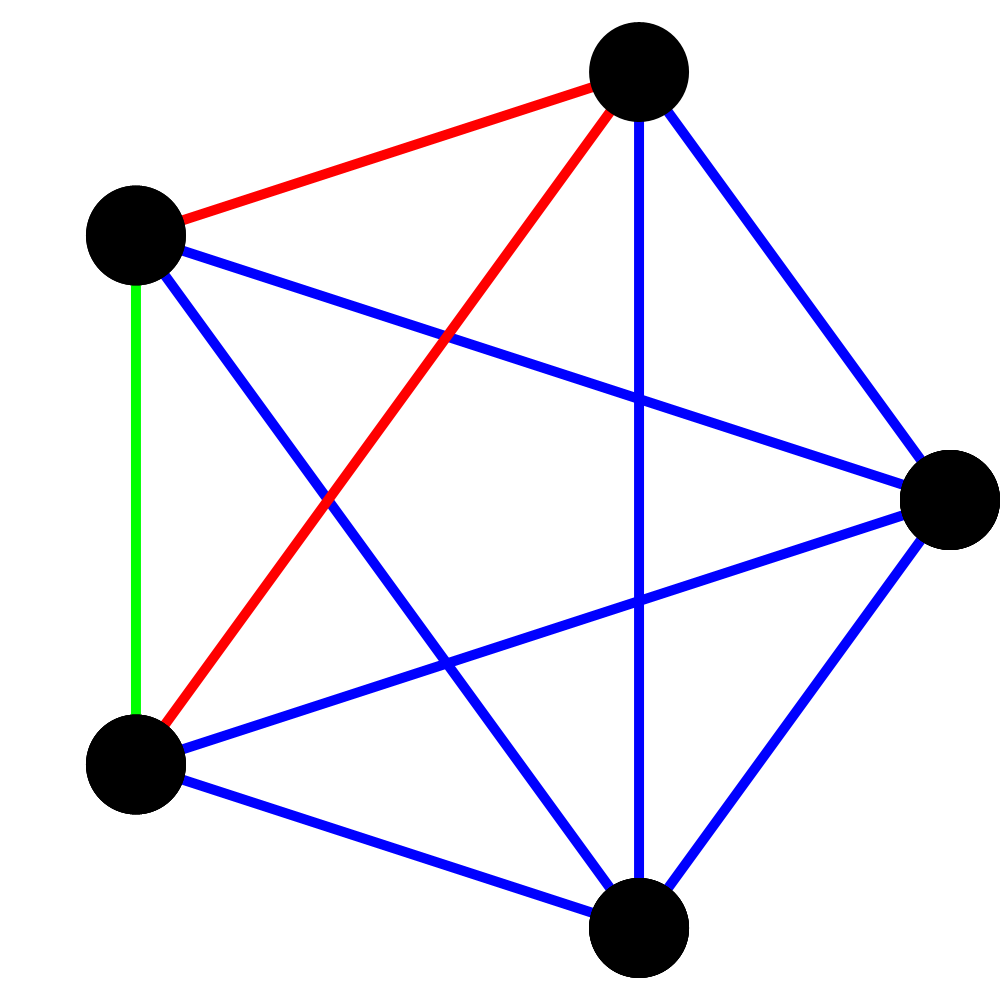} &
\includegraphics[width=0.06\textwidth]{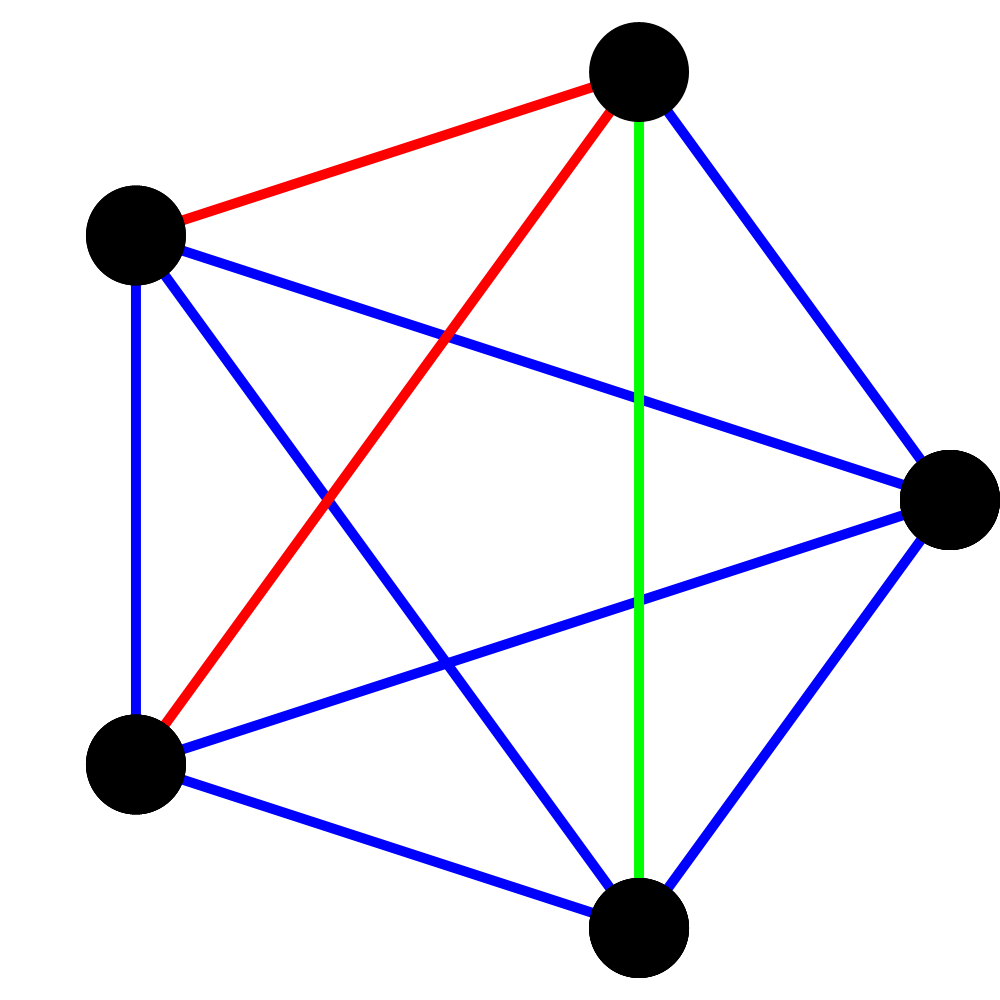} &
\includegraphics[width=0.06\textwidth]{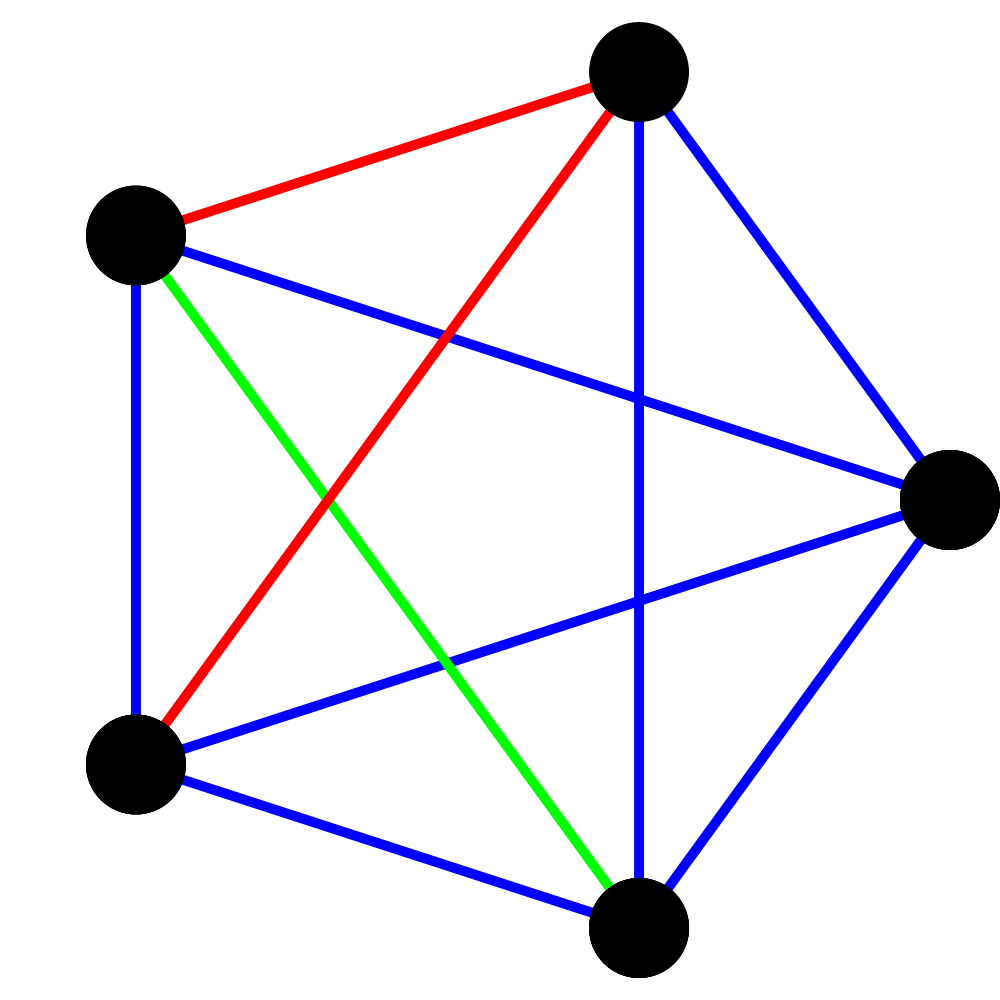} & \includegraphics[width=0.06\textwidth]{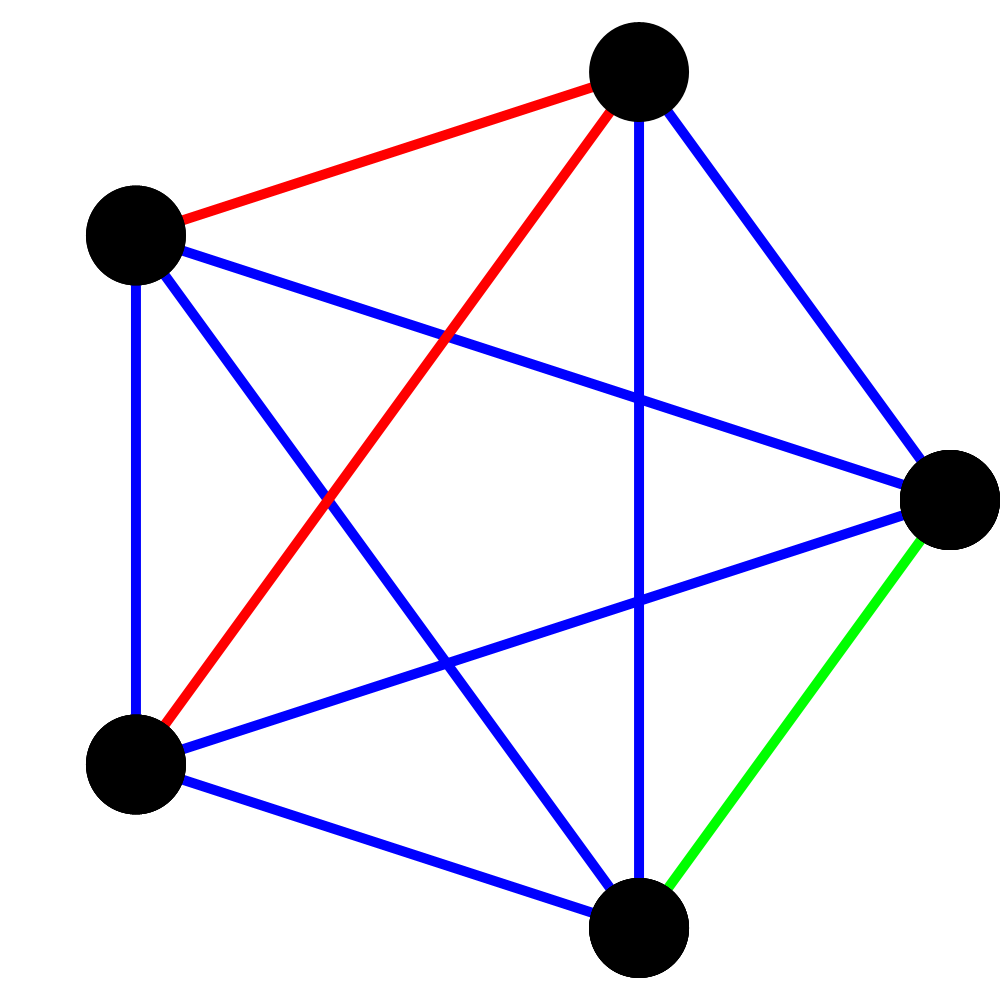} &
\includegraphics[width=0.06\textwidth]{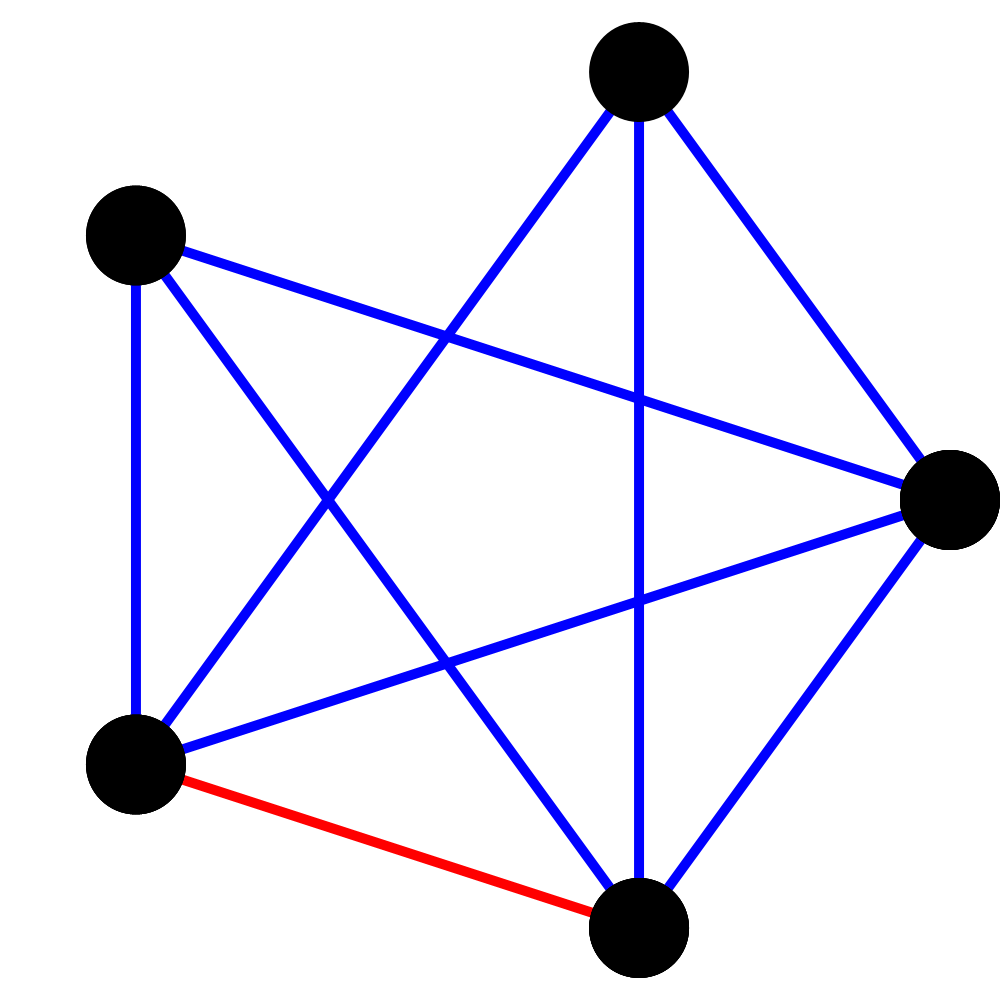} &
\includegraphics[width=0.06\textwidth]{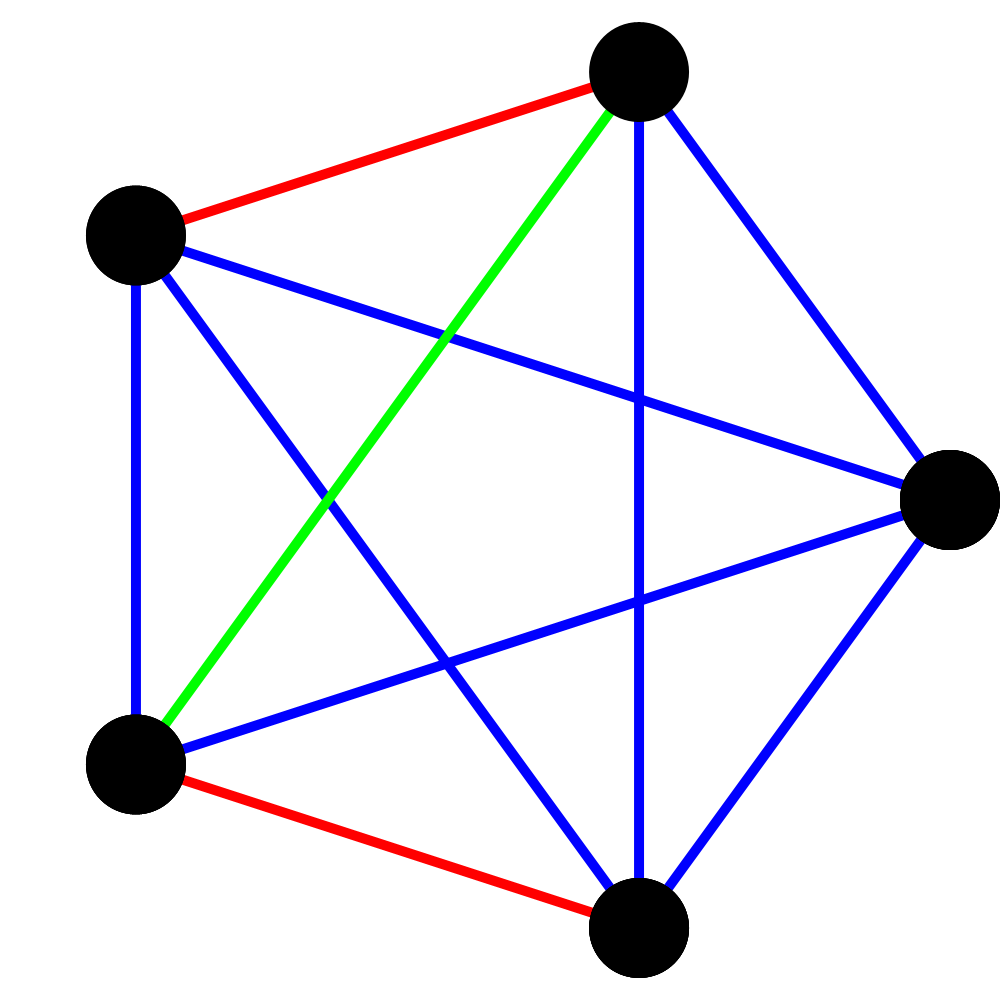} &
\includegraphics[width=0.06\textwidth]{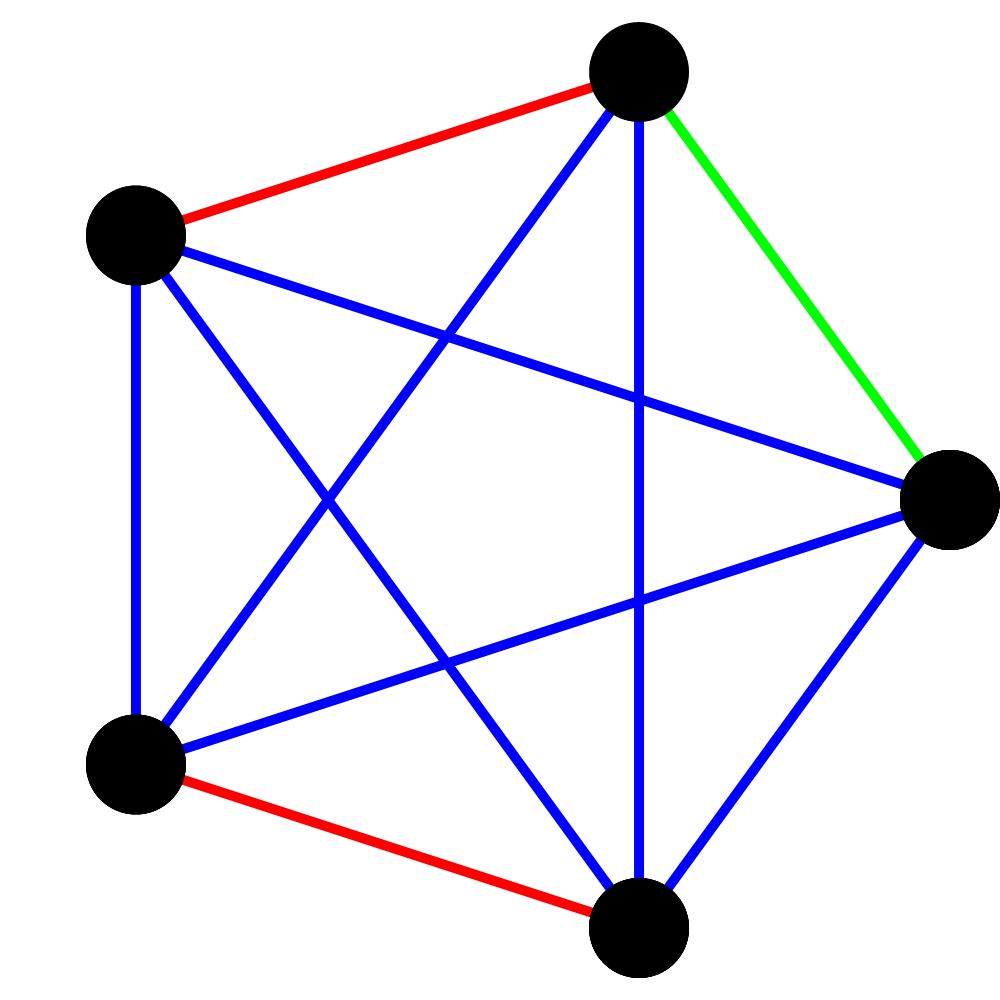} & \\
\hline
\TT{fg000} & 3 & 5 & 3 & 17624 & 17624 & 17624 & 3884 & 3884 & 3884 & 3884 & 19696 & 37 \\
& & & &
\includegraphics[width=0.06\textwidth]{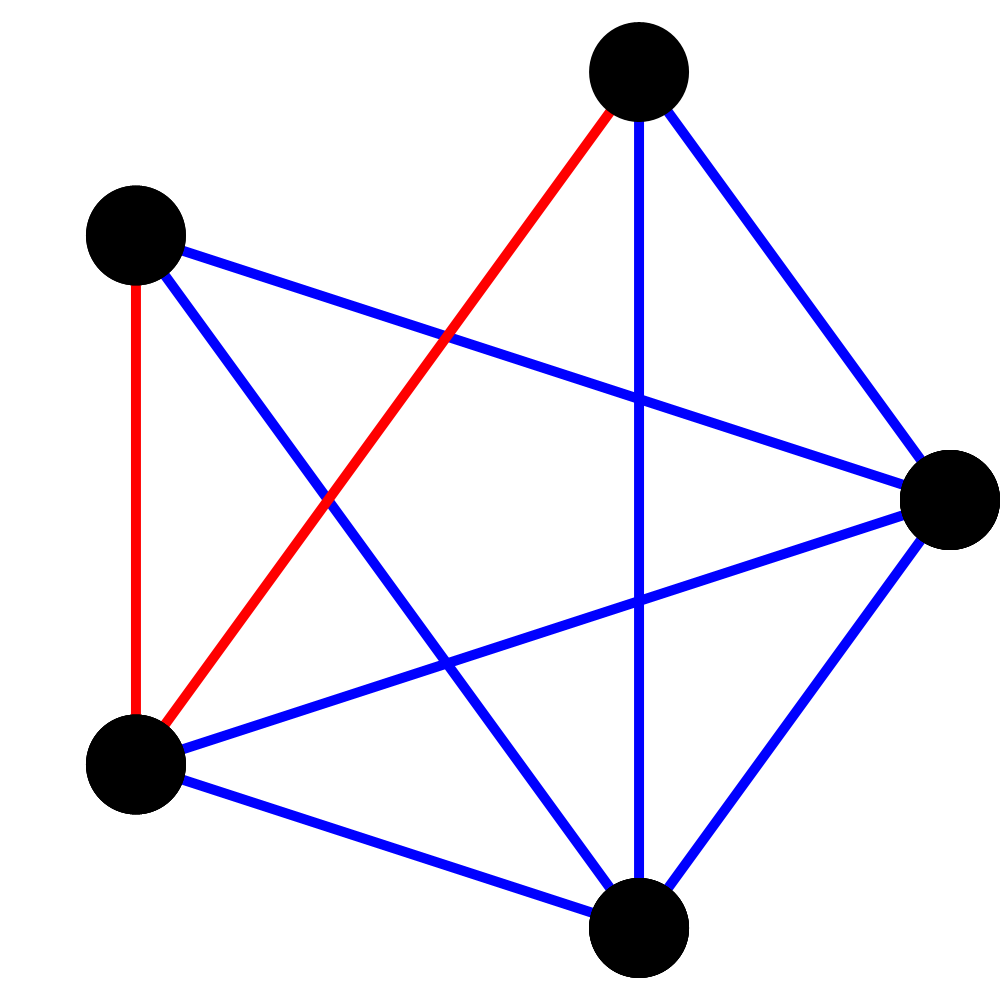} & 
\includegraphics[width=0.06\textwidth]{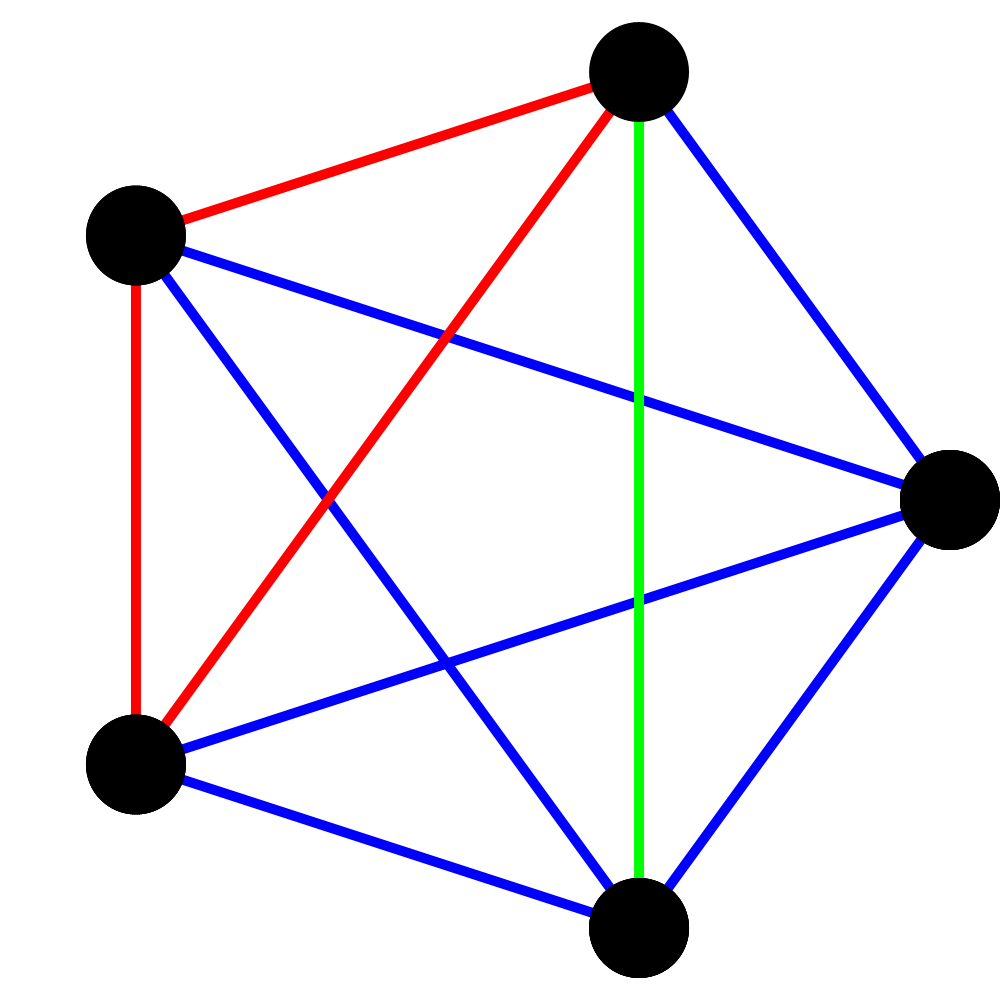} &
\includegraphics[width=0.06\textwidth]{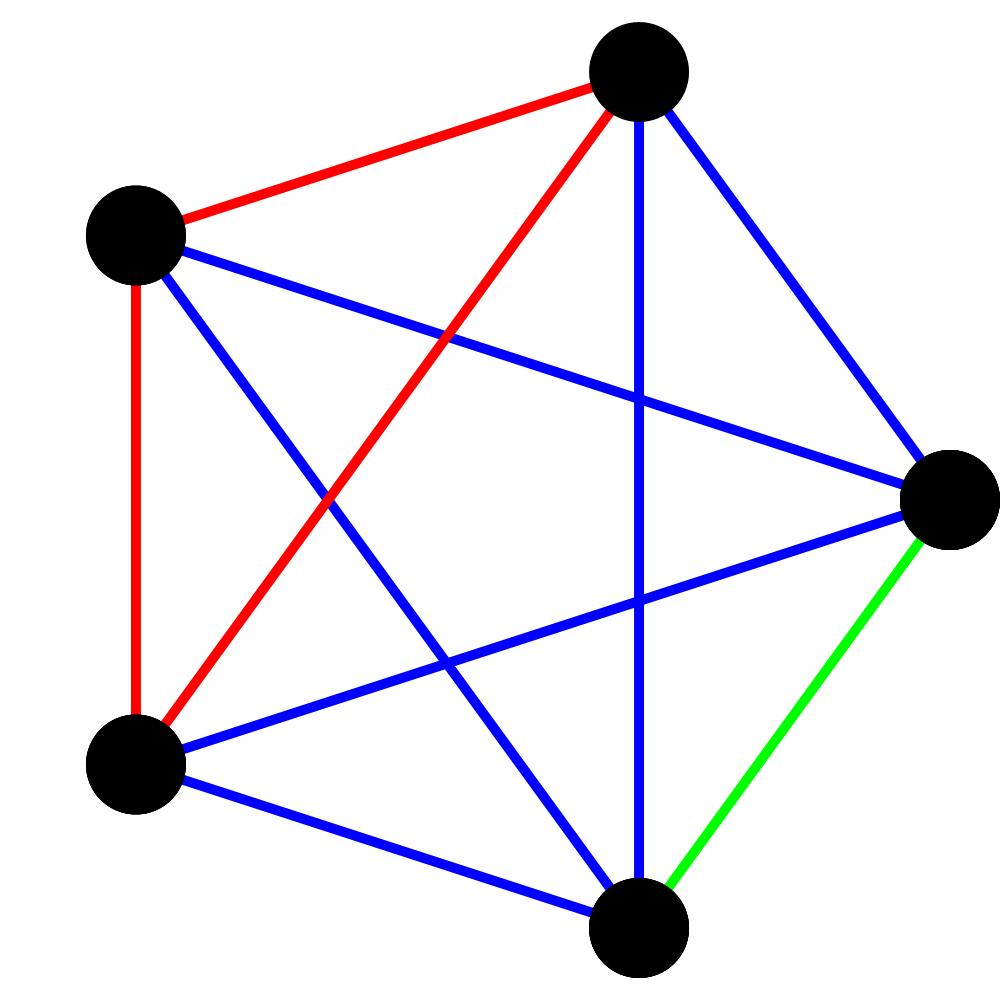} &
\includegraphics[width=0.06\textwidth]{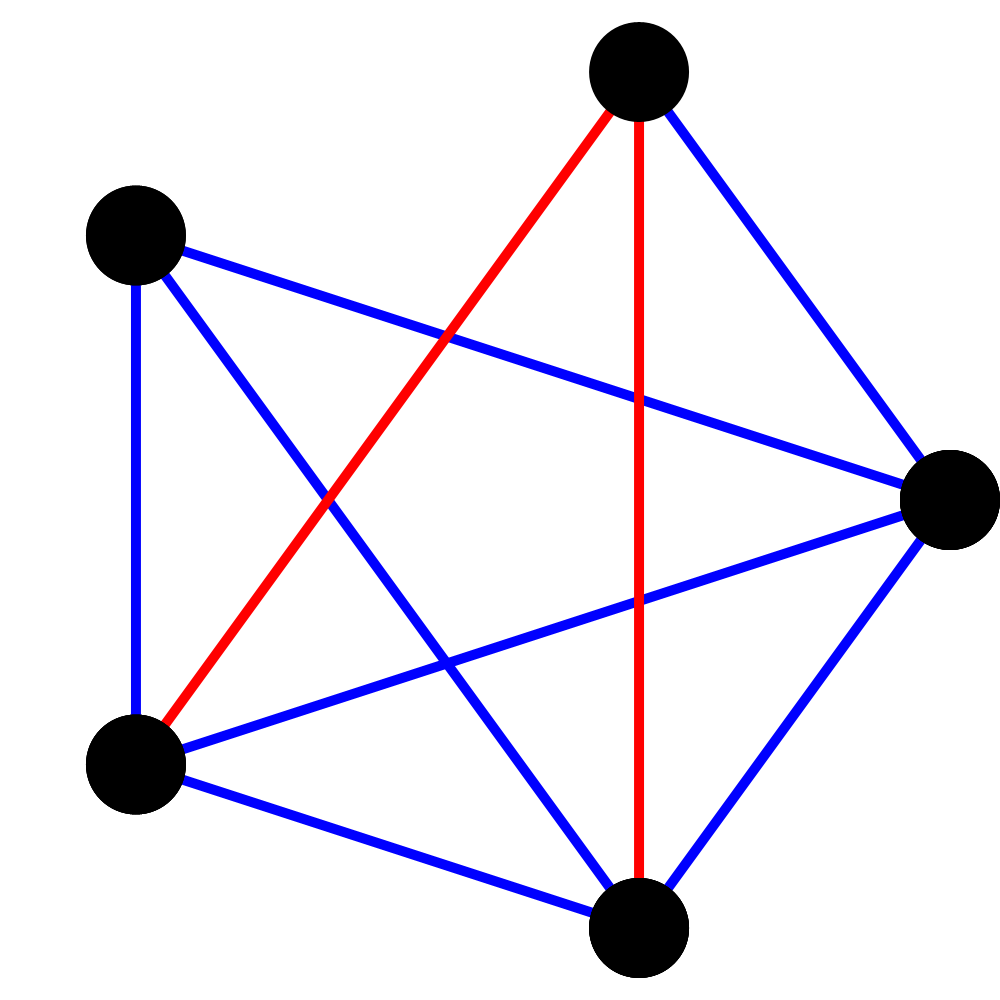} & 
\includegraphics[width=0.06\textwidth]{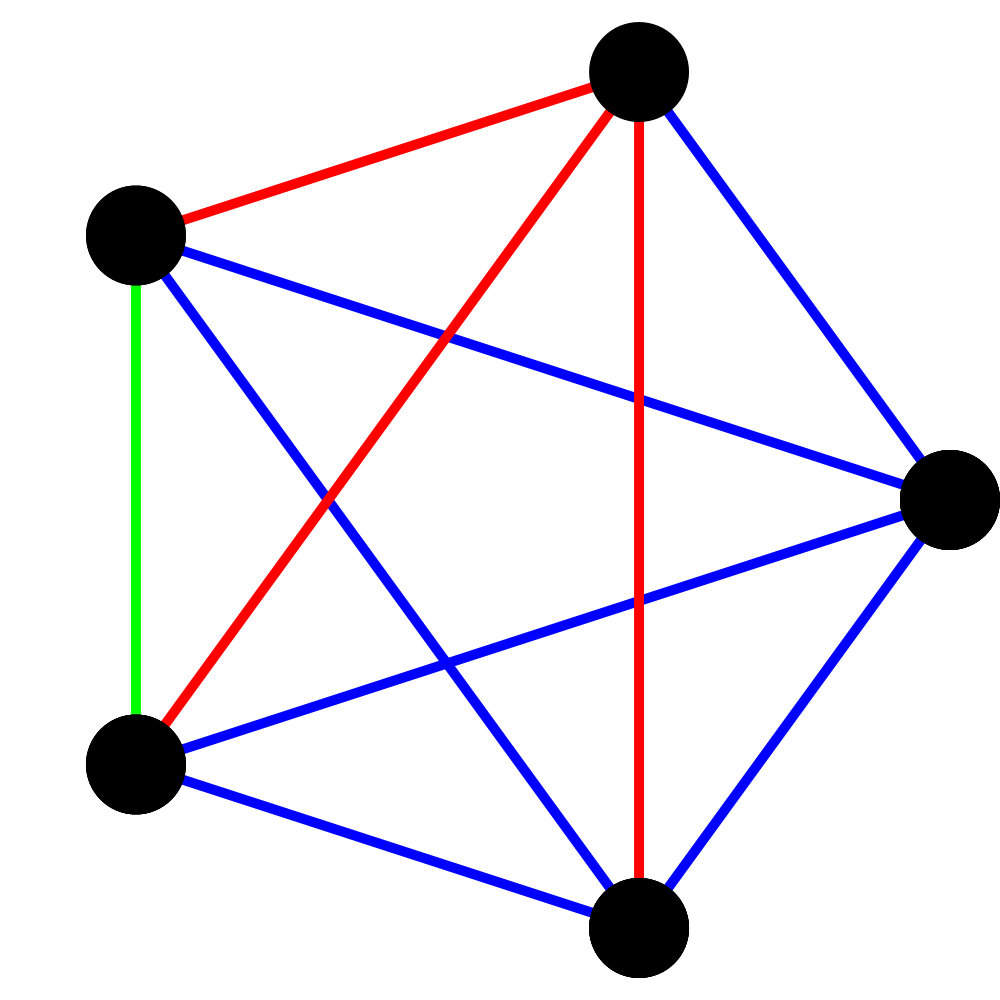} &
\includegraphics[width=0.06\textwidth]{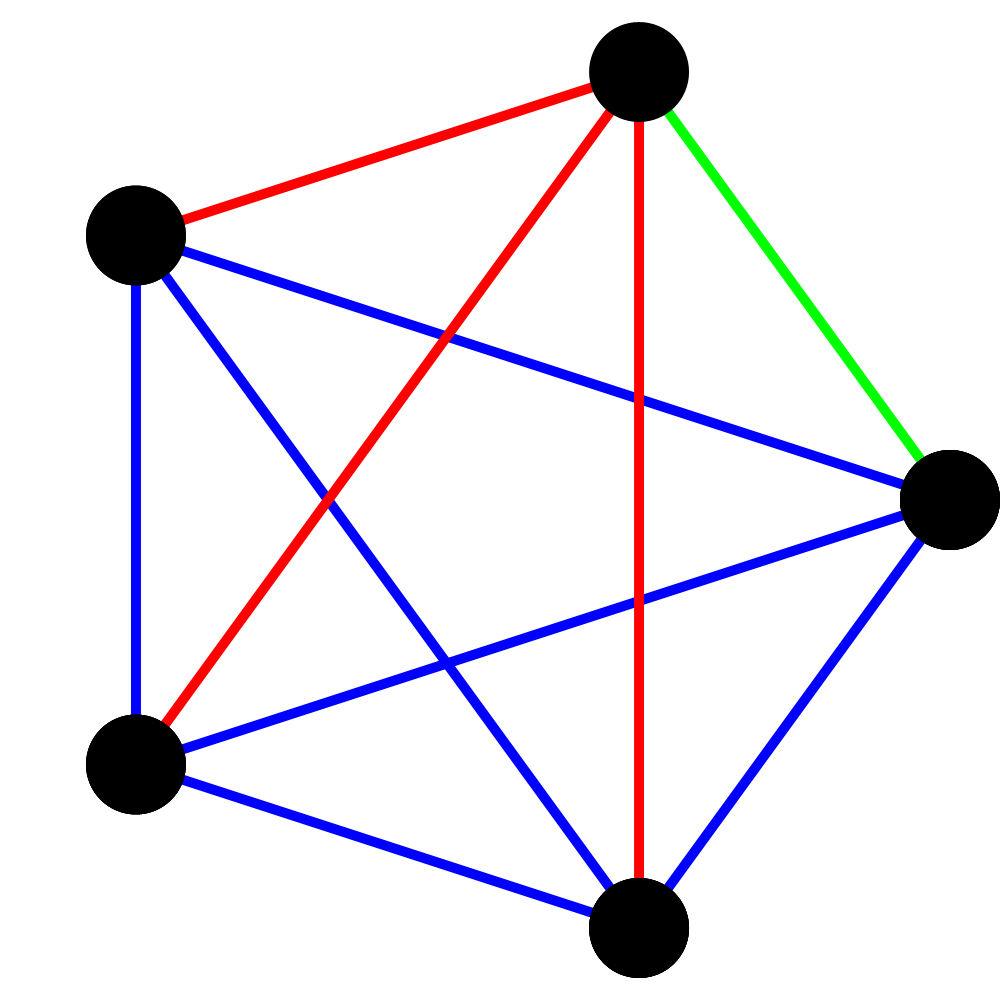} & 
\includegraphics[width=0.06\textwidth]{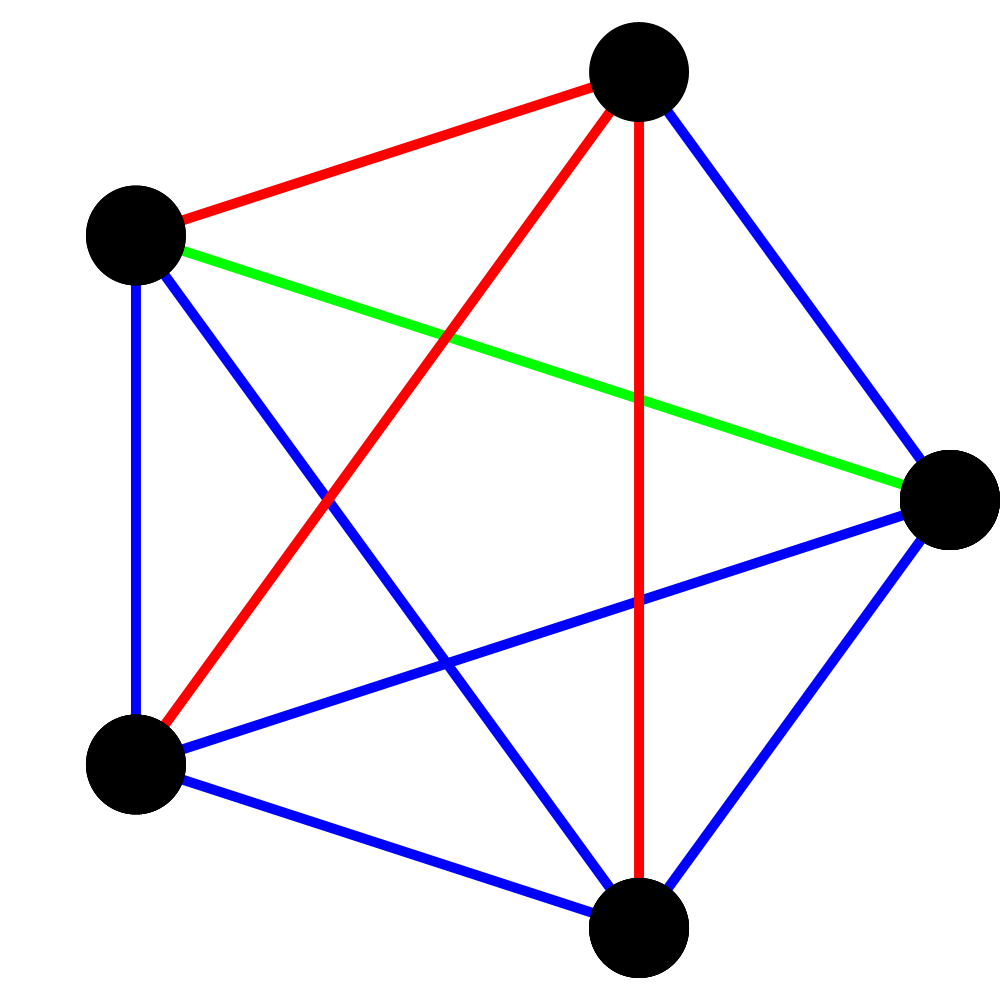} &
\includegraphics[width=0.06\textwidth]{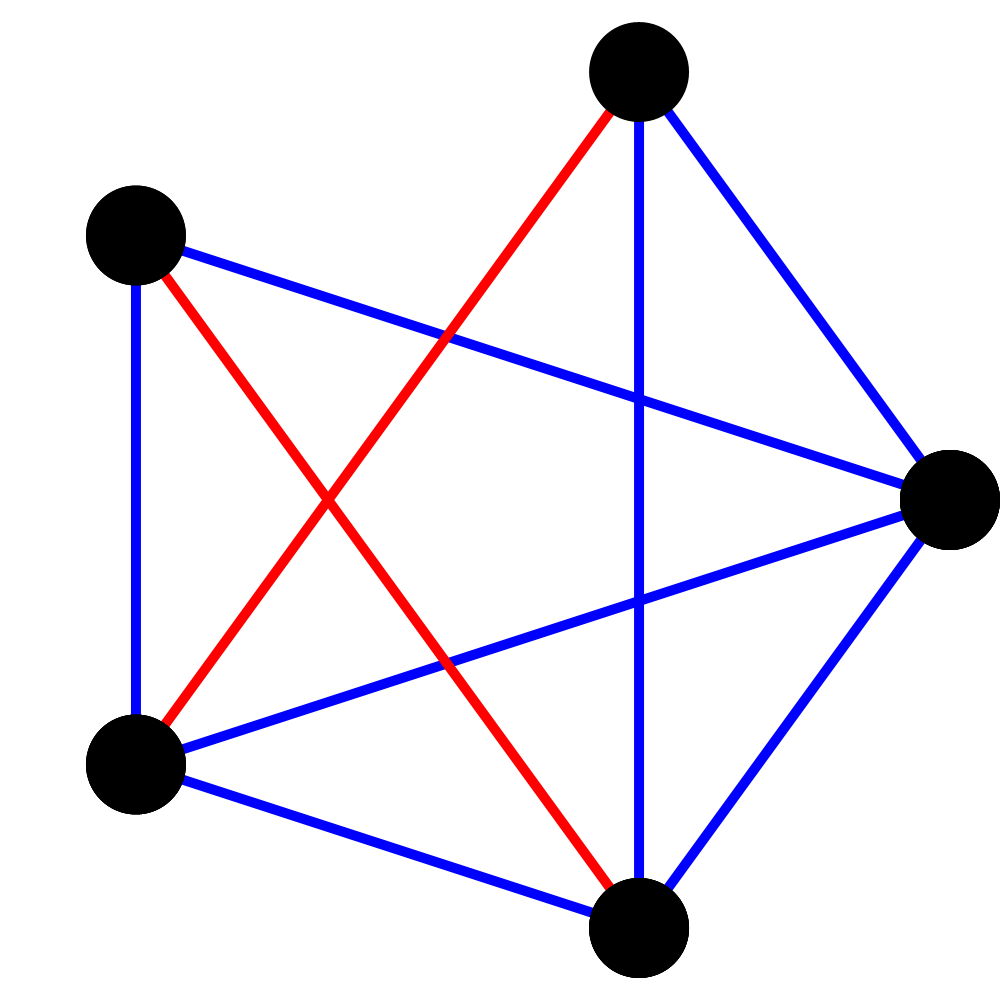} & \\
& & & & 19696 & 19696 & 19696 & 19696 & 19696 & 21696 & 21696 & 21696 & \\
& & & &
\includegraphics[width=0.06\textwidth]{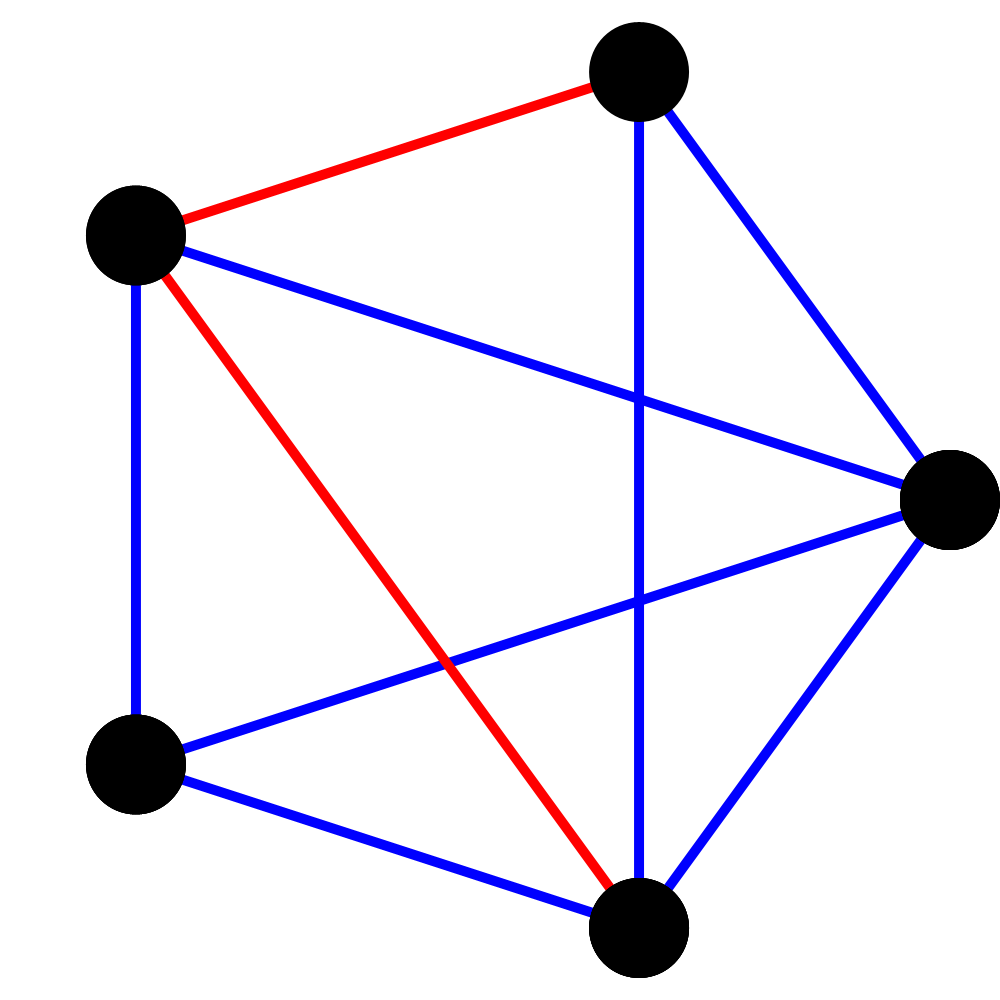} & 
\includegraphics[width=0.06\textwidth]{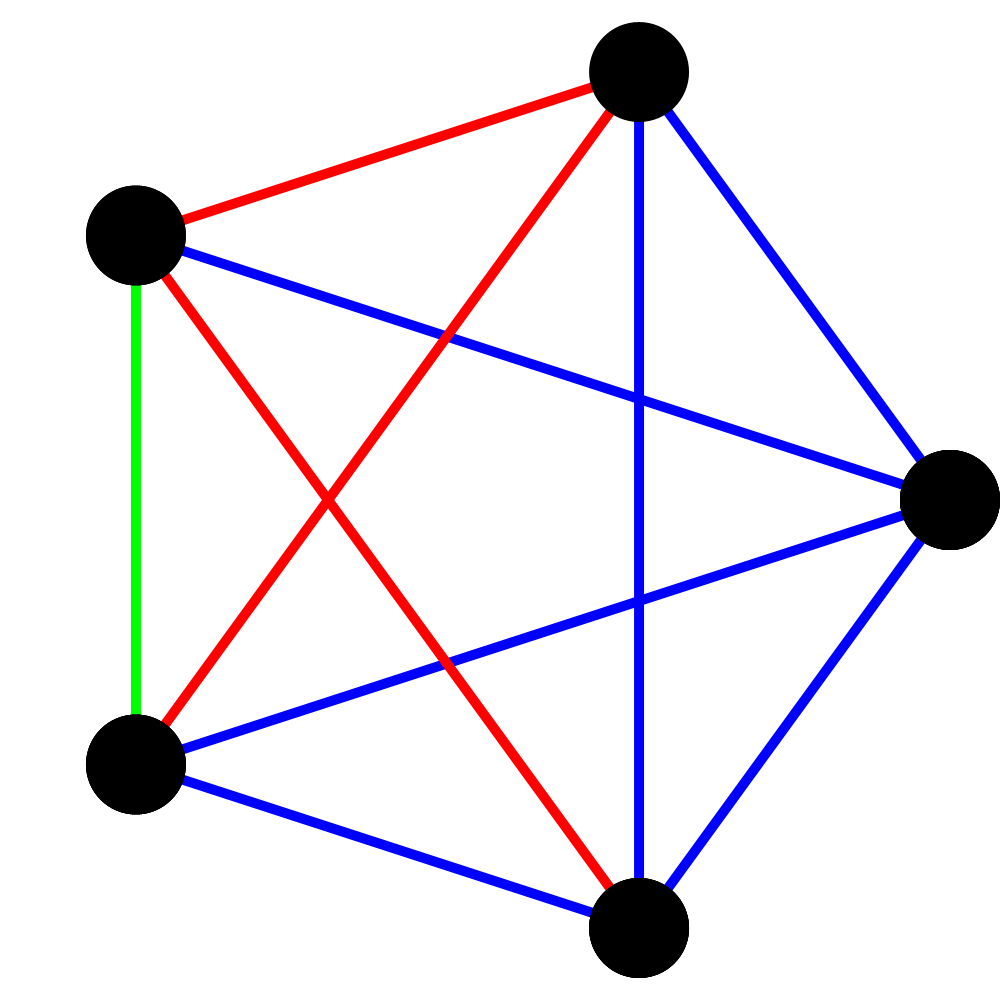} &
\includegraphics[width=0.06\textwidth]{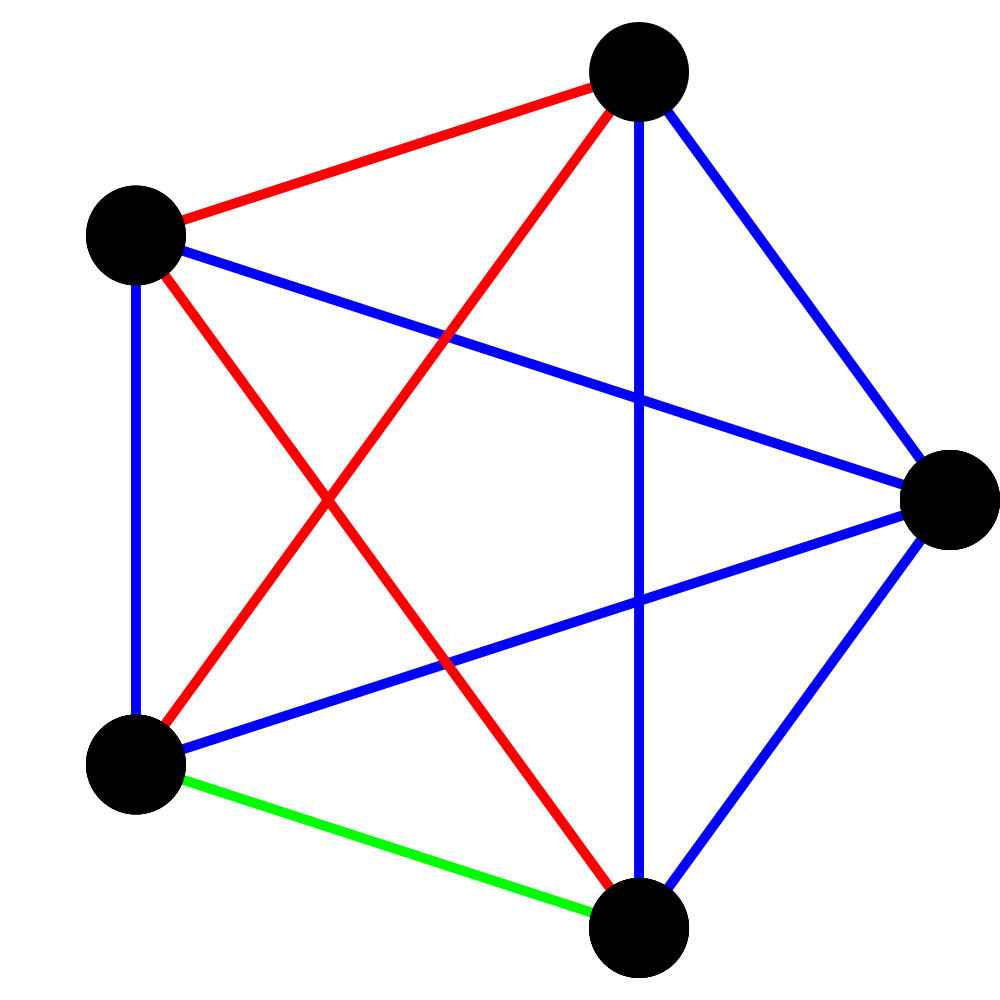} &
\includegraphics[width=0.06\textwidth]{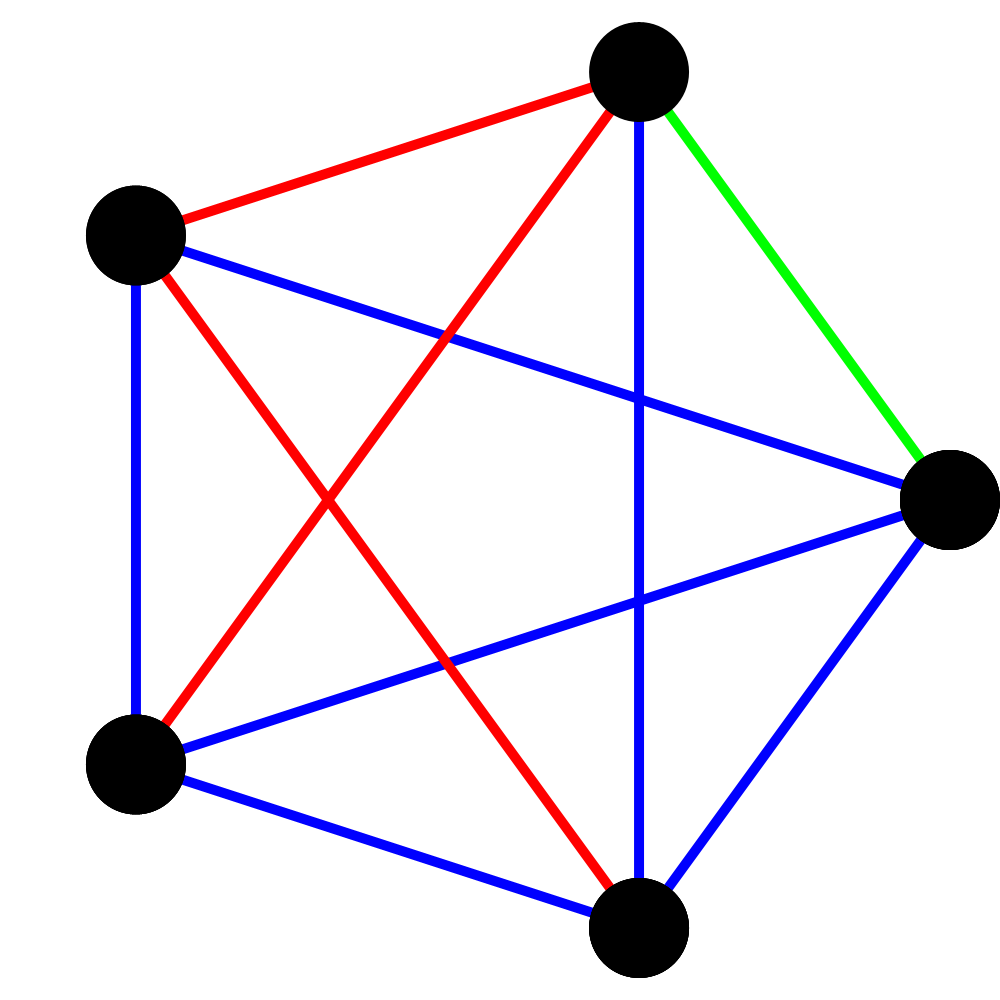} & 
\includegraphics[width=0.06\textwidth]{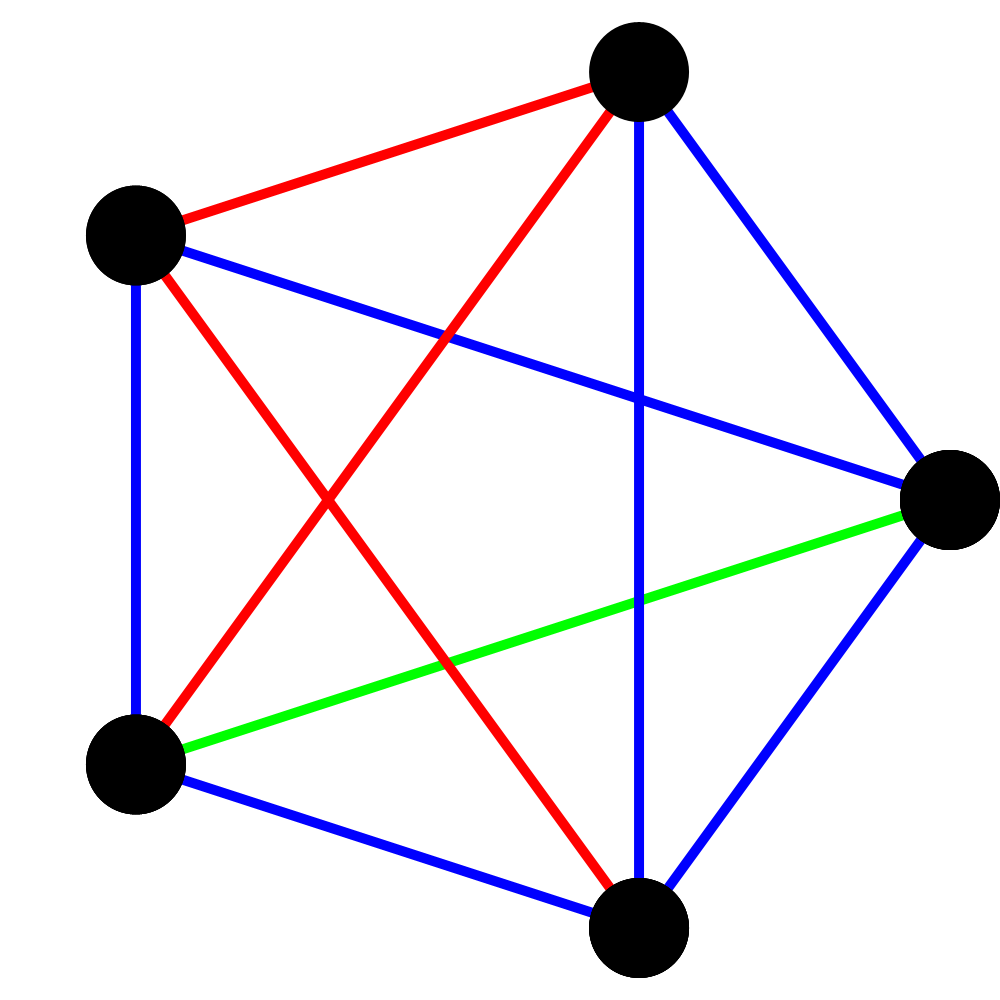} &
\includegraphics[width=0.06\textwidth]{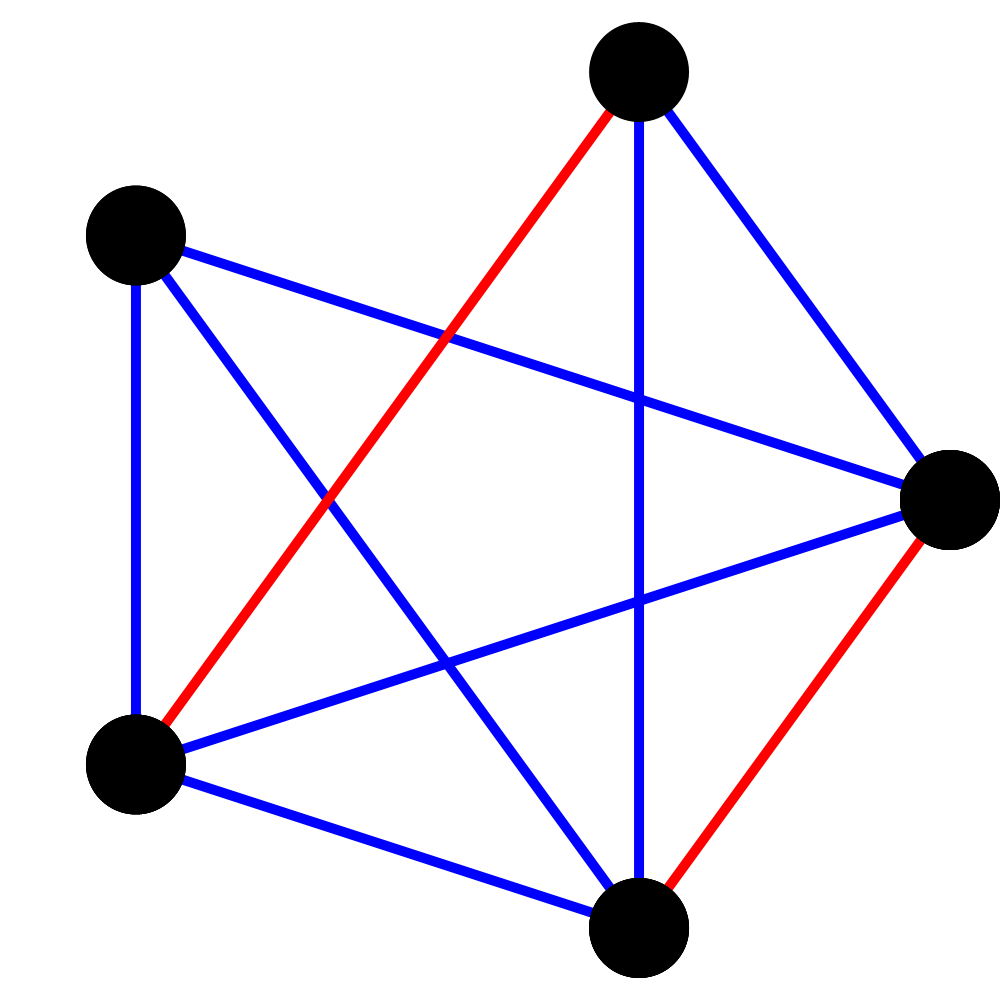} & 
\includegraphics[width=0.06\textwidth]{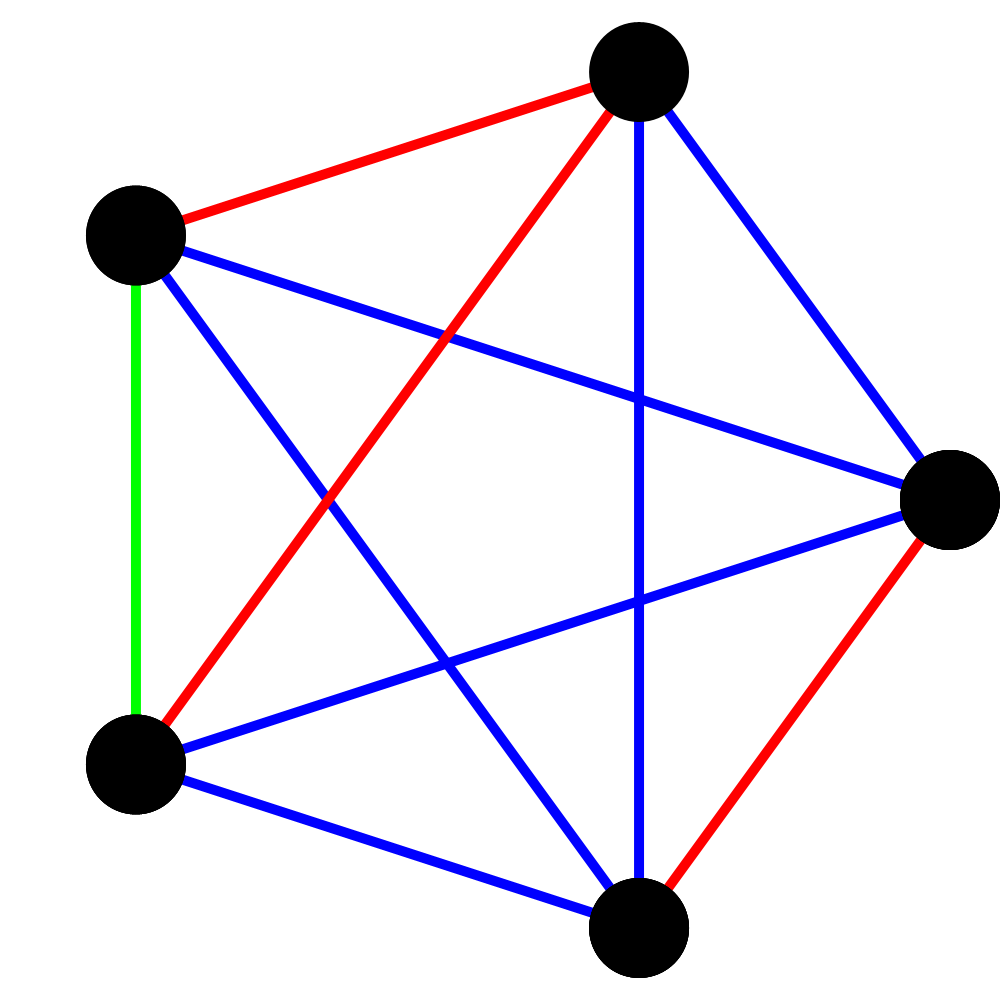} &
\includegraphics[width=0.06\textwidth]{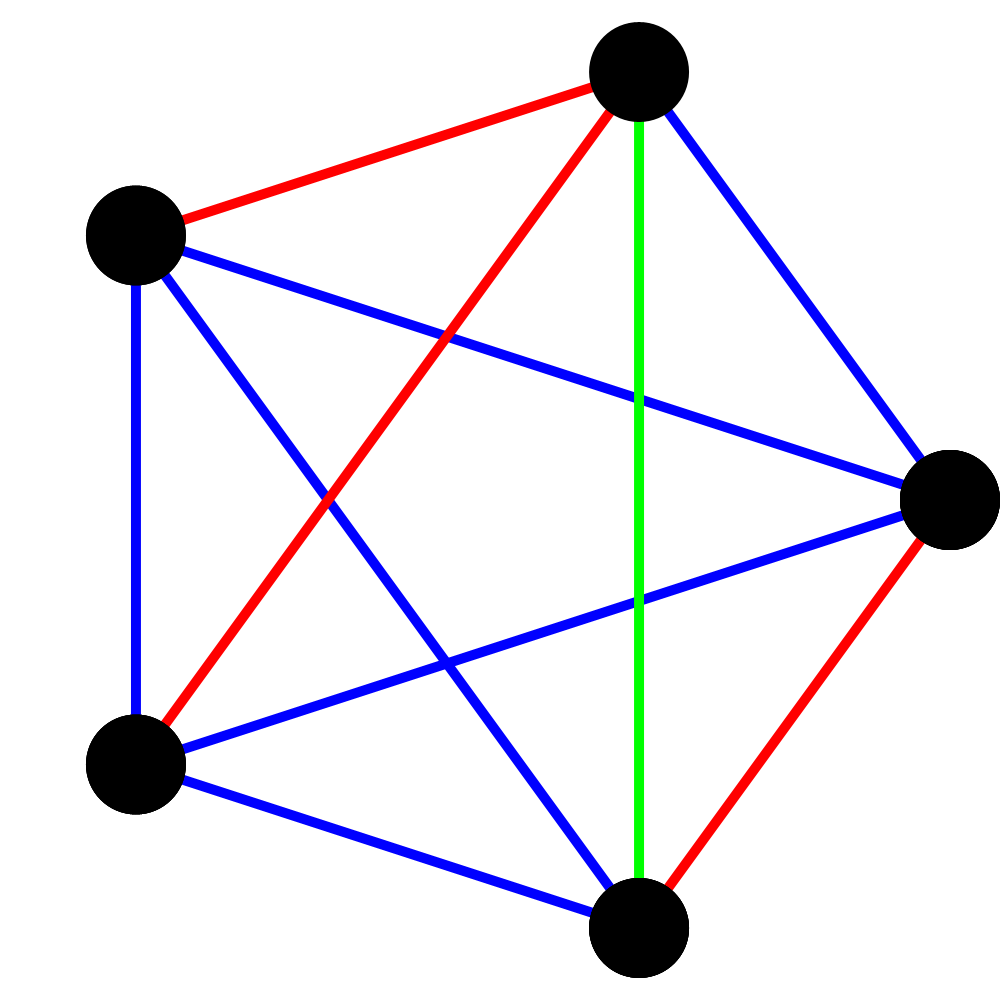} & \\
& & & & 21696 & 21696 & 16356 & 28640 & 16948 & 29888 & 74056 & 76832 & \\
& & & &
\includegraphics[width=0.06\textwidth]{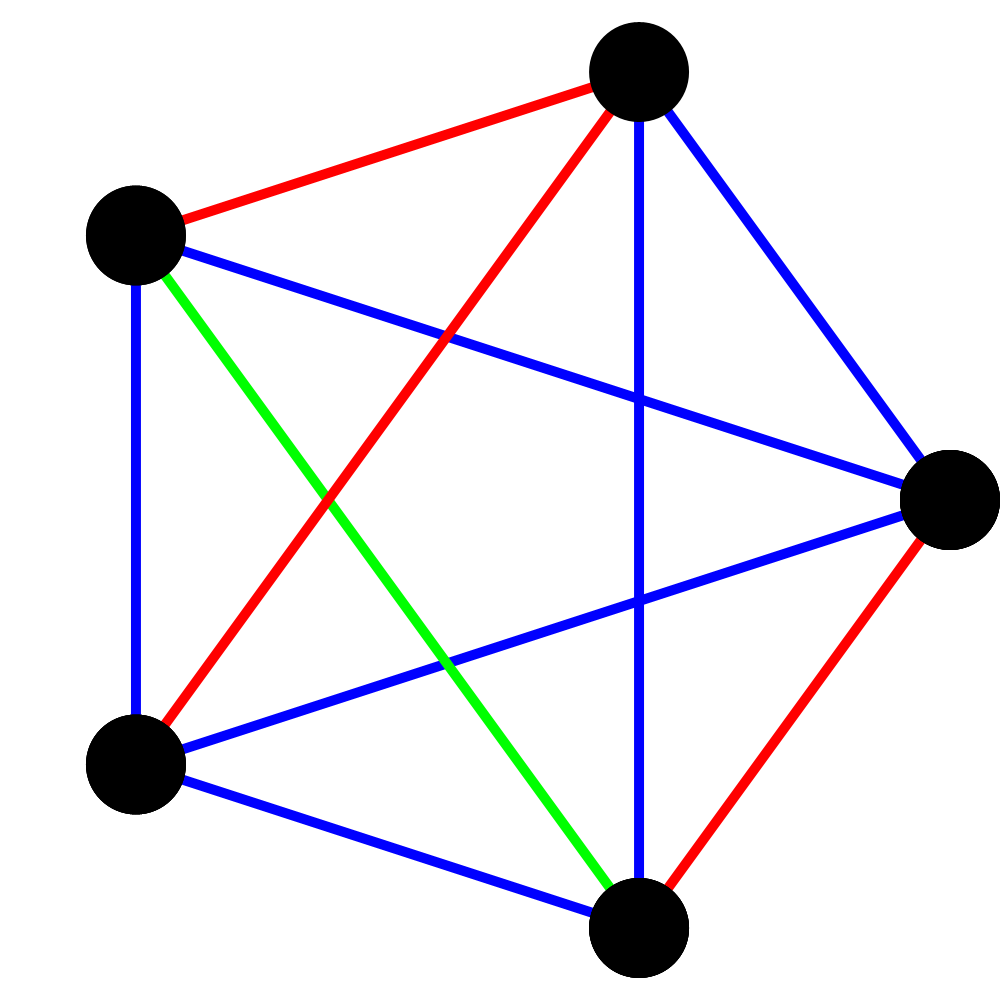} & 
\includegraphics[width=0.06\textwidth]{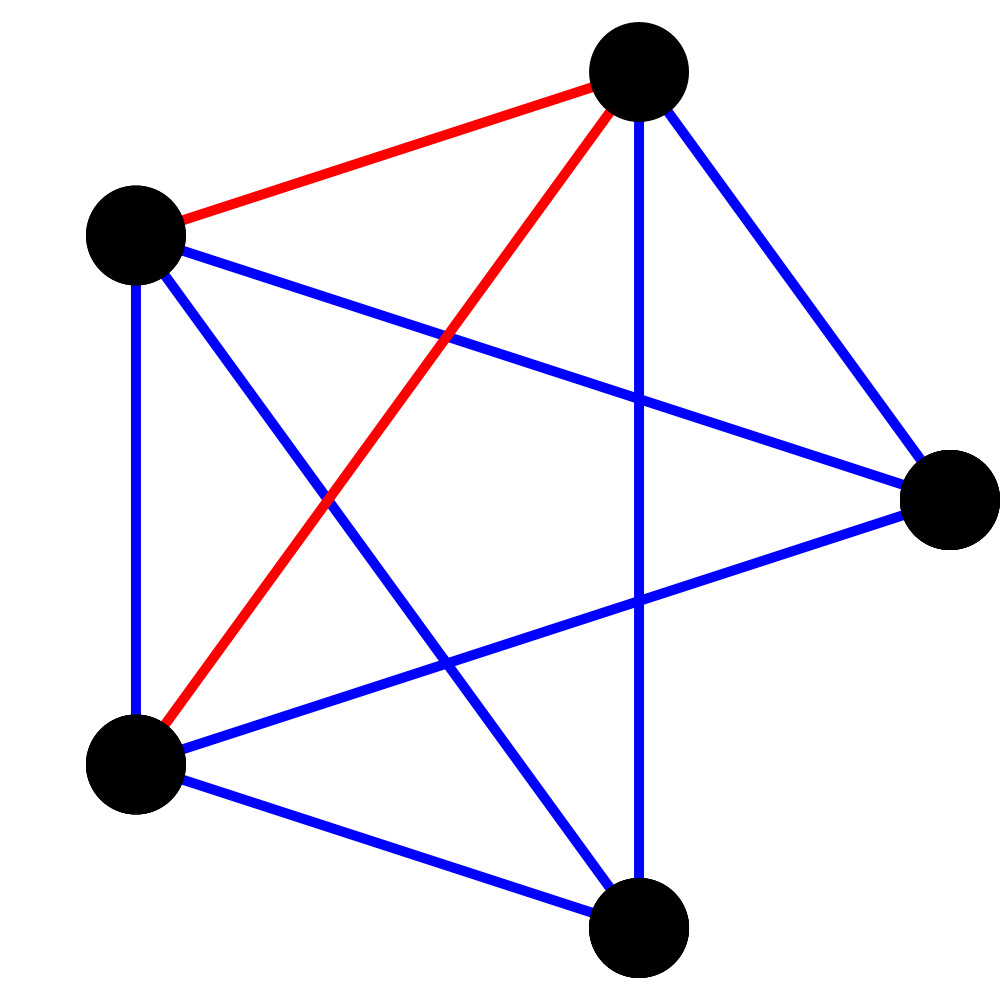} &
\includegraphics[width=0.06\textwidth]{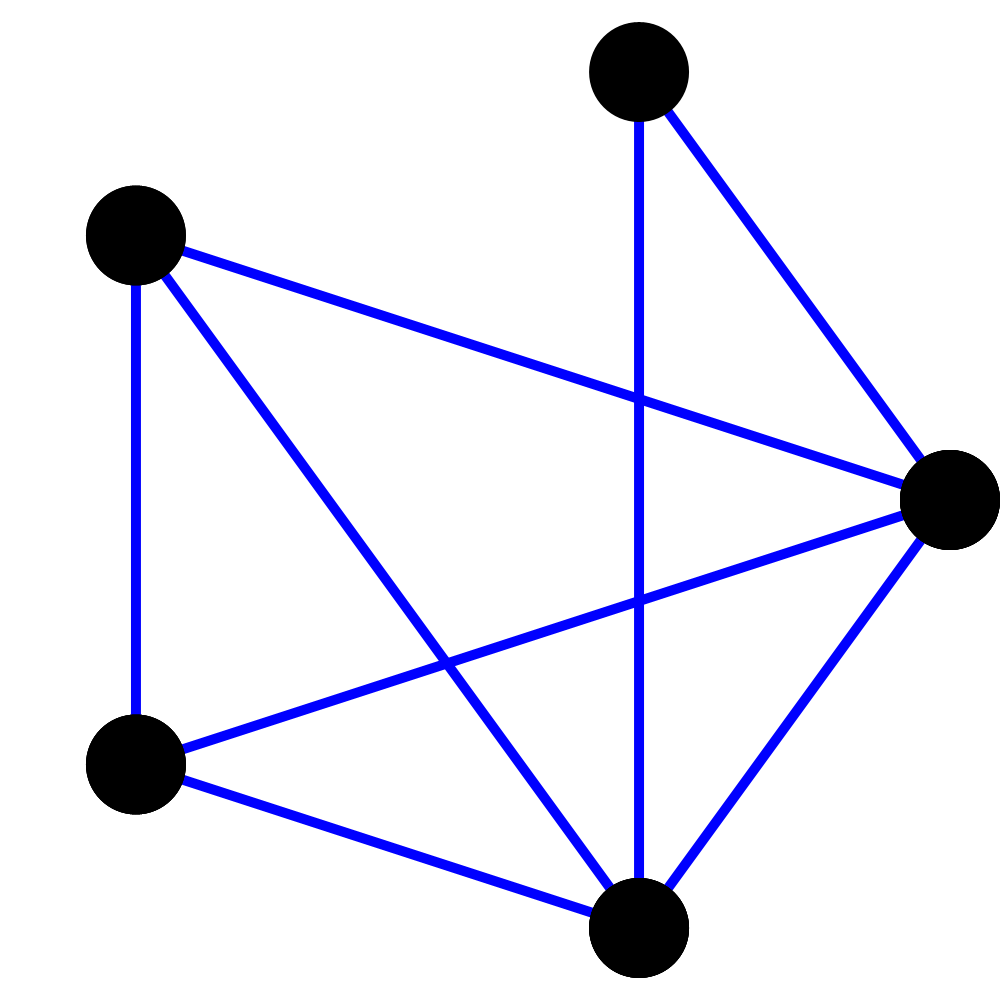} &
\includegraphics[width=0.06\textwidth]{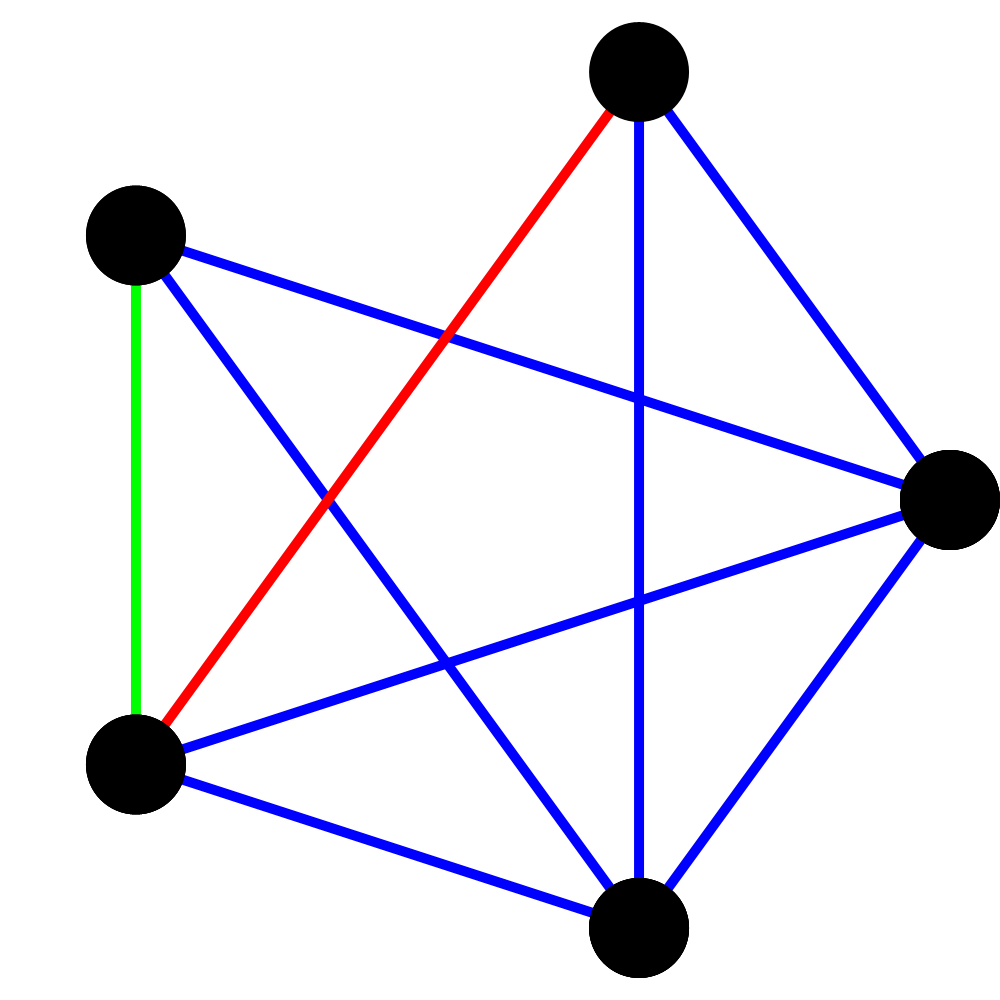} & 
\includegraphics[width=0.06\textwidth]{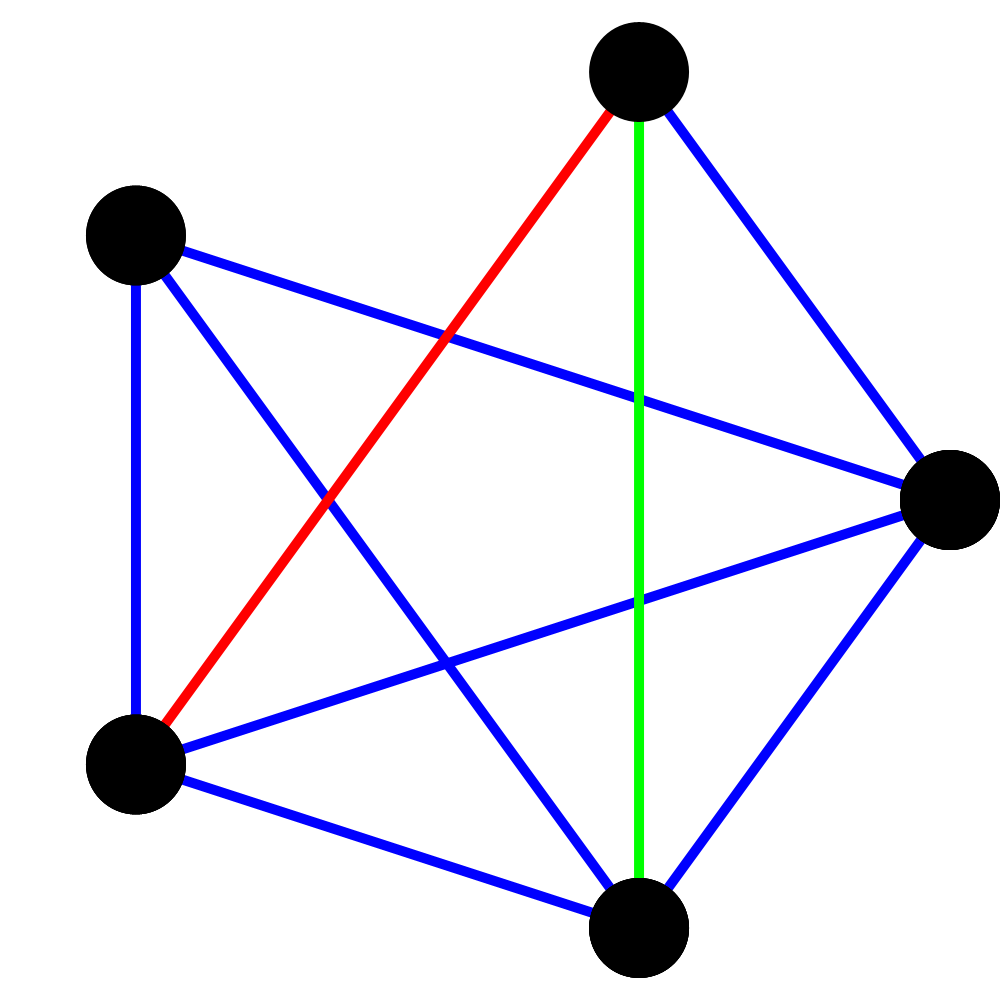} &
\includegraphics[width=0.06\textwidth]{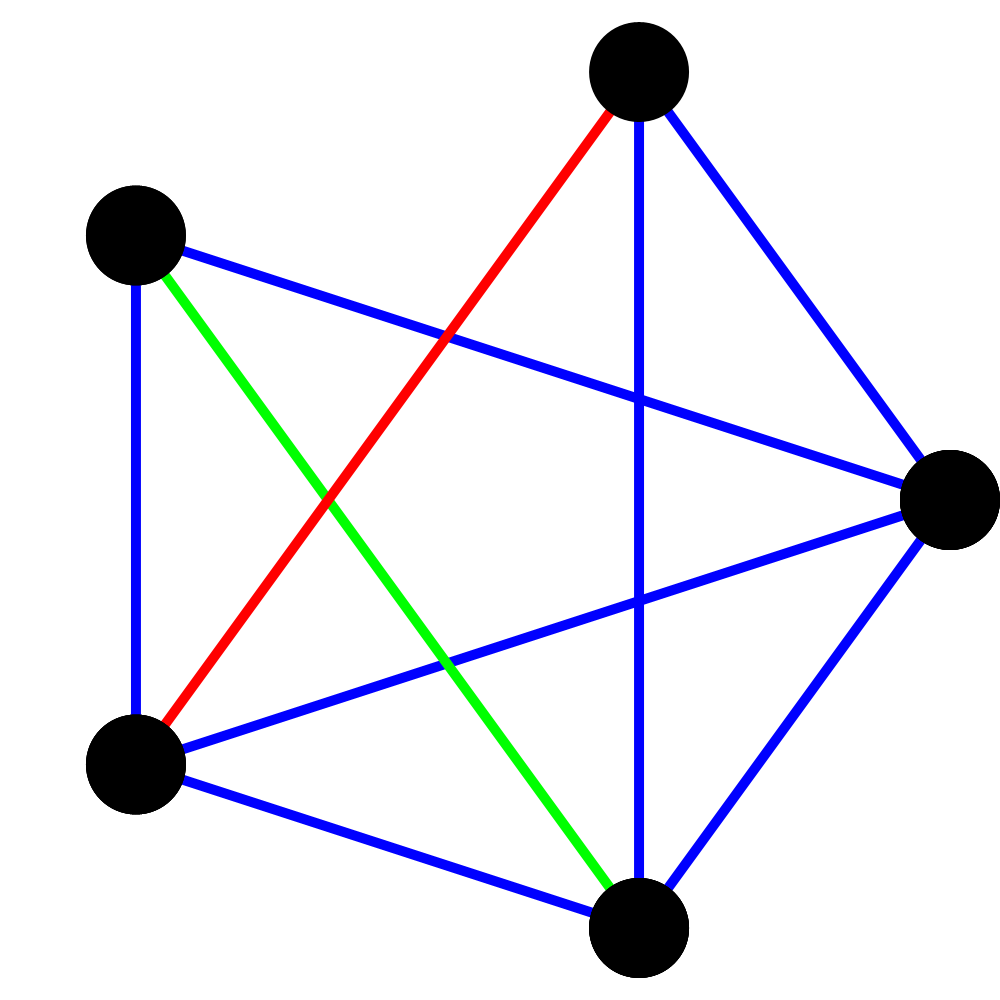} & 
\includegraphics[width=0.06\textwidth]{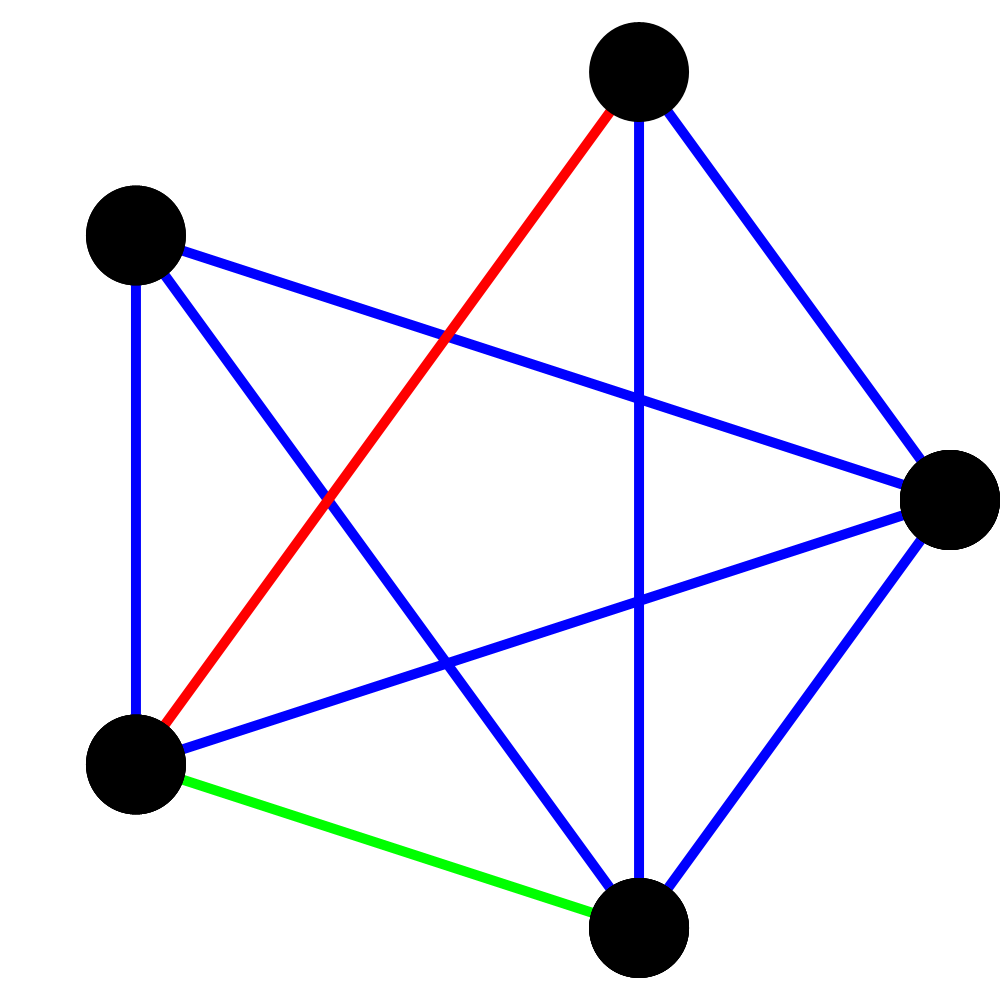} &
\includegraphics[width=0.06\textwidth]{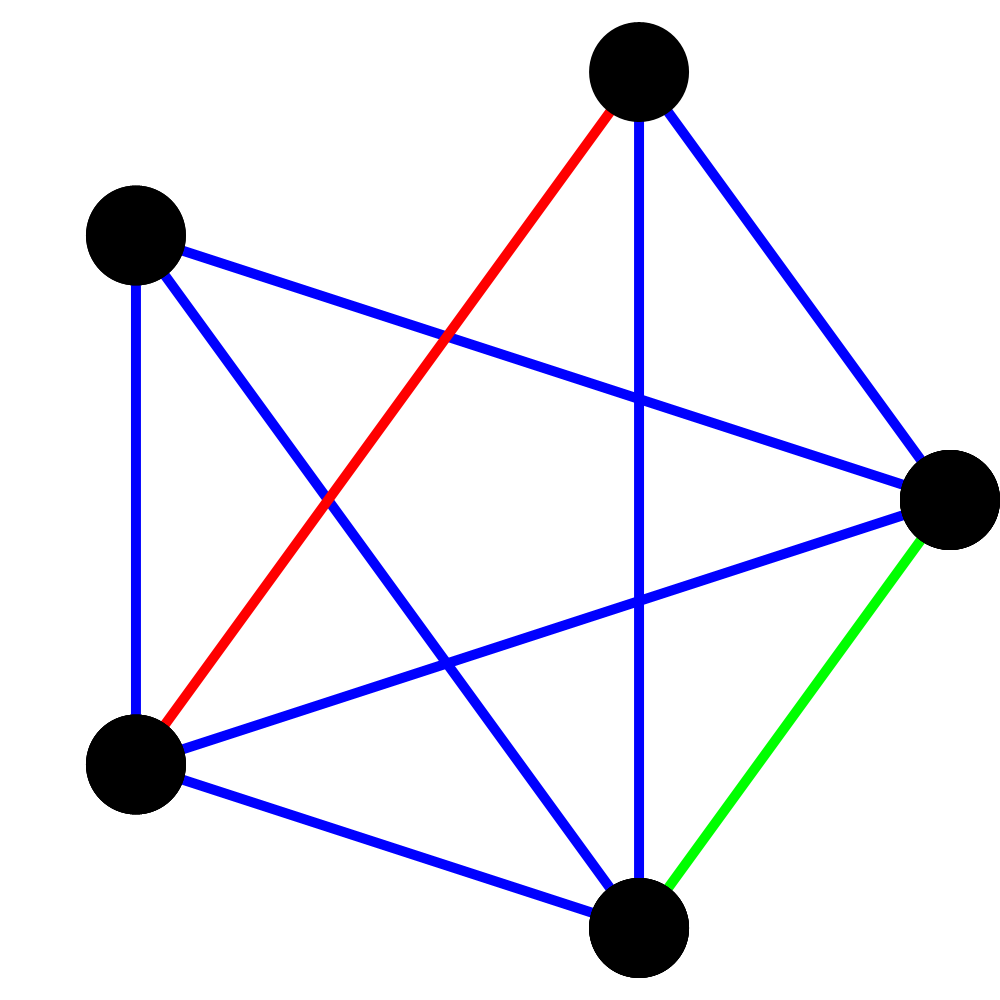} & \\
& & & & 74480 & 31183 & 87328 & 17364 & 77816 & 31964 & 33262 & 88000 & \\
& & & &
\includegraphics[width=0.06\textwidth]{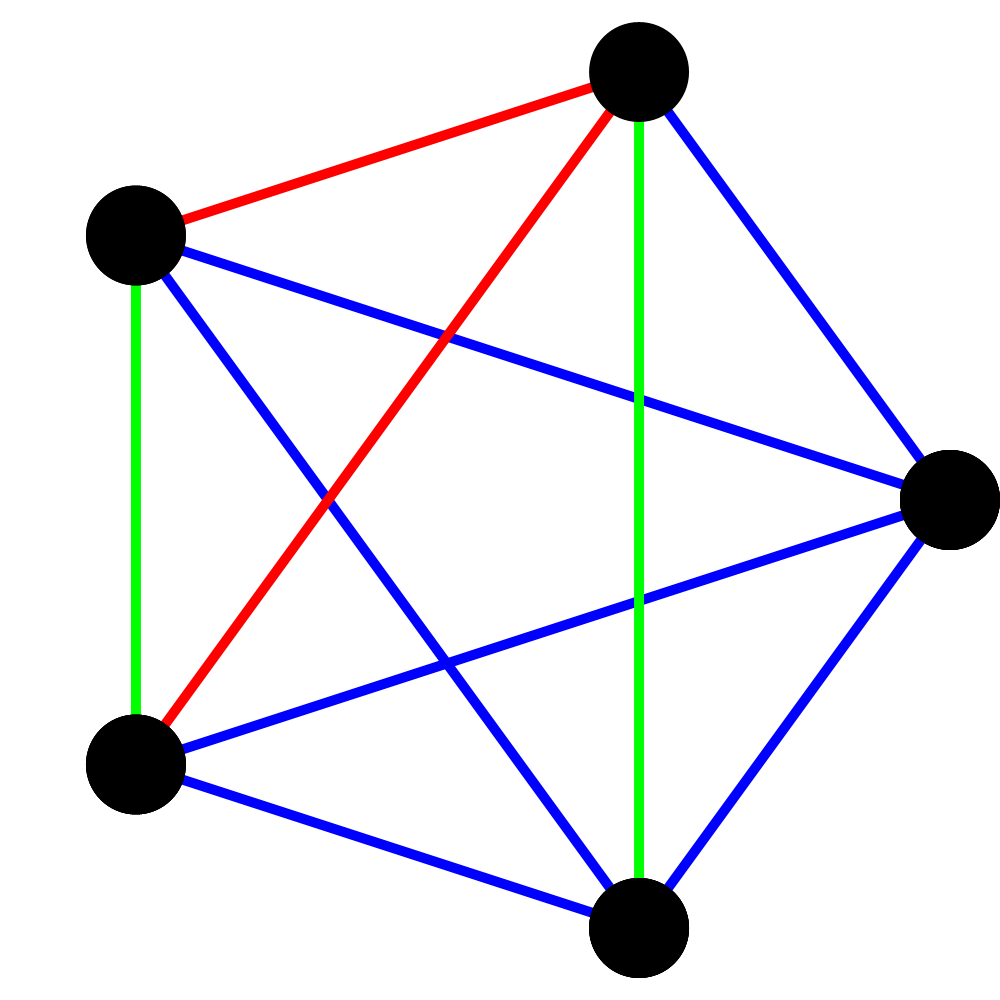} & 
\includegraphics[width=0.06\textwidth]{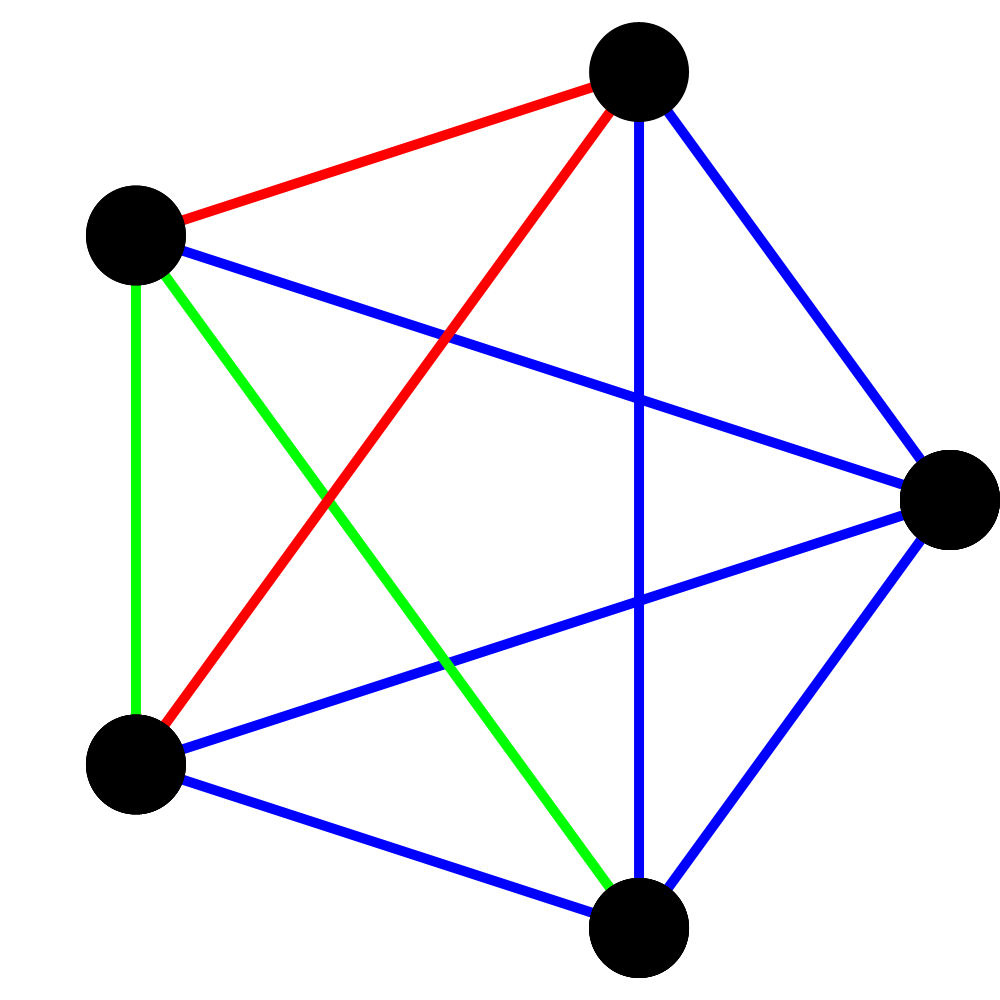} &
\includegraphics[width=0.06\textwidth]{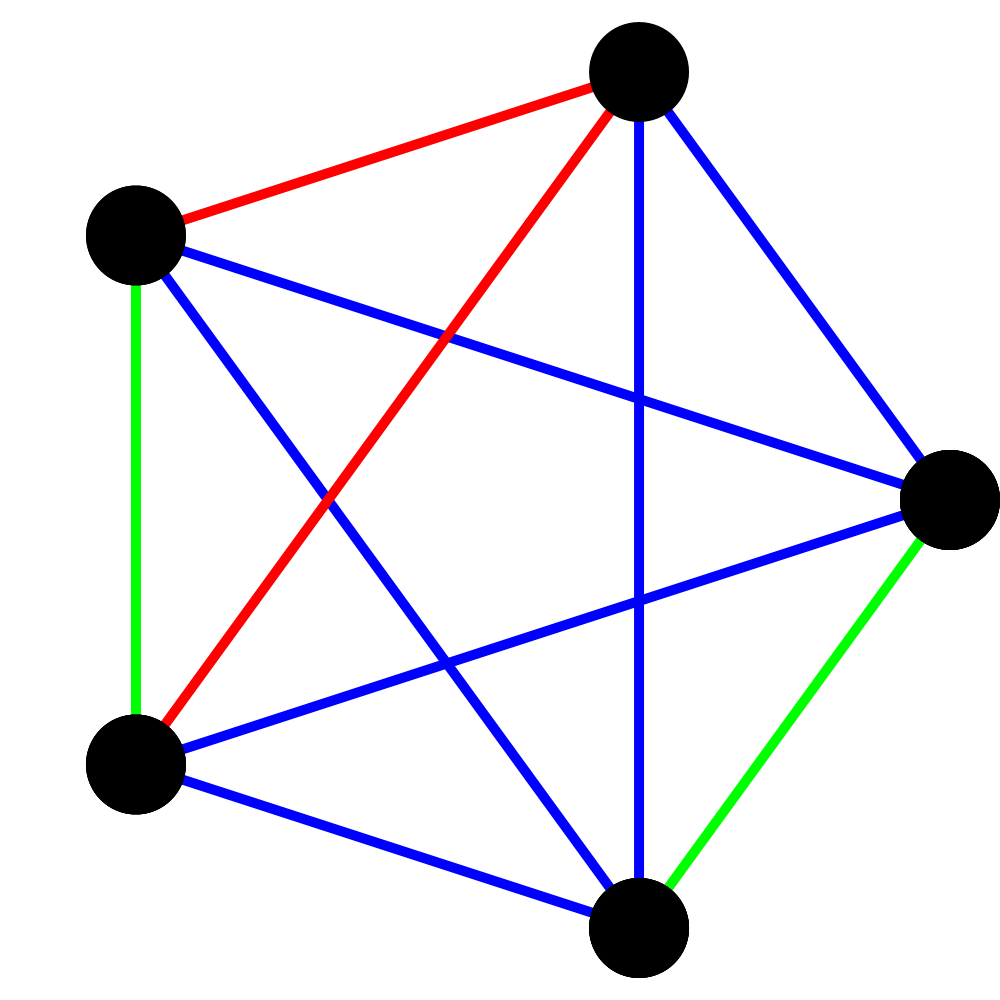} &
\includegraphics[width=0.06\textwidth]{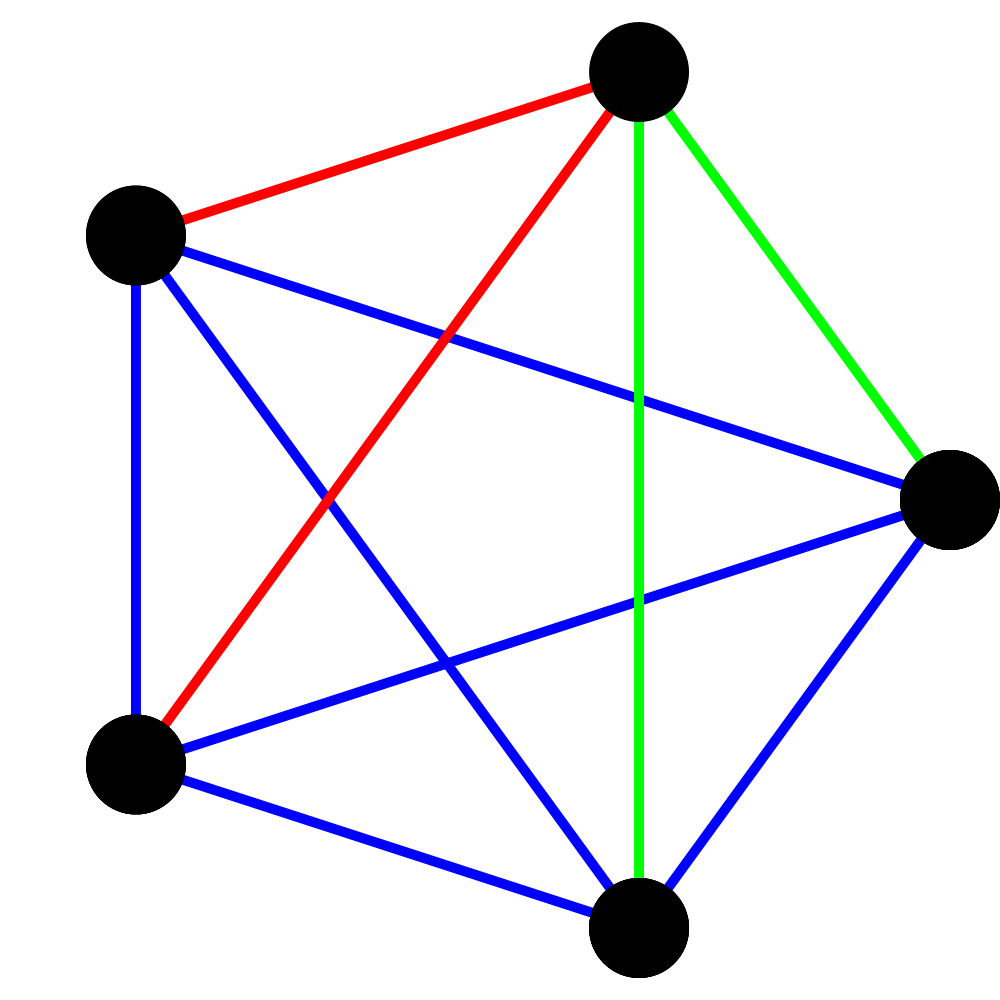} & 
\includegraphics[width=0.06\textwidth]{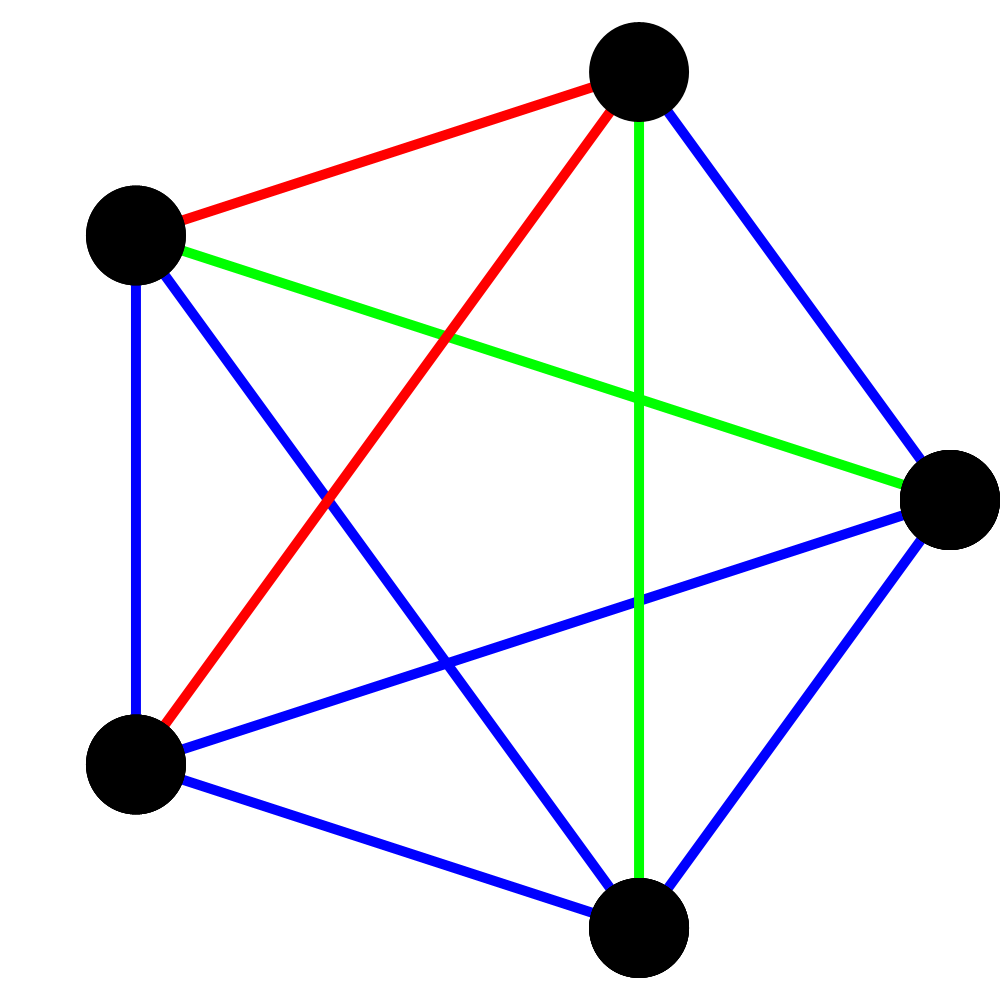} &
\includegraphics[width=0.06\textwidth]{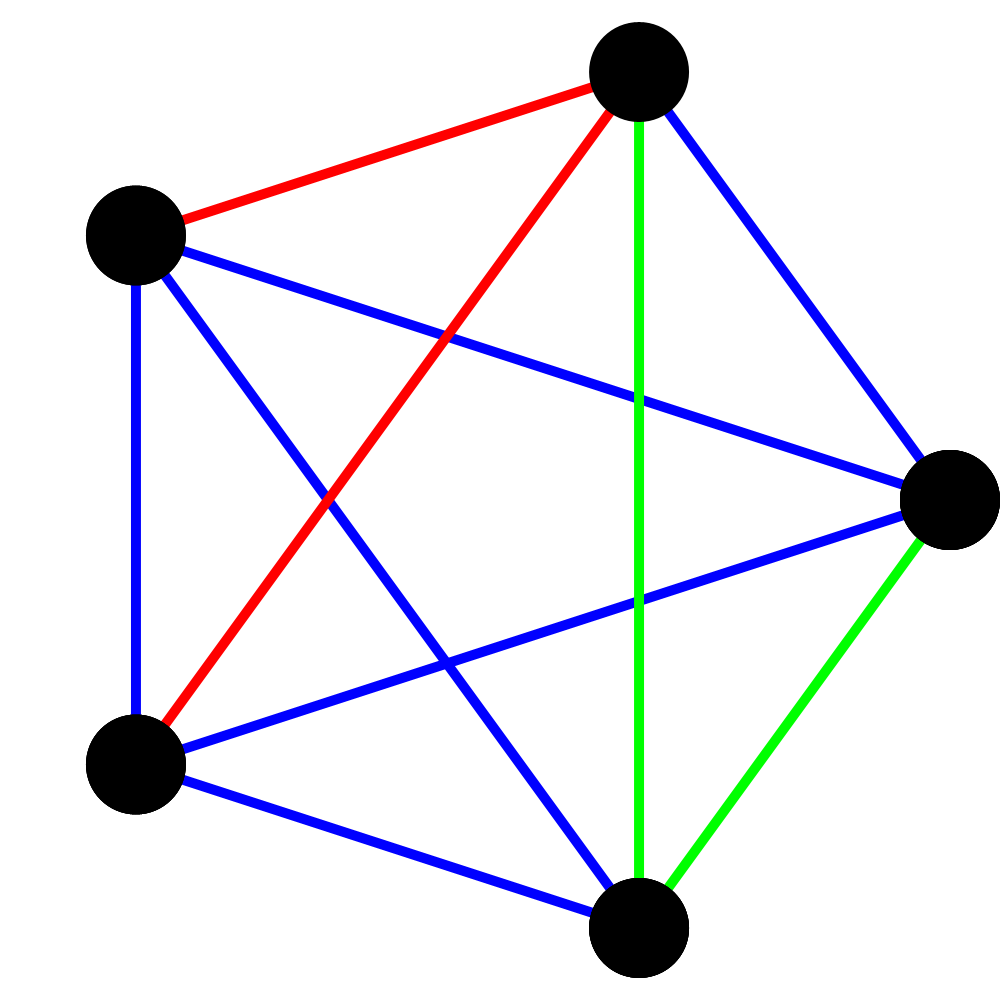} & 
\includegraphics[width=0.06\textwidth]{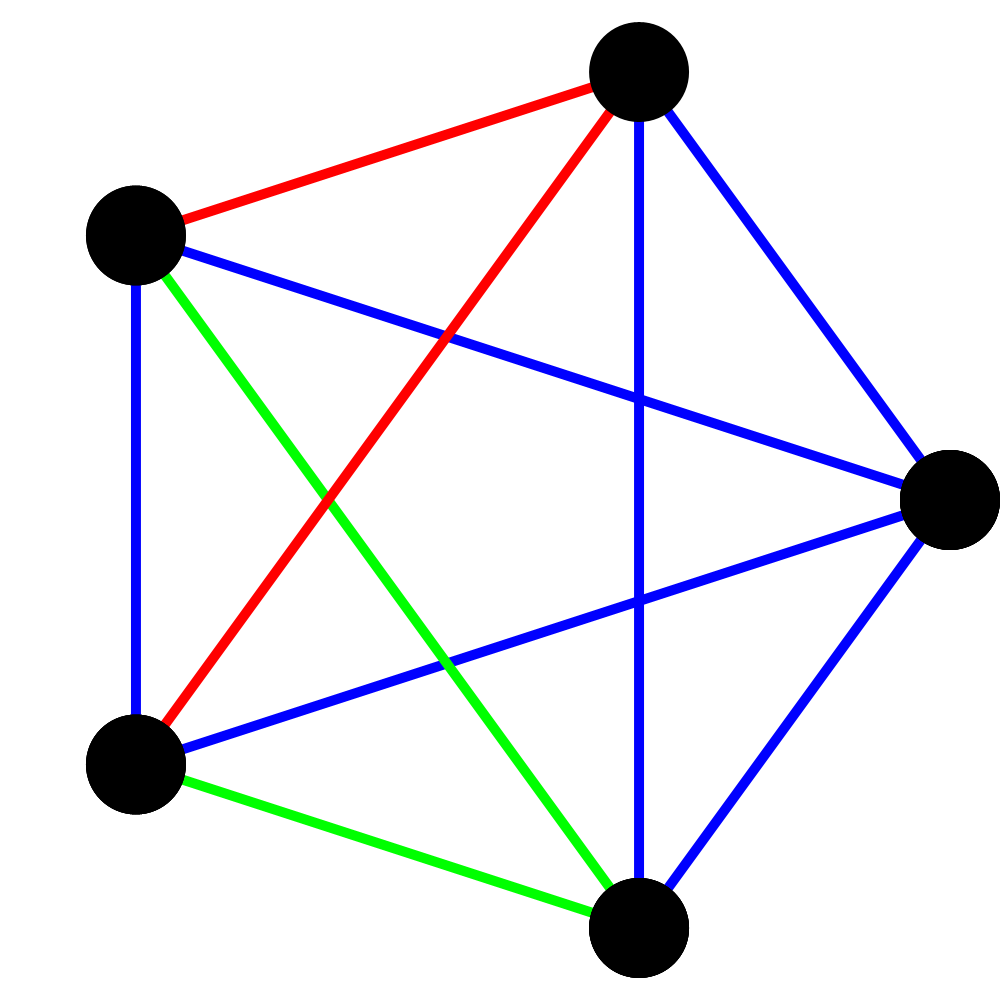} &
\includegraphics[width=0.06\textwidth]{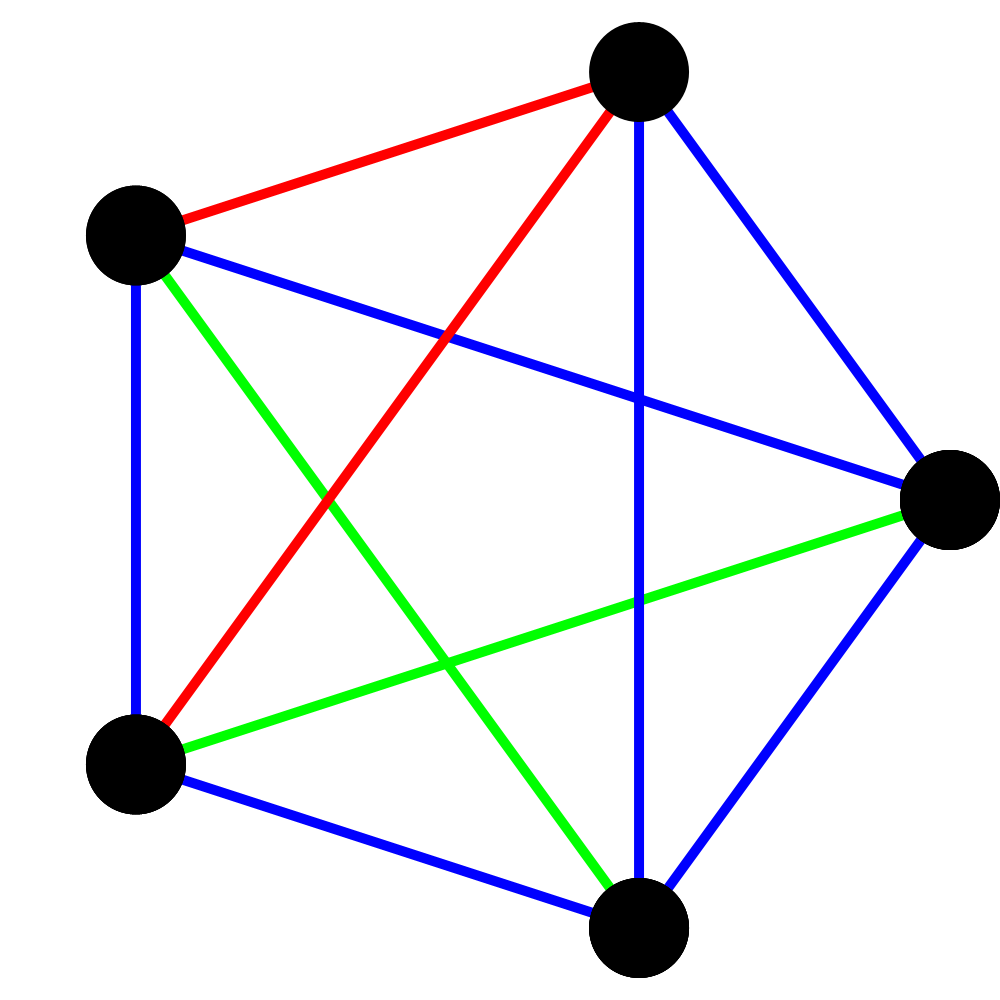} & \\
& & & & 33884 & 171696 & 198032 & 193648 & 207664 & & & & \\
& & & &
\includegraphics[width=0.06\textwidth]{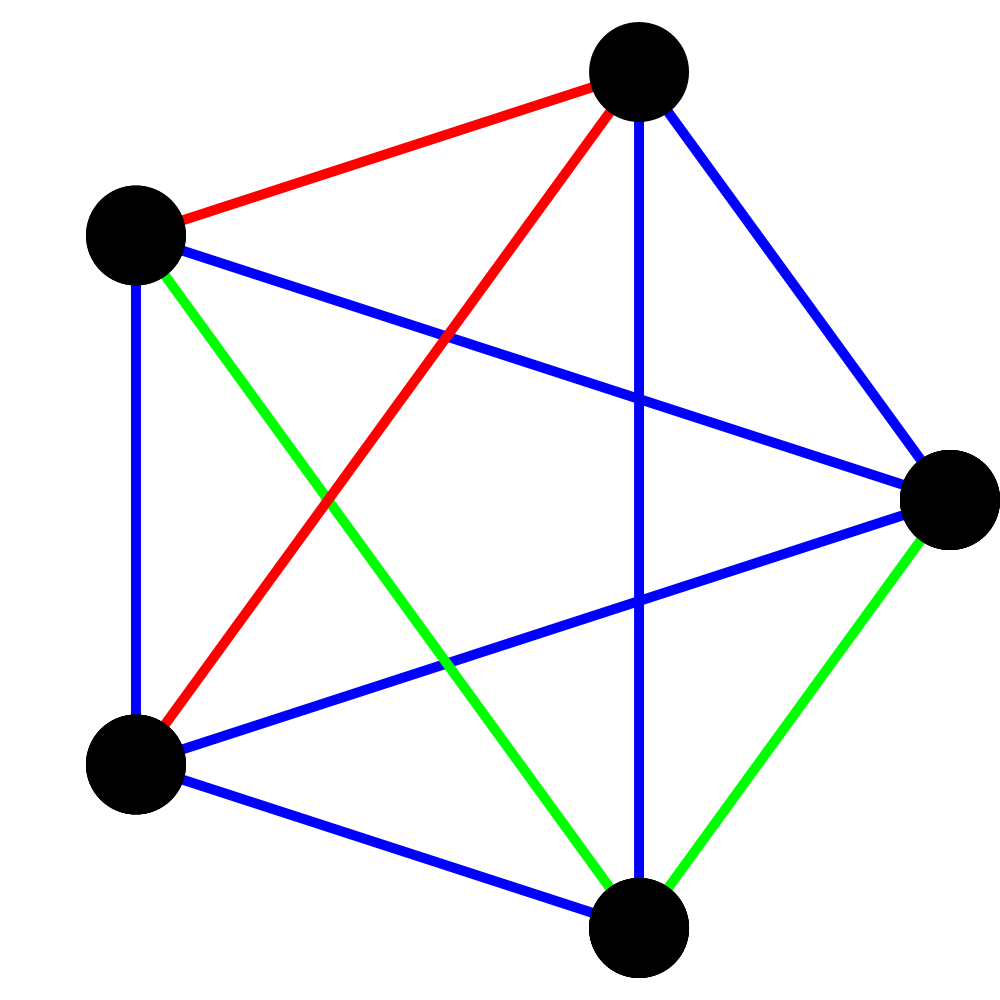} & 
\includegraphics[width=0.06\textwidth]{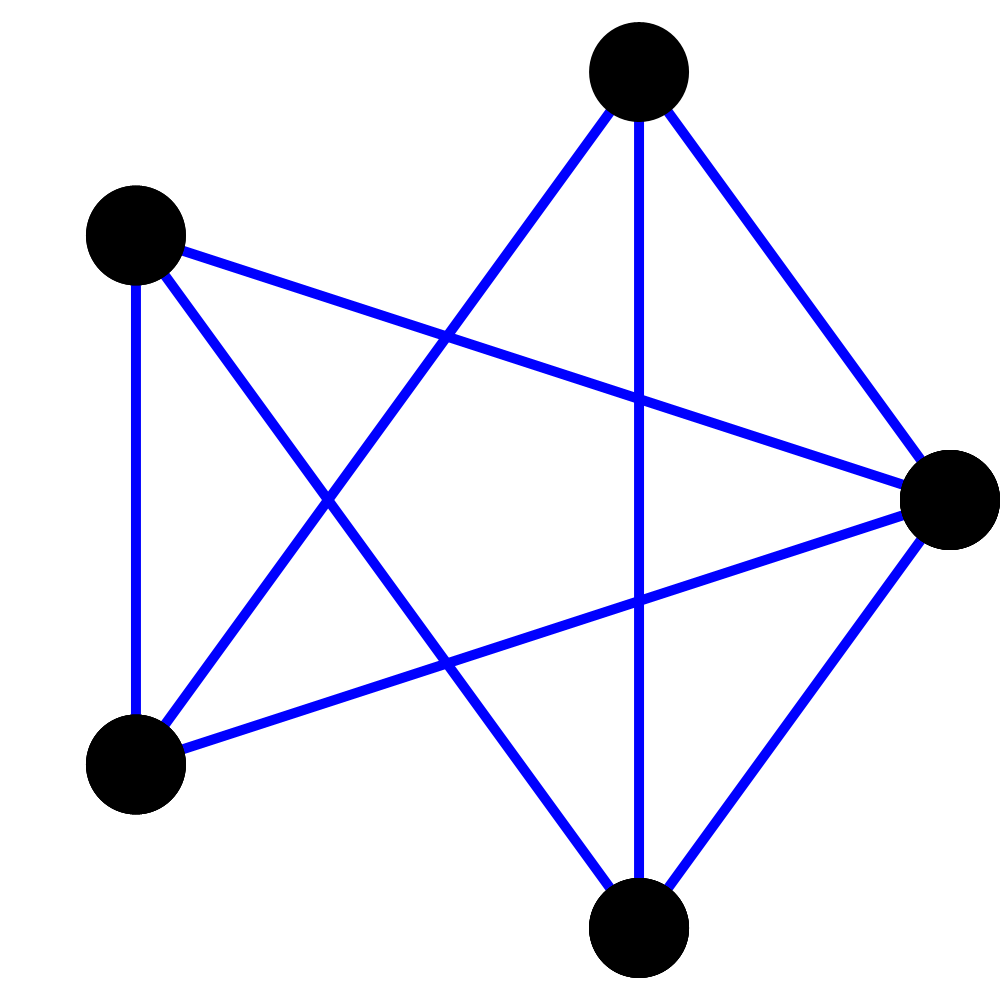} &
\includegraphics[width=0.06\textwidth]{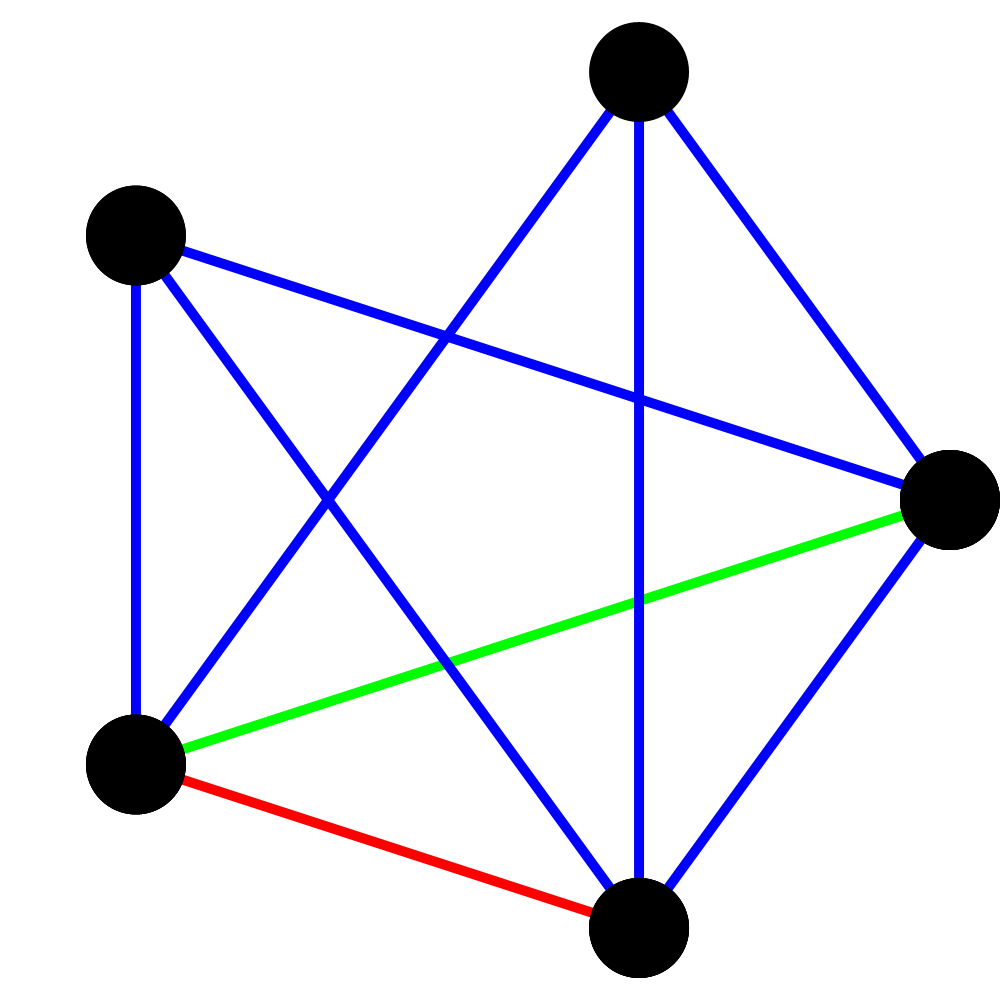} &
\includegraphics[width=0.06\textwidth]{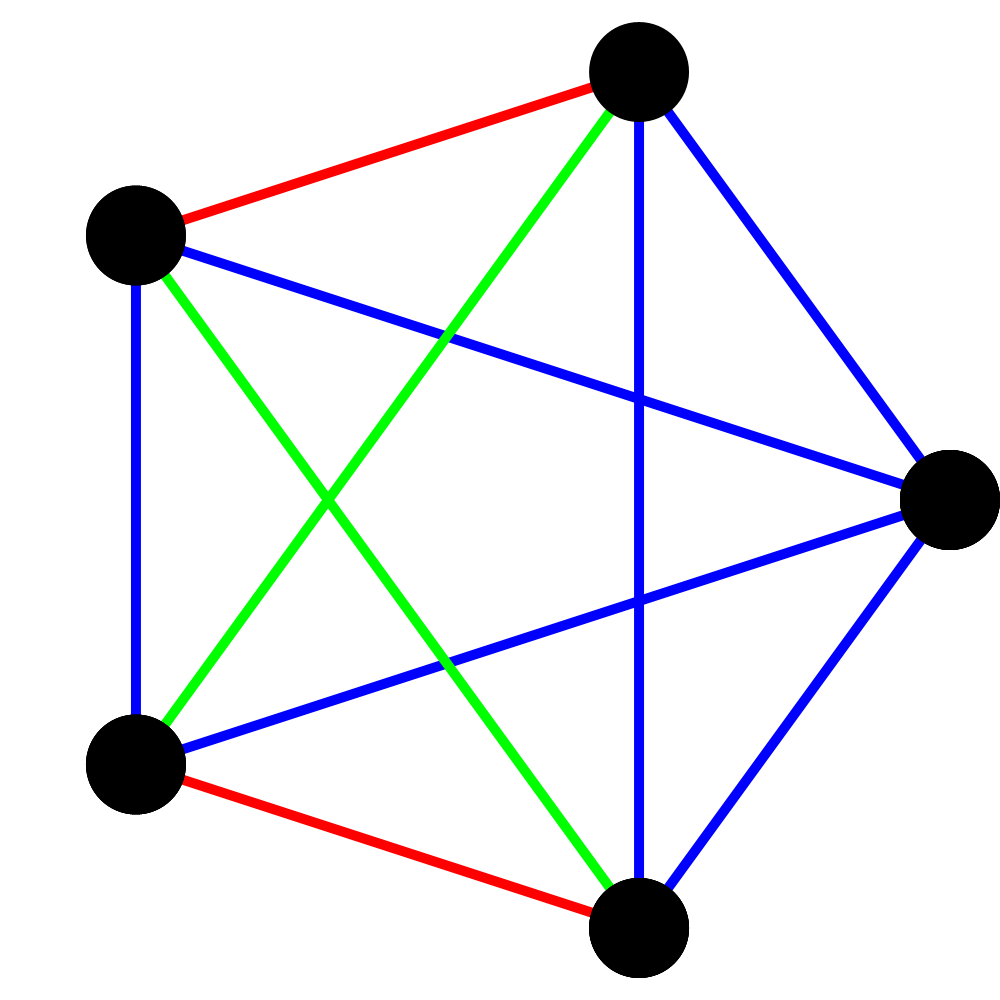} & 
\includegraphics[width=0.06\textwidth]{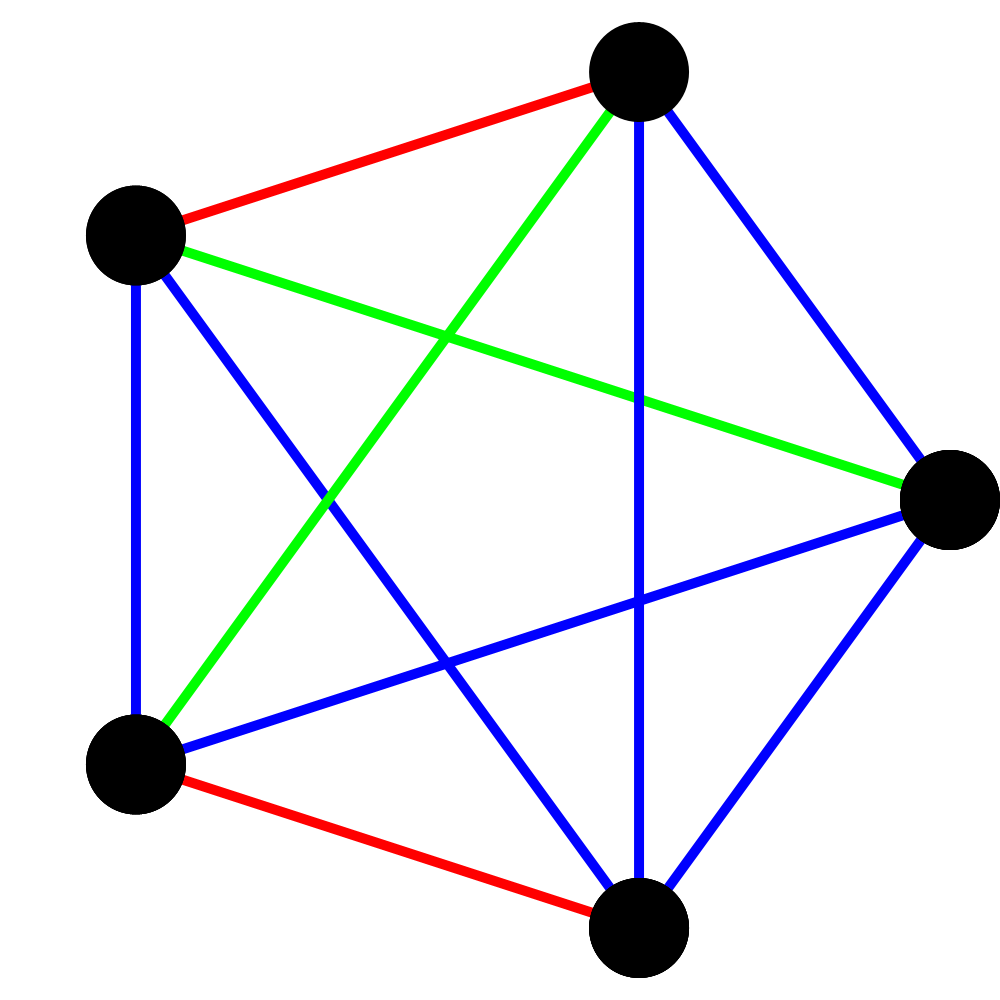} & & & & \\
\hline
\end{tabular}
}
\caption{\textbf{Visualization of Isomorphism Classes.} Visualization of one representative 4-coloring for each isomorphism class of minimal relaxations for autocalibration problems \TT{fguv0}, \TT{fgu00}, \TT{fg000} in $M = 3$ views. For each triplet $(\mathtt{fguvs},M,N)$, we report one representative 4-coloring for each isomorphism class and its associated solution count in $\mathbb{C}$. Solution counts refer to unknown depths and the parameters of $\omega$ in~\eqref{eq:omega}--\eqref{eq:depth-equation-2}.}
\label{SM:tab:isomorphism-viz}
\vspace{-0.5em}
\end{table*}
