# Supplementary material for: Minimal Perspective Autocalibration
Source: arXiv:2405.05605 source file (2024-05-09)
Supplement: Supplementary file 8 [file supp-tab-skew.tex]

% \renewcommand{\arraystretch}{0.975}
\begin{table}[ht]
    \centering
    { \footnotesize
    \begin{tabular}{|c|c|c|c|c|} 
         \hline
         Prior on $K$ & $M$ & $N$ & $L$ & Min \# sol. in $\mathbb{C}$ \\ \hline
         \TT{fguvs^\star} & 2 & - & 1 & $\infty$ \\ 
         \TT{fguvs^\star} & 3 & 5 & 1 & 2313 \\ \hline
         \TT{fg0vs^\star} & 2 & - & 2 & $\infty$ \\ 
         \TT{fg0vs^\star} & 3 & 5 & 2 & 19365 \\ \hline
         \TT{f1uvs^\star} & 2 & - & 2 & $\infty$ \\ 
         \TT{f1uvs^\star} & 3 & 5 & 2 & 29044 \\ \hline
         \TT{f10vs^\star} & 2 & 7 & 3 & 36 \\ 
         \TT{f10vs^\star} & 3 & 5 & 3 & 8272 \\ \hline
         \TT{1guvs^\star} & 2 & - & 2 & $\infty$ \\ 
         \TT{1guvs^\star} & 3 & 5 & 2 & 29046 \\ \hline
         \TT{1g0vs^\star} & 2 & 7 & 3 & 36 \\ 
         \TT{1g0vs^\star} & 3 & 5 & 3 & 8282 \\ \hline
         \TT{11uvs^\star} & 2 & - & 3 & 48 \\ 
         \TT{11uvs^\star} & 3 & 5 & 3 & 8940 \\ \hline
         \TT{110vs^\star} & 2 & 6 & 4 & 60 \\ 
         \TT{110vs^\star} & 3 & 4 & 4 & 1336 \\ \hline
         \TT{ffuvs^\star} & 2 & - & 2 & $\infty$ \\ 
         \TT{ffuvs^\star} & 3 & 5 & 2 & 16188 \\ \hline
         \TT{ff0vs^\star} & 2 & 7 & 3 & 24 \\ 
         \TT{ff0vs^\star} & 3 & 5 & 3 & 4482 \\ \hline
    \end{tabular}
    }
\caption{\textbf{Non-zero Skew Autocalibration Problems.} Specification of 20 notable minimal problems in 2 and 3 views $(M)$ where $s^\star = \frac{s}{g}$ is known and non-zero and $v$ is unknown. For each triplet $(\mathtt{fguvs},M,N)$, we report $L$, number of linear constraints on $K$, and the minimum, taken over all minimal relaxations, solution count in $\mathbb{C}$ for generic input (including ~$s^*.$)
As in~\Cref{tab:Minimal-Autocalibration-Substitution-Tab}, counts refer to unknown depths and the parameters of $\omega$ in~\eqref{eq:omega}--\eqref{eq:depth-equation-2}.}
\label{SM:tab:norm-skew-minimal}
\end{table}
